# Supplementary material for: Probing the link between residual entropy and viscosity of molecular fluids and model potentials
Source: arXiv:1809.05682 ancillary file (2018-09-15)
Supplement: Supplementary file 1 [file SI.pdf]

# Supplementary Information for

## Probing the link between residual entropy and viscosity of molecular fluids and model potentials

**Ian H. Bell**

**Ian H. Bell.**
**E-mail: ian.bell@nist.gov**

### This PDF file includes:

Supplementary text
Figs. S1 to S21
Tables S1 to S16
References for SI reference citations

## Supporting Information Text

## Contents

**1 Units** **2**

**2 Molecular fluids** **2**

2.A Gas Phase . . . 2
2.B Conversion of density-explicit EOS . . . 3
2.C Selected Contours of $s^{\mathrm{r}}$ . . . 5
2.D Coverage . . . 6
2.D.1 Argon . . . 8
2.D.2 Methane . . . 8
2.D.3 $CO_2$ . . . 8
2.D.4 $SF_6$ . . . 9
2.D.5 R-134a . . . 9
2.D.6 R-125 . . . 9
2.D.7 Methanol . . . 10
2.D.8 Water . . . 10
2.E Fluid-Specific Correlations . . . 12

**3 Model Potentials** **14**

3.A Residual Entropy . . . 14
3.B Hard sphere analysis . . . 14
3.C Inverse-power pair potential (IPP) analysis . . . 15
3.C.1 Dilute gas . . . 16
3.C.2 Dense phase . . . 17
3.C.3 Residual Entropy . . . 17
3.D WCA analysis . . . 18
3.D.1 Simulation method . . . 20
3.E Lennard-Jones . . . 21
3.F Overview . . . 23

**4 Residual Entropy Corresponding States** **24**

4.A Alternative Length Scales . . . 24
4.B IPP potential . . . 26
4.C Hard sphere . . . 27

**5 Fitted parameters** **29**

## 1. Units

The parameter $\rho_{\mathrm{N}}$ is the number density of molecules per cubic meter, and is obtained from $\rho_{\mathrm{N}} = \rho N_{\mathrm{A}}$, where the density $\rho$ is in mol m$^{-3}$, $N_{\mathrm{A}}$ is Avogadro's constant (6.022140857(74)$\times$ $10^{23}$ mol$^{-1}$)(1), and $k_{\mathrm{B}}$ is Boltzmann's constant (1.38064852(79)$\times$ $10^{-23}$ J K$^{-1}$) (1). The mass of one molecule $m$ is given by $M/N_{\mathrm{A}}$, where $M$ is the molar mass in kg mol$^{-1}$.

## 2. Molecular fluids

**2.A. Gas Phase.** Figure S1 shows the results in the gaseous region. This zoomed-in view shows more clearly the deviation from the monovariate relationship between reduced viscosity and residual entropy than the zoomed-out version in the main manuscript.

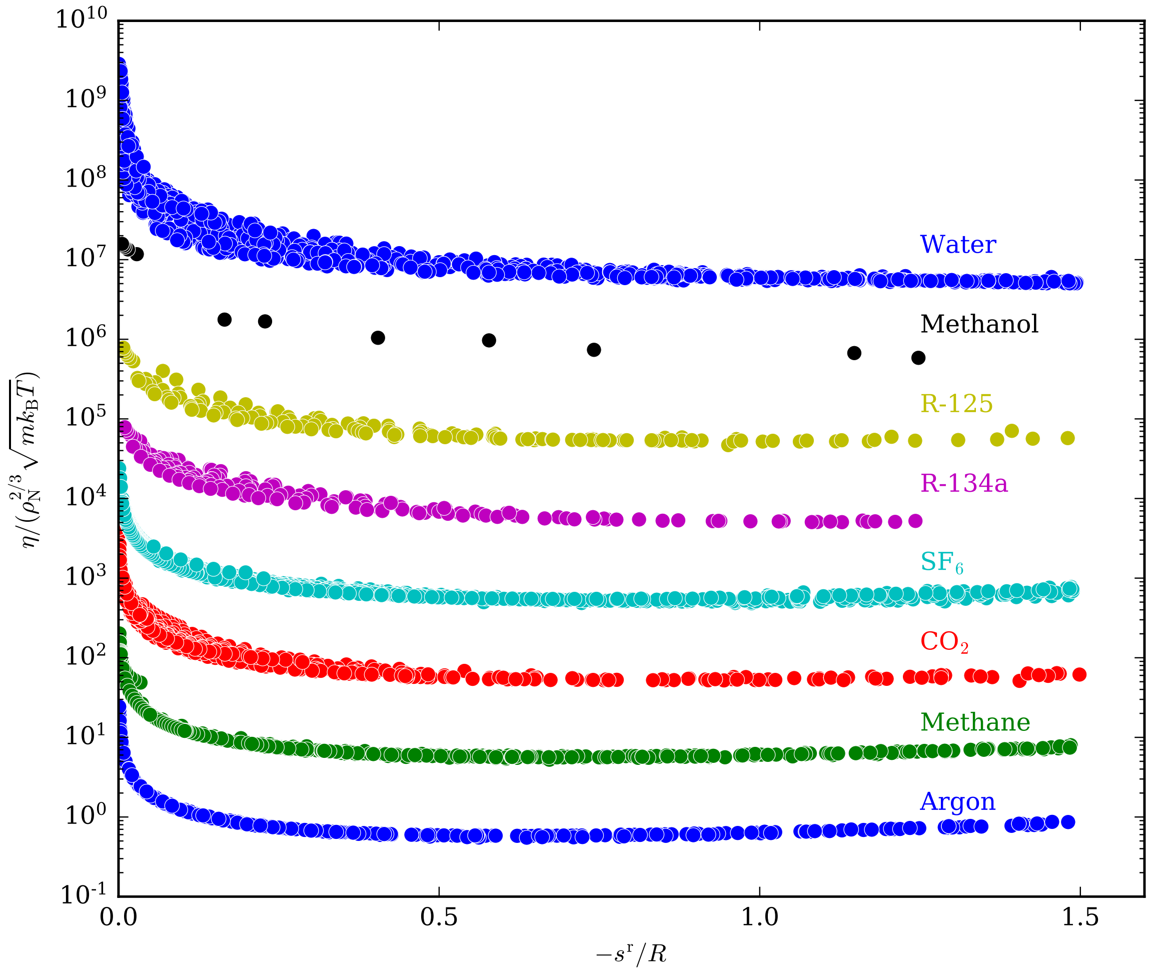


**Fig. S1.** Overview of relationship between reduced viscosity and residual entropy for the molecular fluids in the gaseous region. The data are vertically stacked by multiplying by increasing powers of 10.

**2.B. Conversion of density-explicit EOS.** The reference equation of state for carbon dioxide of Span and Wagner (2) has an upper pressure limit of 800 MPa. Giordano *et al.* (3) have measured the $p$-$v$-$T$ relationship of carbon dioxide and report a density correlation in the form $\rho = f(T, p)$ for the range of 0.1-8 GPa and 300-700 K with an uncertainty of 2 %. The residual entropy is obtained from this formulation as described below.

The link between the entropy $s$ and the $p$-$v$-$T$ relationship is provided by the Maxwell relationship

$$\left(\frac{\partial s}{\partial p}\right)_T = -\left(\frac{\partial v}{\partial T}\right)_p \qquad [1]$$

with $s$ and $v$ as molar quantities. This equation can be integrated to obtain an entropy difference $\Delta s$ between a reference pressure $p_0$ and the pressure of interest $p$ along an isotherm:

$$\Delta s = \int_{p_0}^{p} \left(\frac{\partial s}{\partial p}\right)_T \mathrm{d}p. \qquad [2]$$

The equation of state of Giordano *et al.* does not have its own ideal-gas formulation, so we remedy that problem by evaluating the ideal-gas entropy from the equation of state of Span & Wagner.

When the reference pressure is selected within the range of validity of the equation of state of Span and Wagner, the residual entropy for the high-pressure viscosity data can be obtained from the two formulations in a thermodynamically consistent way as

$$s^r = s_{SW}(T, p_0) + \Delta s(T, \rho) - s_{SW}^{(0)}(T, \rho) \qquad [3]$$

Expressed in consistent base-SI units, the EOS of Giordano (3) (originally with pressure in GPa, temperature in Kelvins, and density in g cm$^{-3}$) reads

$$\ln\left(\frac{\rho M}{1000}\right) = \sum_{i=0}^{2}\sum_{j=0}^{3} a_{ij}T^i \left(\ln\frac{p}{1\times 10^9\ \mathrm{Pa}}\right)^j, \quad [4]$$

where $\rho$ is the density in mol m$^{-3}$, $M$ is the molar mass in kg mol$^{-1}$, $p$ is the pressure in Pa, and $T$ is the temperature in K.

After substitution of the molar volume by $v = 1/\rho$, Eq. (1) becomes

$$\left(\frac{\partial s}{\partial p}\right)_T = \frac{1}{\rho^2}\left(\frac{\partial \rho}{\partial T}\right)_p \quad [5]$$

The derivative of the logarithm of the molar density can then be reformulated as

$$\left(\frac{\partial \ln\left(\frac{\rho M}{1000}\right)}{\partial T}\right)_p = \sum_{i=0}^{2}\sum_{j=0}^{3} a_{ij}iT^{i-1}\left(\ln\frac{p}{1\times 10^9\ \mathrm{Pa}}\right)^j \quad [6]$$

and the derivative of the logarithm of the scaled density with the molar density can be given by

$$\frac{\mathrm{d}\ln\left(\frac{\rho M}{1000}\right)}{\mathrm{d}\rho} = \frac{1}{\frac{\rho M}{1000}}\frac{M}{1000} = \frac{1}{\rho} \quad [7]$$

and thus

$$\left(\frac{\partial \rho}{\partial T}\right)_p = \rho\sum_{i=0}^{2}\sum_{j=0}^{3} a_{ij}iT^{i-1}\left(\ln\frac{p}{1\times 10^9\ \mathrm{Pa}}\right)^j \quad [8]$$

or

$$\Delta s = \int_{p_0}^{p}\left[\frac{1}{\rho}\sum_{i=0}^{2}\sum_{j=0}^{3} a_{ij}iT^{i-1}\left(\ln\frac{p}{1\times 10^9\ \mathrm{Pa}}\right)^j\right]\mathrm{d}p, \quad [9]$$

which was in this work integrated numerically with the `quad` function from the python package `scipy.integrate`.

The effect of the two entropy formulations on the scaling of the data of Abramson (4) is shown in Fig. S2. The use of the equation of state of Giordano results in a nearly monovariate representation of the data of Abramson. The experimental uncertainty is claimed to be approximately 10%. In light of the experimental data for argon, in which a pronounced increase in curvature is noted at large values of $-s^{\mathrm{r}}/R$ in these scaled coordinates, selection of the most appropriate equation of state remains a somewhat open question.

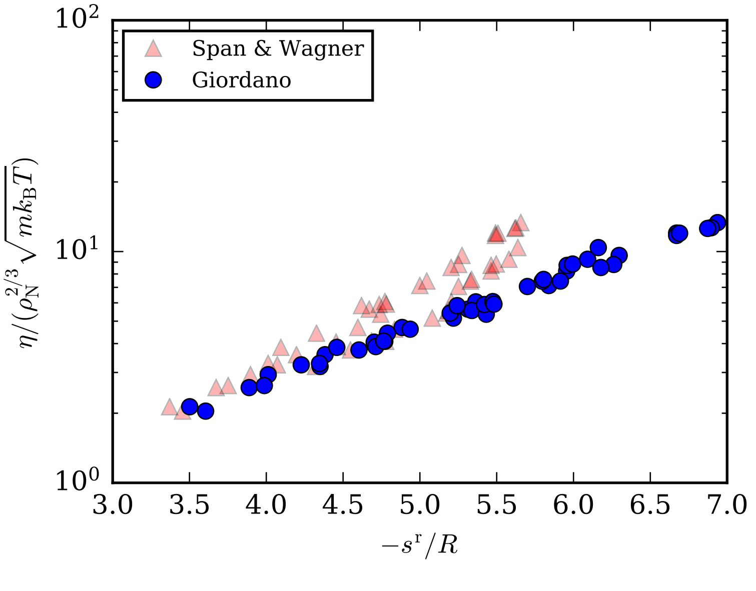


**Fig. S2.** Comparison of entropy scaling approaches for $CO_2$

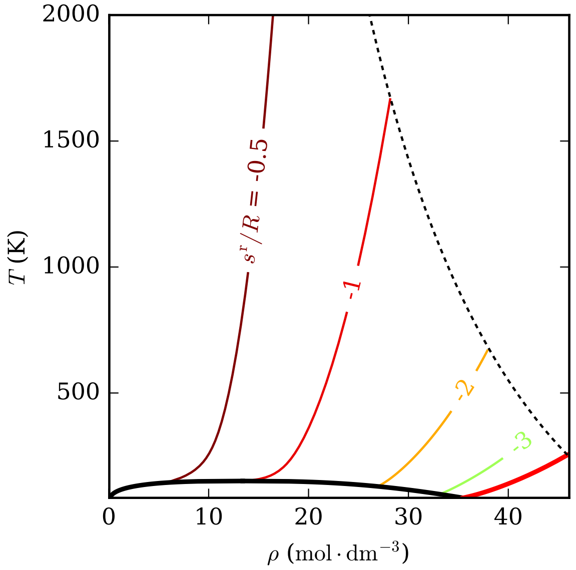


**(a)** Argon (5)

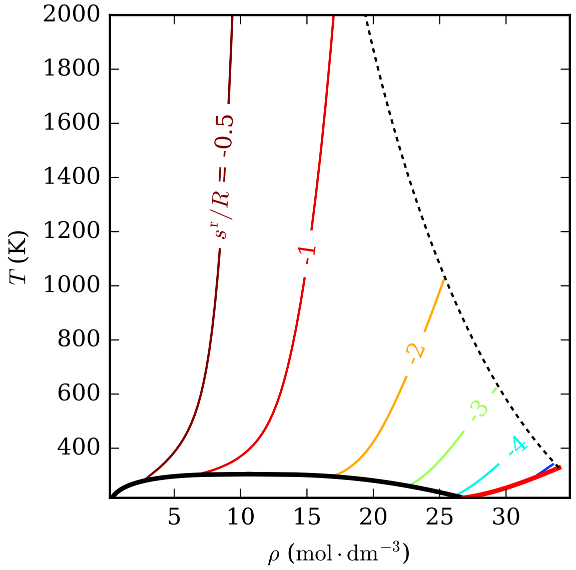


**(b)** $CO_2$ (2)

**Fig. S3.** Contours of the residual entropy $s^r/R$. Contours were generated by the matplotlib plotting library (6), dashed curve is the line of maximum pressure of the equation of state, solid red curve is the melting line, solid black curve is the vapor-liquid co-existence curve (the binodal).

## 2.C. Selected Contours of $s^r$.

**2.D. Coverage.** Figure S4 provides an overview of the data points for each fluid in temperature, density coordinates. Tables S1 to S8 provides tabular information on the data sources that were included in our study. We do not include data sets in the dilute-gas limit, as these data are not relevant for the liquid phase.

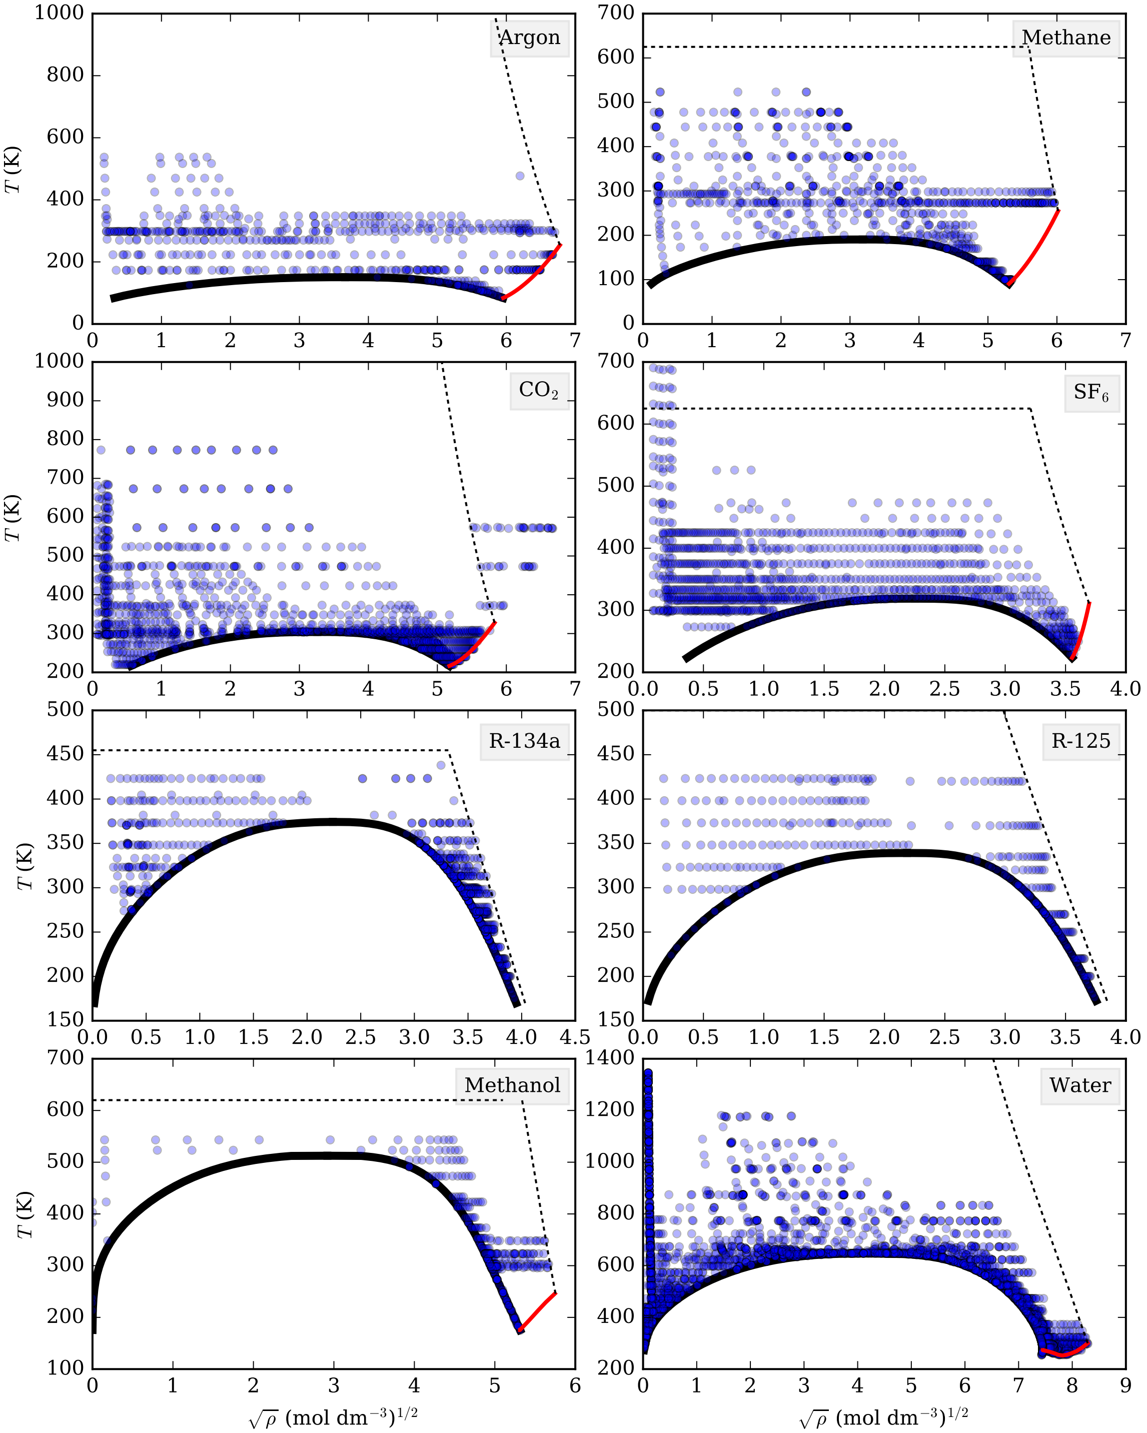


**Fig. S4.** Data coverage of the experimental viscosity measurements for each fluid in this study. Dashed lines indicate the maximum temperature and pressure limits of the equation of state for each fluid. Melting lines, when available, are also included, in red. Each marker corresponds to one data point, and additional data on the considered datasets are included in the supplemental material.

**Table S1. Summary of data sources employed for Argon**

| Author | Year | $N$ | $T$/K | Reference |
|---|---|---|---|---|
| Michels et al. | 1954 | 100 | 273.15 - 348.15 | (7) |
| Kestin, Whitelaw | 1963 | 48 | 295.44 - 537.49 | (8) |
| Gracki et al. | 1969 | 47 | 173.15 - 298.15 | (9) |
| Kestin et al. | 1971 | 40 | 297.33 - 298.46 | (10) |
| Haynes | 1973 | 153 | 107.00 - 298.00 | (11) |
| Haynes | 1973 | 14 | 85.00 - 150.00 | (11) |
| Vermesse, Vidal | 1973 | 25 | 308.15 - 308.15 | (12) |
| Trappeniers et al. | 1980 | 44 | 223.15 - 323.15 | (13) |
| van der Gulik, Trappeniers | 1986 | 25 | 174.45 - 174.45 | (14) |
| Mostert et al. | 1989 | 25 | 174.45 - 174.45 | (15) |
| Abramson | 2011 | 9 | 293.90 - 477.10 | (16) |

#### 2.D.1. Argon.

**Table S2. Summary of data sources employed for Methane**

| Author | Year | $N$ | $T$/K | Reference |
|---|---|---|---|---|
| Ross and Brown | 1957 | 28 | 222.99 - 298.14 | (17) |
| Baron et al. | 1959 | 40 | 324.79 - 408.13 | (18) |
| Carmichael et al. | 1965 | 173 | 277.59 - 477.60 | (19) |
| Haynes | 1973 | 20 | 95.01 - 190.01 | (20) |
| Chuang et al. | 1976 | 36 | 173.16 - 273.15 | (21) |
| Diller | 1980 | 116 | 100.01 - 299.99 | (22) |
| Huang and Swift | 1966 | 59 | 113.16 - 273.15 | (23) |
| van der Gulik et al. | 1988 | 39 | 298.15 - 298.15 | (24) |
| van der Gulik et al. | 1992 | 125 | 273.10 - 273.10 | (25) |
| Evers et al. | 2002 | 61 | 233.15 - 523.15 | (26) |
| Hurly et al. | 2003 | 26 | 293.15 - 293.15 | (27) |
| Abramson | 2011 | 2 | 294.30 - 295.00 | (28) |

#### 2.D.2. Methane.

**Table S3. Summary of data sources employed for $CO_2$**

| Author | Year | $N$ | $T$/K | Reference |
|---|---|---|---|---|
| Golubev, Petrov | 1953 | 144 | 293.14 - 523.17 | (29) |
| Michels et al. | 1957 | 195 | 273.15 - 348.12 | (30) |
| Kestin, Whitelaw | 1963 | 43 | 295.00 - 525.11 | (31) |
| Golubev et al. | 1971 | 72 | 473.11 - 773.07 | (32) |
| Golubev, Shepeleva | 1971 | 107 | 241.76 - 293.84 | (33) |
| Haepp | 1976 | 84 | 298.32 - 474.95 | (34) |
| Vogel, Barkow | 1986 | 40 | 295.08 - 646.87 | (35) |
| Hendl et al. | 1993 | 94 | 297.18 - 685.12 | (36) |
| Docter et al. | 1997 | 8 | 298.15 - 523.15 | (37) |
| van der Gulik | 1997 | 292 | 220.00 - 308.15 | (38) |
| Estrada-Alexanders, Hurly | 2008 | 123 | 220.00 - 370.00 | (39) |
| Abramson | 2009 | 47 | 307.85 - 574.15 | (4) |
| Schäfer et al. | 2015 | 54 | 253.15 - 473.16 | (40) |

#### 2.D.3. $CO_2$.

**Table S4. Summary of data sources employed for $SF_6$**

| Author | Year | $N$ | $T$/K | Reference |
|---|---|---|---|---|
| Kestin et al. | 1971 | 2 | 296.39 - 302.81 | (41) |
| Ueda, Kigoshi | 1974 | 8 | 273.46 - 348.16 | (42) |
| Timrot et al. | 1975 | 62 | 297.40 - 525.90 | (43) |
| Grigorev et al. | 1977 | 133 | 245.15 - 473.15 | (44) |
| Kestin et al. | 1977 | 10 | 296.15 - 474.15 | (45) |
| Ulybin, Makarushkin | 1977 | 63 | 230.00 - 300.00 | (46) |
| Hoogland, Trappeniers | 1982 | 13 | 318.75 - 323.65 | (47) |
| Hoogland et al. | 1985 | 26 | 298.11 - 333.18 | (48) |
| Takahashi et al. | 1987 | 33 | 274.00 - 318.55 | (49) |
| Strehlow, Vogel | 1989 | 77 | 298.51 - 690.72 | (50) |
| Hurly et al. | 2003 | 15 | 298.15 - 298.15 | (51) |
| Wilhelm et al. | 2005 | 677 | 300.00 - 425.00 | (52) |
| Estrada-Alexanders, Hurly | 2008 | 8 | 273.16 - 273.16 | (53) |

#### 2.D.4. $SF_6$.

**Table S5. Summary of data sources employed for R-134a**

| Author | Year | $N$ | $T$/K | Reference |
|---|---|---|---|---|
| Ruvinskii et al. | 1990 | 34 | 257.58 - 404.56 | (54) |
| Kumagai, Takahashi | 1991 | 8 | 273.15 - 343.13 | (55) |
| Okubo et al. | 1992 | 81 | 213.09 - 423.25 | (56) |
| Diller et al. | 1993 | 63 | 200.01 - 299.99 | (57) |
| Diller et al. | 1993 | 30 | 175.01 - 319.99 | (57) |
| Assael et al. | 1994 | 32 | 273.15 - 333.26 | (58) |
| Pasekov, Ustyuzhanin | 1994 | 37 | 275.27 - 370.53 | (59) |
| Assael et al. | 1995 | 7 | 273.15 - 333.15 | (60) |
| MacPherson | 1995 | 27 | 255.75 - 333.20 | (61) |
| Assael, Polimatidou | 1996 | 22 | 273.94 - 333.19 | (62) |
| Oliveira, Fenghour | 1996 | 10 | 245.35 - 343.05 | (63) |
| Shibasaki-Kitagawa et al. | 1998 | 126 | 298.15 - 423.15 | (64) |
| Laesecke et al. | 1999 | 91 | 240.85 - 350.10 | (65) |
| Comuñas et al. | 2003 | 35 | 293.15 - 373.15 | (66) |
| Laesecke, Bair | 2011 | 19 | 293.15 - 438.15 | (67) |
| Meng et al. | 2011 | 43 | 258.15 - 338.13 | (68) |
| Meng et al. | 2013 | 54 | 253.14 - 353.16 | (69) |
| Zhao et al. | 2014 | 7 | 312.86 - 368.26 | (70) |

#### 2.D.5. R-134a.

**Table S6. Summary of data sources employed for R-125**

| Author | Year | $N$ | $T$/K | Reference |
|---|---|---|---|---|
| Diller and Peterson | 1993 | 105 | 200.00 - 420.00 | (71) |
| Diller, Peterson | 1993 | 32 | 176.00 - 330.00 | (71) |
| Ripple and Matar | 1993 | 15 | 250.05 - 301.95 | (72) |
| Assael et al. | 1995 | 5 | 273.15 - 313.15 | (73) |
| Ripple and Defibaugh | 1997 | 7 | 255.95 - 303.07 | (74) |
| Oliveira and Wakeham | 1999 | 13 | 223.99 - 331.99 | (75) |
| Takahashi et al. | 1999 | 131 | 298.15 - 423.15 | (76) |
| Fröba et al. | 1999 | 11 | 233.15 - 333.15 | (77) |

#### 2.D.6. R-125.

**Table S7. Summary of data sources employed for Methanol**

| Author | Year | $N$ | $T$/K | Reference |
|---|---|---|---|---|
| Bridgman | 1926 | 14 | 303.13 - 348.12 | (78) |
| Mitsukuri, Tonomura | 1927 | 13 | 174.89 - 273.15 | (79) |
| Blokker | 1936 | 16 | 298.14 - 491.16 | (80) |
| Amis et al. | 1942 | 5 | 283.18 - 323.13 | (81) |
| Bridgman | 1949 | 1 | 298.14 - 298.14 | (82) |
| Golubev | 1970 | 66 | 423.11 - 543.11 | (83) |
| Hammond et al. | 1958 | 6 | 293.14 - 337.62 | (84) |
| Ling, van Winkle | 1958 | 6 | 303.13 - 423.13 | (85) |
| Bamelis et al. | 1965 | 4 | 298.14 - 328.13 | (86) |
| Isakova, Oshueva | 1966 | 47 | 293.14 - 433.14 | (87) |
| Harlow | 1967 | 27 | 303.13 - 348.12 | (88) |
| Yergovich et al. | 1971 | 11 | 183.16 - 283.15 | (89) |
| Weber | 1975 | 17 | 273.15 - 373.12 | (90) |
| Lee et al. | 1976 | 6 | 288.15 - 323.14 | (91) |
| Schneider | 1978 | 27 | 183.16 - 323.14 | (92) |
| Isdale et al. | 1985 | 44 | 298.13 - 323.14 | (93) |
| Pikkarainen | 1988 | 1 | 303.14 - 303.14 | (94) |
| Matsuo, Makita | 1991 | 24 | 303.15 - 323.15 | (95) |
| Herbst et al. | 1992 | 6 | 296.15 - 296.15 | (96) |
| Aminabhavi et al. | 1993 | 3 | 298.15 - 308.15 | (97) |
| Cook et al. | 1993 | 3 | 295.65 - 295.65 | (98) |
| Assael, Polimatidou | 1994 | 24 | 295.00 - 323.20 | (99) |
| Tu et al. | 2001 | 4 | 293.15 - 313.15 | (100) |

***2.D.7. Methanol.***

**Table S8. Summary of data sources employed for Water**

| First Author | Year | $N$ | $T$/K | Reference |
|---|---|---|---|---|
| Abdulagatov | 2003 | 27 | 297.88 - 574.32 | (101) |
| Abdulagatov | 2004 | 25 | 294.46 - 597.56 | (102) |
| Abdulagatov | 2005 | 28 | 296.70 - 573.70 | (103) |
| Abulagatov | 2005 | 25 | 294.46 - 597.56 | (102) |
| Agaev | 1967 | 598 | 273.37 - 373.12 | (104) |
| Agaev | 1980 | 166 | 263.15 - 473.26 | (105) |
| Assael | 1994 | 19 | 293.11 - 328.08 | (106) |
| Baldauf | 1983 | 3 | 283.15 - 303.14 | (107) |
| Berstad | 1988 | 18 | 292.62 - 298.62 | (108) |
| Coe | 1944 | 3 | 298.14 - 313.13 | (109) |
| Collings | 1983 | 12 | 274.15 - 343.13 | (110) |
| DeFries | 1977 | 46 | 258.15 - 283.15 | (111) |
| Dudziak | 1966 | 91 | 433.14 - 833.15 | (112) |
| Dumas | 1970 | 4 | 289.04 - 294.04 | (113) |
| Eicher | 1971 | 13 | 264.87 - 313.14 | (114) |
| Forst | 2000 | 95 | 260.15 - 313.15 | (115) |
| Goncalves | 1980 | 6 | 293.14 - 333.13 | (116) |
| Hallett | 1963 | 20 | 254.17 - 273.15 | (117) |
| Hardy | 1949 | 10 | 278.15 - 398.13 | (118) |
| Harlow | 1967 | 125 | 275.35 - 373.12 | (119) |
| Harris | 2004 | 109 | 255.65 - 298.15 | (120, 121) |
| Horne | 1966 | 140 | 275.40 - 293.50 | (122) |
| Isdale | 1975 | 22 | 298.14 - 323.14 | (123) |
| James | 1984 | 8 | 273.15 - 333.13 | (124) |
| Kerimov | 1969 | 224 | 373.12 - 548.25 | (125) |
| Kestin | 1960 | 19 | 410.61 - 510.92 | (126) |

Continued on next page...

Table S8 – continued from previous page

| First Author | Year | $N$ | $T$/K | Reference |
|---|---|---|---|---|
| Kestin | 1963 | 39 | 421.09 - 548.44 | (127) |
| Kestin | 1977 | 70 | 283.67 - 311.86 | (128) |
| Kestin | 1978 | 111 | 312.54 - 423.01 | (129) |
| Kestin | 1981 | 78 | 298.70 - 424.06 | (130) |
| Kestin | 1985 | 74 | 297.84 - 491.91 | (131) |
| Kingham | 1974 | 20 | 273.64 - 283.11 | (132) |
| Korosi | 1968 | 9 | 298.14 - 423.13 | (133) |
| Korson | 1969 | 13 | 283.14 - 343.12 | (134) |
| Kozlov | 1985 | 6 | 283.15 - 338.13 | (135) |
| Kubota | 1979 | 32 | 283.15 - 348.13 | (136) |
| Kudish | 1974 | 5 | 288.15 - 308.14 | (137) |
| Latto | 1965 | 555 | 383.43 - 1346.24 | (138) |
| Lee | 1992 | 3 | 303.14 - 323.14 | (139) |
| Lee | 1995 | 3 | 303.15 - 323.15 | (140) |
| Malyarov | 1959 | 1 | 293.14 - 293.14 | (141) |
| Mashovets | 1971 | 11 | 364.83 - 547.61 | (142) |
| Mayinger | 1962 | 84 | 351.92 - 980.05 | (143) |
| Mazurkiew. | 1990 | 1 | 298.14 - 298.14 | (144) |
| Melzer | 1989 | 3 | 283.15 - 303.14 | (145) |
| Moszinsky | 1961 | 66 | 293.49 - 540.18 | (146) |
| Naake | 1984 | 18 | 291.35 - 478.61 | (147) |
| Nagashima | 1969 | 251 | 322.83 - 1178.71 | (148) |
| Nagashima | 1974 | 53 | 523.31 - 874.43 | (149) |
| Olive | 1994 | 1 | 303.15 - 303.15 | (150) |
| Oltermann | 1977 | 96 | 613.92 - 655.98 | (151) |
| Penkina | 1971 | 7 | 373.12 - 523.11 | (152) |
| Rankumar | 1989 | 5 | 303.14 - 343.13 | (153) |
| Ravikovich | 1958 | 7 | 298.83 - 355.92 | (154) |
| Rivkin | 1966 | 41 | 323.13 - 573.18 | (155) |
| Rivkin | 1968 | 127 | 548.18 - 723.16 | (156) |
| Rivkin | 1970 | 162 | 496.66 - 668.18 | (157) |
| Rivkin | 1972 | 157 | 496.61 - 668.10 | (158) |
| Rivkin | 1973 | 59 | 648.61 - 773.07 | (159) |
| Rivkin | 1975 | 197 | 496.61 - 668.10 | (160) |
| Roscoe | 1958 | 1 | 293.14 - 293.14 | (161) |
| Rosenberg. | 1992 | 1 | 297.14 - 297.14 | (162) |
| Sato | 1968 | 17 | 429.93 - 473.22 | (163) |
| Sato | 1970 | 79 | 433.14 - 778.15 | (164) |
| Shifrin | 1959 | 114 | 422.13 - 1139.61 | (165) |
| Stanley | 1969 | 93 | 275.38 - 293.15 | (166) |
| Swindells | 1952 | 1 | 293.14 - 293.14 | (167) |
| Tanaka | 1965 | 152 | 285.24 - 1181.06 | (168) |
| Tanaka | 1987 | 47 | 283.15 - 348.13 | (169) |
| Teske | 2005 | 109 | 297.39 - 440.41 | (170) |
| Timrot | 1973 | 46 | 325.74 - 772.07 | (171) |
| Weber | 1955 | 9 | 273.15 - 313.13 | (172) |
| White | 1914 | 11 | 263.86 - 293.14 | (173) |
| Whitelaw | 1960 | 55 | 293.54 - 927.42 | (174) |
| Wode | 1994 | 5 | 293.15 - 313.15 | (175) |
| Yasumoto | 1970 | 15 | 279.88 - 302.13 | (176) |

***2.D.8. Water.***

**2.E. Fluid-Specific Correlations.** As described in the main manuscript, polynomial curves were fit of the form

$$\eta^{\#} = \ln\left[\frac{\eta}{\rho_{\rm N}^{2/3}\sqrt{mk_{\rm B}T}}\cdot\left(-\frac{s^{\rm r}}{R}\right)^{2/3}\right] = \sum_i c_i\left(-\frac{s^{\rm r}}{R}\right)^i. \quad [10]$$

The coefficients of the correlations are given in Table S9 and a graphical representation of each correlation is shown in Fig. S5.

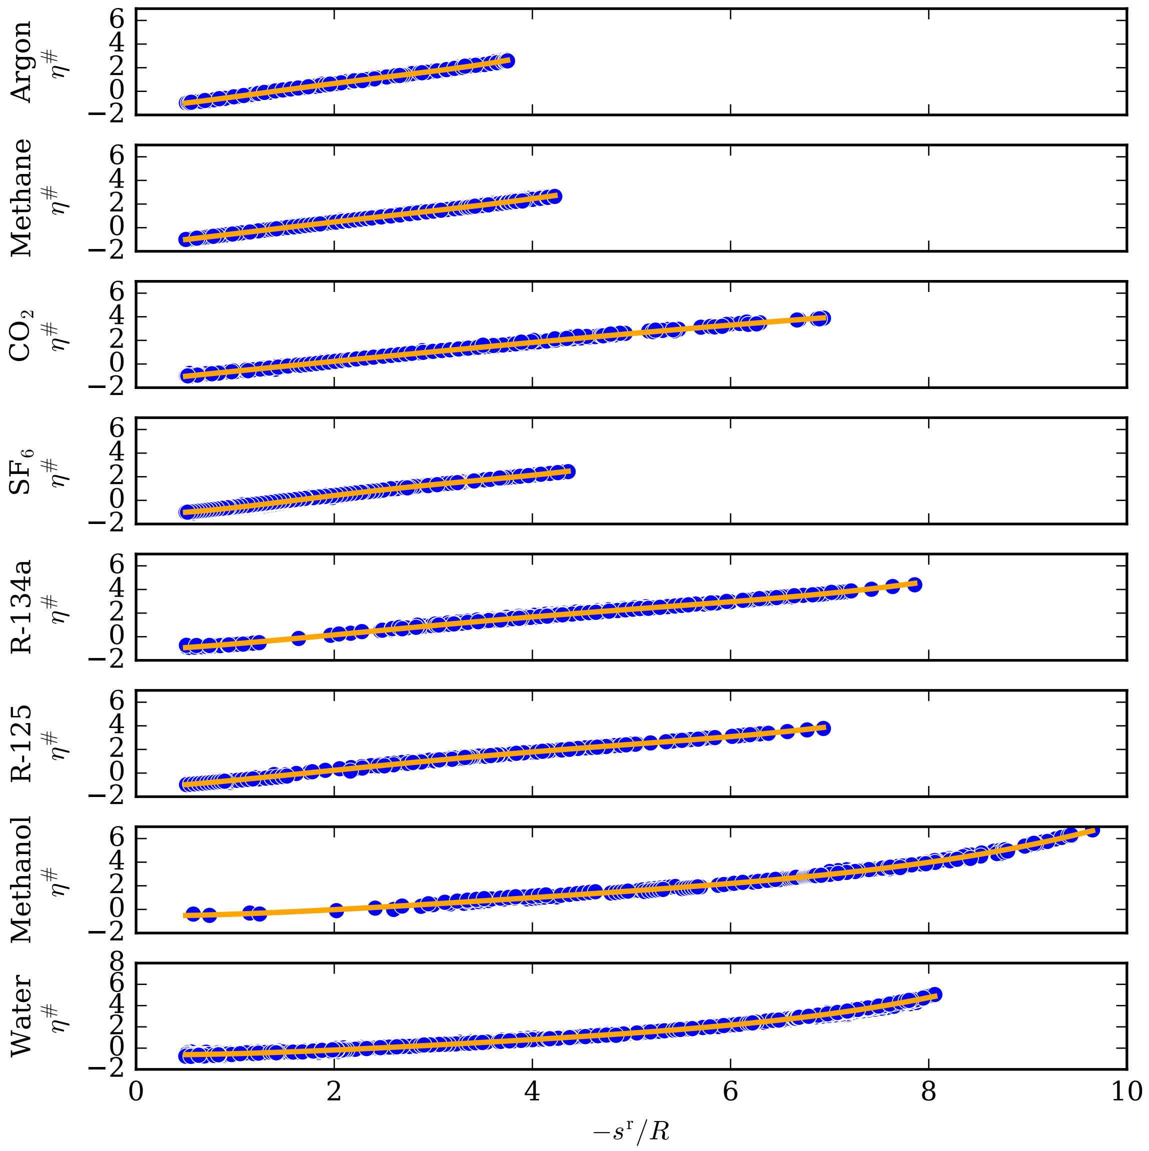


**Fig. S5.** Correlations for each fluid of the form of Eq. (10).

**Table S9. Coefficients for each correlation of the form of Eq. (10) and displayed in Fig. S5. The AAD is for $-s^{\rm r}/R > 0.5$, and given by $AAD = \mathrm{mean}(\mathrm{abs}(\vec{\eta}_{\rm fit}/\vec{\eta}_{\rm exp} - 1)) \times 100$**

| Fluid | $c_0$ | $c_1$ | $c_2$ | $c_3$ | $c_4$ | AAD (%) |
|---|---|---|---|---|---|---|
| Argon | -1.404672164 | 0.6259224251 | 0.4946245134 | -0.196563441 | 0.0257934875 | 2.13 |
| Methane | -1.472307657 | 0.8937830881 | 0.118654351 | -0.05250941825 | 0.007078948658 | 2.31 |
| $CO_2$ | -1.477170836 | 0.8933282033 | -0.02605311557 | 0.003529087823 | -0.000316904443 | 2.63 |
| $SF_6$ | -1.184642564 | 0.04962200976 | 0.7258600137 | -0.2188521818 | 0.02151784914 | 3.34 |
| R-134a | -1.163903171 | 0.3990382292 | 0.2072836786 | -0.04405771211 | 0.002918568642 | 3.52 |
| R-125 | -1.291465461 | 0.5420590701 | 0.193961336 | -0.04843108388 | 0.003552677597 | 3.17 |
| Methanol | -0.5691844549 | 0.0265333847 | 0.1713888914 | -0.02714071018 | 0.001776012196 | 4.30 |
| Water | -0.6335660942 | -0.05294371385 | 0.1979960332 | -0.03397428597 | 0.002572761038 | 3.32 |

## 3. Model Potentials

**3.A. Residual Entropy.** In some cases the residual entropy can be obtained in a closed-form solution from the equation of state (for instance from Carnahan and Starling (177) for the hard sphere). In other cases, closed-form integrable virial expansions for the compressibility factor $Z$ are used, and in still other cases, virial expansions for $Z$ are used that are not integrable analytically (the asymptotically consistent approximation for the IPP for instance (178)). In general, we can obtain the residual entropy from

$$\frac{s^{\rm r}}{R} = -\left(\frac{\partial a^{\rm r}}{\partial T}\right)_\rho = -T\left(\frac{\partial \alpha^{\rm r}}{\partial T}\right)_\rho - \alpha^{\rm r} \qquad [11]$$

where the reduced residual Helmholtz energy is obtained by integration of

$$\alpha^{\rm r} = \int_0^\xi \frac{Z(\xi)-1}{\xi}{\rm d}\xi \qquad [12]$$

where $\xi$ is the independent variable of the potential (the packing fraction for the hard sphere, the scaling parameter $\gamma$ for the IPP, $\zeta_{\rm e}$ for the WCA potential). In the case of the Lennard-Jones 12-6 potential, a multiparameter equation of state is available.

Therefore $s^{\rm r}/R$ is given by

$$\frac{s^{\rm r}}{R} = -T\left(\frac{Z(\xi)-1}{\xi}\right)\left(\frac{\partial \xi}{\partial T}\right)_\rho - \alpha^{\rm r}, \qquad [13]$$

because

$$\left(\frac{\partial \alpha^{\rm r}}{\partial \xi}\right)_\rho = \frac{Z(\xi)-1}{\xi} \qquad [14]$$

**3.B. Hard sphere analysis.** Carnahan and Starling(177) proposed a formulation for the compressibility factor $Z$ for a hard sphere fluid given by

$$Z = \frac{1+\zeta+\zeta^2-\zeta^3}{(1-\zeta)^3}, \qquad [15]$$

in terms of the packing fraction $\zeta$

$$\zeta = \frac{\pi N_{\rm A}\rho\sigma^3}{6}, \qquad [16]$$

that was more accurate than all predecessors. Here, $\rho$ is the molar density in mol/m$^3$, $N_{\rm A}$ is Avogadro's number, and $\sigma$ is the hard sphere diameter in m.

Equation (15) can be integrated to obtain the non-dimensionalized residual Helmholtz energy $\alpha^{\rm r} = a^{\rm r}/(RT)$

$$\alpha^{\rm r} = \int_0^\zeta \frac{Z-1}{\zeta}{\rm d}\zeta \qquad [17]$$

which yields

$$\alpha^{\rm r} = \frac{\zeta(4-3\zeta)}{(1-\zeta)^2} \qquad [18]$$

The residual entropy is given by

$$\frac{s^{\rm r}}{R} = -T\left(\frac{\partial \alpha^{\rm r}}{\partial T}\right)_\rho - \alpha^{\rm r} \qquad [19]$$

but $\alpha^{\rm r}$ has no temperature dependence, thus the residual entropy is simply equal to

$$\frac{s^{\rm r}}{R} = -\alpha^{\rm r} = -\frac{\zeta(4-3\zeta)}{(1-\zeta)^2}. \qquad [20]$$

According to Enskog theory (see for example Sigurgeirsson and Heyes (179, Eq. 17)), the viscosity divided by the dilute-gas viscosity $\eta_{\rho\to 0}$ is equal to

$$\frac{\eta_{\rm E}}{\eta_{\rho\to 0}} = 1.016/g(\sigma) + 0.8(b/v) + 0.7737g(\sigma)(b/v)^2, \qquad [21]$$

where the ratio of the molar volume $v = 1/\rho$ to the close packed volume $b = 2\pi N_{\rm A}\sigma^3/3$ is equal to (180)

$$\frac{v}{b} = \frac{\dfrac{\pi N_{\rm A}\sigma^3}{6\zeta}}{\dfrac{2\pi N_{\rm A}\sigma^3}{3}} = \frac{1}{4\zeta} \qquad [22]$$

and the radial distribution function at contact (180) can be obtained from

$$g(\sigma) = (Z-1)\cdot(v/b). \qquad [23]$$

Thus the viscosity ratio $\eta_{\rm E}/\eta_{\rho\to 0}$ as a function of $s^{\rm r}/R$ becomes a monovariate function of the packing fraction $\zeta$; neither $\eta_{\rm E}/\eta_{\rho\to 0}$ nor $s^{\rm r}/R$ is an explicit function of $\sigma$ or $T$.

The Enskog hard-sphere viscosity is then corrected with an empirical fit of molecular dynamics simulations as a function of the ratio of the packing fraction to the close-packed packing fraction $\zeta_{\rm cp} = \pi\sqrt{2}/6 \approxeq 0.7405$ (179, p. 470). The hard-sphere fluid freezes at approximately $\zeta = 0.494$ (179) In the nomenclature of hard-sphere literature, $V_0/V = \zeta/\zeta_{\rm cp}$. Therefore the correction term of Sigurgeirsson and Heyes (179, Eq. 39) is given by

$$\frac{\eta}{\eta_{\rm E}} = \begin{cases} 1.02, & \zeta/\zeta_{\rm cp} < 0.42 \\ 1.02 + 18(\zeta/\zeta_{\rm cp} - 0.35)^3, & 0.42 < \zeta/\zeta_{\rm cp} < 0.575 \\ 1.02 + 18(\zeta/\zeta_{\rm cp} - 0.35)^3 + 575(\zeta/\zeta_{\rm cp} - 0.575)^3, & \zeta/\zeta_{\rm cp} > 0.575 \end{cases} \quad [24]$$

The reduced hard-sphere viscosity is given by

$$\frac{\eta}{\rho_{\rm N}^{2/3}\sqrt{mk_{\rm B}T}} = \frac{\eta}{\eta_{\rm E}}\frac{\eta_{\rm E}}{\eta_{\rho\to 0}}\frac{\eta_{\rho\to 0}}{\rho_{\rm N}^{2/3}\sqrt{mk_{\rm B}T}} \quad [25]$$

where with the dilute gas viscosity of

$$\eta_{\rho\to 0} = \frac{5}{16\sigma^2}\sqrt{\frac{mk_{\rm B}T}{\pi}} \quad [26]$$

the reduced dilute-gas viscosity is given by

$$\frac{\eta_{\rho\to 0}}{\rho_{\rm N}^{2/3}\sqrt{mk_{\rm B}T}} = \frac{\frac{5}{16\sigma^2}\sqrt{\frac{mk_{\rm B}T}{\pi}}}{\rho_{\rm N}^{2/3}\sqrt{mk_{\rm B}T}} = \frac{\frac{5}{16\sqrt{\pi}\sigma^2}}{\left(\frac{6\zeta}{\sigma^3\pi}\right)^{2/3}} = \frac{5\pi^{1/6}}{16(6\zeta)^{2/3}}. \quad [27]$$

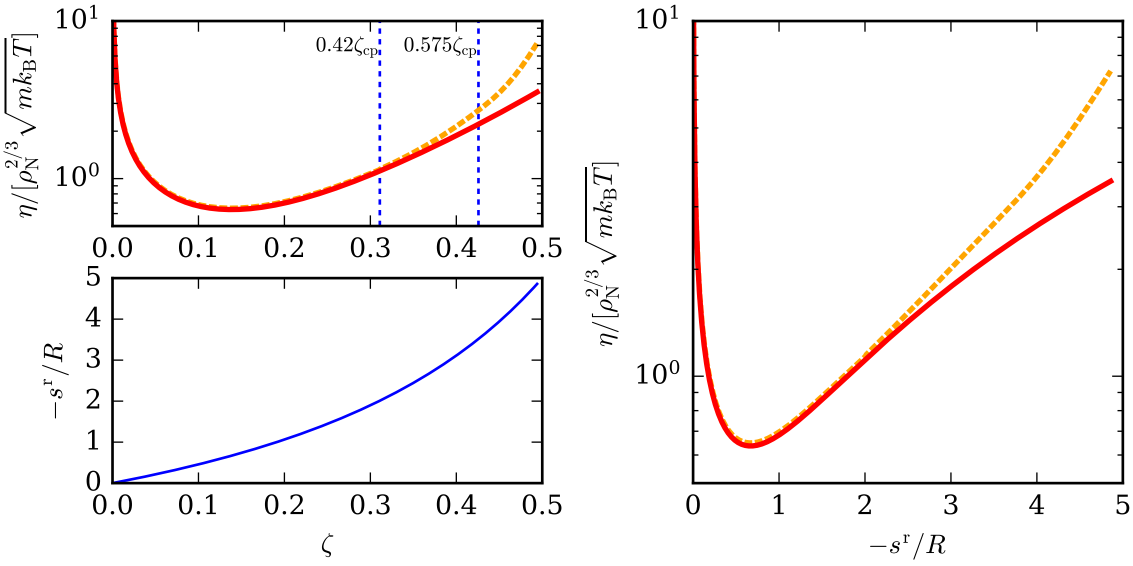


**Fig. S6.** Hard sphere potential: reduced viscosity and residual entropy each plotted against packing fraction $\zeta$ as well as reduced viscosity plotted as a function of residual entropy. Red solid curves: Enskog theory, orange dashed curves: Enskog theory plus empirical correction of Sigurgeirsson and Heyes (179)

**3.C. Inverse-power pair potential (IPP) analysis.** The independent variable $\gamma$ for IPP scaling is given by

$$\gamma = \rho_{\rm N}\sigma^3(T^*)^{-3/n} = \rho^*(T^*)^{-3/n} \quad [28]$$

with $T^* = T/(\varepsilon/k_{\rm B})$, and the number density can be obtained by rearranging the expression for $\gamma$ to obtain

$$\rho_{\rm N} = \frac{\gamma}{\sigma^3(T^*)^{-3/n}}. \quad [29]$$

***3.C.1. Dilute gas.*** For the IPP potential given by $U = \frac{\kappa}{(\nu-1)r^{\nu-1}}$, where $U$ is the potential, $r$ is the separation in meters, and $\kappa$ and $\nu$ are the parameters of the potential. Chapman & Cowling (181, p. 172) give the equation for viscosity in the limit of zero density

$$\eta_{\rho\to 0,\mathrm{IPP}} = \left[ \frac{5\sqrt{mk_\mathrm{B}T}\left(\frac{2k_\mathrm{B}T}{\kappa}\right)^{2/(\nu-1)}}{8\sqrt{\pi}A_2(\nu)\Gamma\left(4-\frac{2}{\nu-1}\right)} \right]. \tag{30}$$

It is nowadays more common to express the IPP potential as $U = \varepsilon\cdot(\sigma/r)^n$, for which the variable transformations are:

$$\nu - 1 = n \tag{31}$$

$$\kappa = n\varepsilon\sigma^n \tag{32}$$

Substitution into Eq. (30) yields

$$\eta_{\rho\to 0,\mathrm{IPP}} = \frac{\sqrt{m\varepsilon}}{\sigma^2}F(n)(T^*)^{n'}, \tag{33}$$

with

$$n' = \frac{2}{n} + \frac{1}{2}, \tag{34}$$

or

$$\frac{\eta^*_{\rho\to 0,\mathrm{IPP}}}{(T^*)^{n'}} = \frac{\eta_{\rho\to 0,\mathrm{IPP}}\sigma^2}{(T^*)^{n'}\sqrt{m\varepsilon}} = F(n) \tag{35}$$

with the function $F(n)$ that is uniquely a function of $n$ given by

$$F(n) = \frac{5\left(\frac{2}{n}\right)^{2/n}}{8\sqrt{\pi}A_2(\nu=n+1)\Gamma\left(4-\frac{2}{n}\right)}. \tag{36}$$

The term $A_2(\nu)$ can be obtained from the general form (181, Eq. 10.31-6)

$$A_l(\nu) = \int_0^\infty (1-\cos^l(\chi))v_0\mathrm{d}v_0 \tag{37}$$

in which the term $\chi$ in the integral is obtained from (181, Eq. 10.31-3)

$$\chi = \pi - 2\int_0^{v_{00}} \left[1 - v^2 - \frac{2}{\nu-1}\left(\frac{v}{v_0}\right)^{\nu-1}\right]^{-1/2} \mathrm{d}v \tag{38}$$

and the limit of the integral $v_{00}$ is the positive root of

$$v_{00} = -\frac{2}{(\nu-1)v_0^{\nu-1}}v^{\nu-1} - v^2 + 1 \tag{39}$$

which must be solved numerically. The code to evaluate $A_l$ with numerical integration is given below in the Python language (compatible with Python versions 2.7 and 3.x)

```
import scipy.integrate
import numpy as np
def A_l(nu,l=2):
    def integrand(v0):
        def get_v00(v0):
            c = np.zeros((nu,))
            c[-1] = 1
            c[-3] = -1
            c[0] = -2/(nu-1)/v0**(nu-1)
            roots = np.roots(c)
            root = roots[np.isreal(roots) & (roots>0)]
            assert(len(root)==1)
            return np.real(root[0])
        def chi(v0):
            def inner(v):
                return (1-v**2-2/(nu-1)*(v/v0)**(nu-1))**-0.5
            v00 = get_v00(v0)
            val, err = scipy.integrate.quad(inner, 0, v00)
            return np.pi-2*val
        return (1-np.cos(chi(v0))**l)*v0
    val, err = scipy.integrate.quad(integrand, 0, np.inf)
    return val
for nu in [5,7,9,11,13,15,21,25]:
    print(nu, nu-1, A_l(nu,l=2))
```

**3.C.2. Dense phase.** The simulations for the IPP potential was carried by Fomin et al.(182) at specified pairs of $\rho^* = \rho_{\rm N}\sigma^3$ and $T^* = Tk_{\rm B}/\varepsilon$. Fomin et al.(182), developed a polynomial fit of $\eta^*/(T^*)^{n'}$, with $n = 12$, and $n' = 2/3$, as a function of $\gamma$. While Fomin use the incorrect dilute-gas limit in their fit (the value of $\eta^*/(T^*)^{n'}$ should be equal to $F(n)$ at $\gamma = 0$), the coefficients in Table S10 yield the correct dilute-gas limit. The form of the correlation is given by

$$\ln\left(\frac{\eta^*}{(T^*)^{2/3}}\right) = \sum_i c_i\gamma^i \qquad [40]$$

in which the $c_0$ term is specified to yield the value of $F(n = 12)$ at $\gamma = 0$, and the remaining parameters are fit to the simulation results of Fomin et al.(182).

**Table S10. Table of coefficients for the correlation for viscosity for the IPP ($n = 12$) potential from Eq. (40)**

| i | $c_i$ |
|---|---|
| 0 | -1.765439248 |
| 1 | -0.5350660584 |
| 2 | 6.481818594 |
| 3 | -5.161736066 |
| 4 | 1.946447525 |

The reducing viscosity is given by

$$\rho_{\rm N}^{2/3}\sqrt{mk_{\rm B}T} = \left(\frac{\gamma}{\sigma^3(T^*)^{-3/n}}\right)^{2/3}\sqrt{mk_{\rm B}T} = \gamma^{2/3}(T^*)^{n'}\frac{\sqrt{m\epsilon}}{\sigma^2} \qquad [41]$$

and the ratio of viscosity $\eta$ to $\rho_{\rm N}^{2/3}\sqrt{mk_{\rm B}T}$ (and dividing numerator and denominator by $(T^*)^{n'}$) is then equal to

$$\frac{\eta}{\rho_{\rm N}^{2/3}\sqrt{mk_{\rm B}T}} = \frac{\dfrac{\eta^*\sqrt{m\epsilon}}{\sigma^2(T^*)^{n'}}}{\dfrac{\rho_{\rm N}^{2/3}\sqrt{mk_{\rm B}T}}{(T^*)^{n'}}} = \frac{\eta^*/(T^*)^{n'}}{\gamma^{2/3}} \qquad [42]$$

Therefore, the reduced viscosity is obtained from the correlation for $\eta^*/(T^*)^{n'}$ and dividing by $\gamma^{2/3}$; the reduced viscosity is a function of only the scaling parameter $\gamma$.

**3.C.3. Residual Entropy.** The residual entropy $s^{\rm r}/R$ is obtained from the generalized asymptotically consistent approximation (ACA) for IPP given in Barlow et al. (178). The residual entropy is obtained by evaluating Eq. (13) with the ACA. The ACA form yields a generalized form of the compressibility factor $Z$ as a function of $\gamma$ for a given value of $n$ that must be integrated numerically. For selected values of $n$, including the most popular value of 12, convergent virial expansions of $Z$ have been constructed (178, 183) that have closed-form integrals.

For $-s^{\rm r}/R$, we first begin with the virial expansion for the n=12 IPP potential as calculated by Tan et al. (183),

$$Z = 1 + \sum_{m=2}^{M} B_m\rho_{\rm N}^{m-1} \qquad [43]$$

where the temperature dependence of the virial coefficients is given by(178)

$$B_m = \bar{B}_m[\sigma^3(T^*)^{-3/n}]^{m-1}, \qquad [44]$$

where $\bar{B}_m$ is the reduced virial coefficient, which is solely a function of the softness of the potential $n$. With reference to Eq. (28), the compressibility factor is then given by

$$Z = 1 + \sum_{m=2}^{M} \bar{B}_m(\gamma)^{m-1} \qquad [45]$$

This gives, upon closed-form integration of

$$\alpha^{\rm r} = \int_0^\gamma \frac{Z-1}{\gamma}{\rm d}\gamma \qquad [46]$$

the solution

$$\alpha^{\rm r} = \sum_{m=2}^{M}\frac{\bar{B}_m}{m-1}\gamma^{m-1} \qquad [47]$$

The residual entropy is obtained from

$$\frac{s^{\rm r}}{R} = -\left(\frac{\partial a^{\rm r}}{\partial T}\right)_\rho = -T^*\left(\frac{\partial \alpha^{\rm r}}{\partial T^*}\right)_{\rho^*} - \alpha^{\rm r}. \quad [48]$$

which can be expresed as

$$\frac{s^{\rm r}}{R} = -T^*\left(\frac{{\rm d}\alpha^{\rm r}}{{\rm d}\gamma}\right)\left(\frac{\partial \gamma}{\partial T^*}\right)_{\rho^*} - \alpha^{\rm r}. \quad [49]$$

The derivative of the scaling parameter $\gamma$ is given by

$$\left(\frac{\partial \gamma}{\partial T^*}\right)_{\rho^*} = \frac{-3}{n}\rho^*(T^*)^{-3/n-1} \quad [50]$$

and thus (see Eq. (28))

$$T^*\left(\frac{\partial \gamma}{\partial T^*}\right)_{\rho^*} = \frac{-3\gamma}{n}, \quad [51]$$

and the residual entropy is finally given by

$$\frac{s^{\rm r}}{R} = \frac{3}{n}(Z-1) - \alpha^{\rm r}, \quad [52]$$

in which all the temperature terms cancel; thus the residual entropy is also not a function of temperature except implicitly via $\gamma$

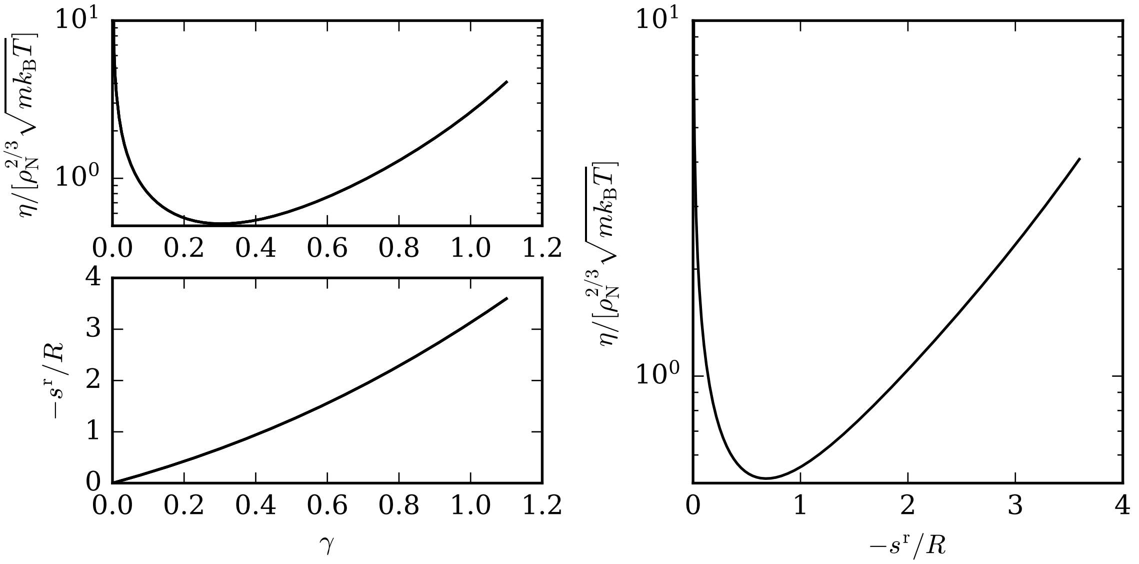


**Fig. S7.** IPP potential with $n = 12$: reduced viscosity and residual entropy, each plotted against scaling variable $\gamma$ as well as reduced viscosity plotted as a function of residual entropy.

**3.D. WCA analysis.** For the repulsive WCA potential, the recommended EOS is that of Heyes and Okumura (184). A WCA-effective packing fraction $\zeta_{\rm e}(T^*, \rho^*)$ is defined by

$$\zeta_{\rm e} = \pi\rho_{\rm N}\sigma_{\rm e}^3/6 = \frac{\pi}{6}\rho^*\left(\frac{\sigma_{\rm e}}{\sigma}\right)^3 \quad [53]$$

with

$$\frac{\sigma_{\rm e}}{\sigma} = \left(\frac{2}{1+\sqrt{T^*}}\right)^{1/6} \quad [54]$$

Another option for the effective length scale is provided in (185), as described in (186).

An empirical form for the compressibility factor was proposed by Heyes and Okumara (184) and is given by

$$Z = \frac{1+\zeta_{\rm e}+a\zeta_{\rm e}^2-b\zeta_{\rm e}^3}{(1-\zeta_{\rm e})^3} \quad [55]$$

with $a = 3.597$ and $b = 5.836$. Following the approach for the hard sphere, we obtain the residual Helmholtz energy by integration of

$$\alpha^{\rm r} = \int_0^{\zeta_{\rm e}} \frac{Z-1}{\zeta_{\rm e}}{\rm d}\zeta_{\rm e}. \quad [56]$$

The residual entropy is obtained from

$$\frac{s^{\rm r}}{R} = -\left(\frac{\partial a^{\rm r}}{\partial T}\right)_{\rho} = -T^{*}\left(\frac{\partial \alpha^{\rm r}}{\partial T^{*}}\right)_{\rho^{*}} - \alpha^{\rm r}. \qquad [57]$$

Unlike the athermal hard-sphere potential, the residual Helmholtz energy for WCA is temperature-dependent due to the temperature dependence of $\sigma_{\rm e}/\sigma$. Expanding the derivatives yields

$$\frac{s^{\rm r}}{R} = -T^{*}\left(\frac{\partial \alpha^{\rm r}}{\partial \zeta_{\rm e}}\right)_{\rho^{*}}\left(\frac{\partial \zeta_{\rm e}}{\partial(\sigma_{\rm e}/\sigma)}\right)_{\rho^{*}}\left(\frac{{\rm d}(\sigma_{\rm e}/\sigma)}{{\rm d}T^{*}}\right) - \alpha^{\rm r}. \qquad [58]$$

In order to simplify the form for the residual entropy, we note that

$$T^{*}\left(\frac{{\rm d}(\frac{\sigma_{\rm e}}{\sigma})}{{\rm d}T^{*}}\right) = \frac{-1}{12}\frac{\sqrt{T^{*}}\frac{\sigma_{\rm e}}{\sigma}}{(1+\sqrt{T^{*}})} \qquad [59]$$

and

$$\left(\frac{\partial \zeta_{\rm e}}{\partial(\sigma_{\rm e}/\sigma)}\right)_{\rho^{*}} = \frac{\pi}{2}\rho^{*}\left(\frac{\sigma_{\rm e}}{\sigma}\right)^{2} \qquad [60]$$

so that we can obtain

$$T^{*}\left(\frac{\partial \zeta_{\rm e}}{\partial(\sigma_{\rm e}/\sigma)}\right)_{\rho^{*}}\left(\frac{\partial(\sigma_{\rm e}/\sigma)}{\partial T^{*}}\right) = \frac{-\pi}{24}\frac{\sqrt{T^{*}}}{(1+\sqrt{T^{*}})}\rho^{*}\left(\frac{\sigma_{\rm e}}{\sigma}\right)^{3} = \frac{-1}{4}\frac{\sqrt{T^{*}}}{(1+\sqrt{T^{*}})}\zeta_{\rm e} \qquad [61]$$

and finally

$$\frac{s^{\rm r}}{R} = \frac{1}{4}\frac{\sqrt{T^{*}}}{(1+\sqrt{T^{*}})}(Z-1) - \alpha^{\rm r}. \qquad [62]$$

Thus, unlike the IPP potential shown above, the temperature dependence of the reduced residual entropy is not entirely captured by the scaling parameter $\zeta_{\rm e}$ and we should not expect all isotherms for the residual entropy to collapse when plotted as a function of $\zeta_{\rm e}$, and indeed they do not. Figure S8 shows the reduced viscosity and residual entropy for the repulsive WCA potential.

As described in the main manuscript, a correlation of the simulation results for the WCA potential was constructed in the form

$$\ln\left(\frac{\eta^{*}}{(\rho^{*})^{2/3}\sqrt{T^{*}}} \times \left(\frac{-s^{\rm r}}{R}\right)^{2/3}\right) = \sum_{i} c_i \left(-\frac{s^{\rm r}}{R}\right)^{i}, \qquad [63]$$

with the coefficients $c_i$ given in Table S11. The multiplication in the left-hand-side of Eq. (63) by $(-s^{\rm r}/R)^{2/3}$ is intended to remove the divergence in the dilute-gas limit where $\rho^{*} = 0$.

**Table S11. Table of coefficients for the correlation for viscosity for the WCA potential from Eq. (63)**

| $i$ | $c_i$ |
|---|---|
| 0 | -1.486168 |
| 1 | 0.923826 |
| 2 | 0.087115 |
| 3 | -0.016928 |

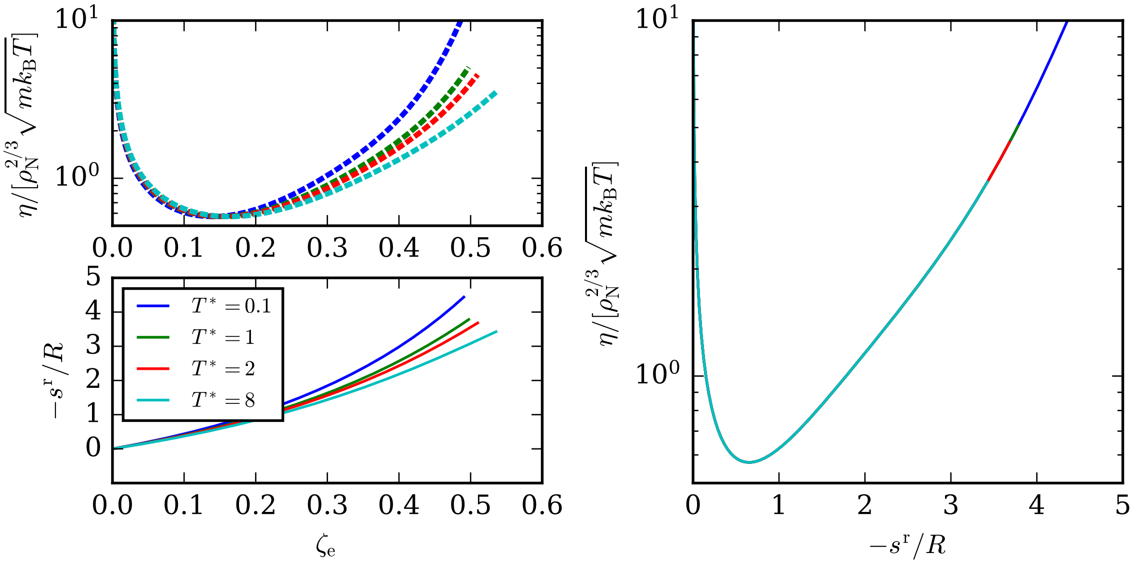


**Fig. S8.** Repulsive WCA potential: reduced viscosity and residual entropy, each plotted against scaling variable $\zeta_e$ as well as reduced viscosity plotted as a function of residual entropy. The maximum density for each value of $T^*$ was taken from Ahmed and Sadus(187).

***3.D.1. Simulation method.*** The molecular simulation results presented below for the repulsive WCA potential were carried out by William Krekelberg of NIST who has graciously given permission to present them in this work:

We perform molecular dynamics (MD) simulation in the microcanonical ensemble using $N = 4000$ particles of mass $m$ in a periodically replicated simulation box of dimension $L \times L \times L$ and volume $V = L^3$. The repulsive Weeks-Chandler-Andersen (WCA) model(188), with particle size $\sigma$ and energy scale $\varepsilon$, was used to model the fluid-fluid interactions. The equations of motion were integrated using the velocity-Verlet algorithm (189) with a reduced time step of $\Delta t^* = 0.0025$. The dimension $L$ was adjusted to achieve the desired reduced density $\rho^* = N/V$. Each system was equilibrated for $10^6$ time steps, during which velocity rescaling was performed every $10^3$ time steps to achieve the desired reduced temperature $T^* = 1.0$. Production runs of $10^7$ time steps were then performed in the microcanonical ensemble. Three independent simulations were performed at each density to obtain statistics. The reduced viscosity $\eta^*$ was calculated using the generalized Einstein relation discussed in Refs. (190, 191). The results of the simulations are given in Table S12.

**Table S12. Reduced viscosity $\eta^*$ from simulation of WCA fluid for several reduced densities $\rho^*$ at $T^* = 1.0$. The last column, $\sigma(\eta^*)$ is the standard deviation of the viscosity across three independent simulations.**

| $\rho^*$ | $\eta^*$ | $\sigma(\eta^*)$ |
|---|---|---|
| 0.05 | 0.174 | 0.003 |
| 0.10 | 0.178 | 0.009 |
| 0.15 | 0.195 | 0.008 |
| 0.20 | 0.206 | 0.002 |
| 0.25 | 0.227 | 0.005 |
| 0.30 | 0.26 | 0.02 |
| 0.35 | 0.30 | 0.01 |
| 0.40 | 0.34 | 0.01 |
| 0.45 | 0.40 | 0.01 |
| 0.50 | 0.45 | 0.02 |
| 0.55 | 0.549 | 0.005 |
| 0.60 | 0.71 | 0.04 |
| 0.65 | 0.81 | 0.02 |
| 0.70 | 1.04 | 0.01 |
| 0.75 | 1.30 | 0.04 |
| 0.80 | 1.66 | 0.04 |
| 0.85 | 2.2 | 0.1 |
| 0.90 | 3.24 | 0.07 |

 

**Table S13. Summary of the simulation results for viscosity for the Lennard-Jones 12-6 potential considered in this study ($N$: number of data points, $T^*$: range of simulation temperatures considered, $\rho^*$: range of simulation density)**

| Author | Year | $N$ | $T^*$ | $\rho^*$ |
|---|---|---|---|---|
| Baidakov et al. (192) | 2012 | 216 | 0.40-2.00 | 0.01-1.20 |
| Galliero et al. (193) | 2005 | 80 | 0.60-4.00 | 0.21-1.00 |
| Heyes (194) | 1988 | 206 | 0.72-10.00 | 0.20-1.22 |
| Meier et al. (195) | 2004 | 343 | 0.70-6.00 | 0.01-1.27 |
| Michels and Trappeniers (196) | 1985 | 36 | 1.30-10.00 | 0.05-0.30 |
| Oderji et al. (197) | 2011 | 167 | 0.70-30.20 | 0.00-0.05 |
| Vasquez et al. (198) | 2004 | 104 | 0.70-6.00 | 0.05-1.30 |

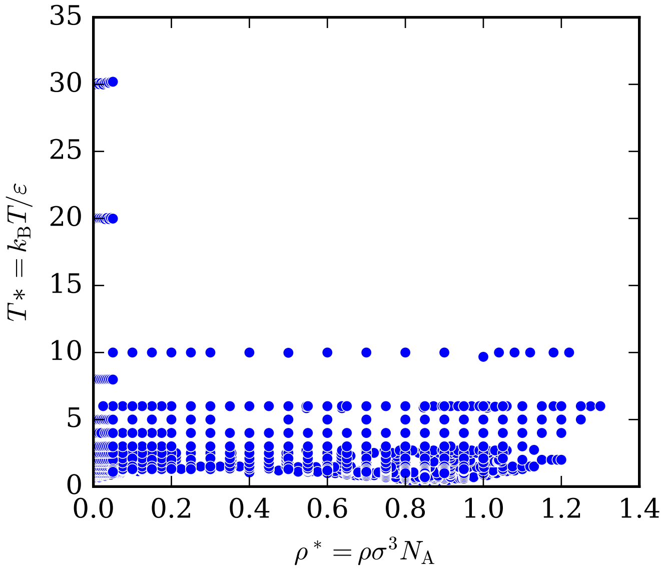


**Fig. S9.** Coverage of the simulated viscosity data for the Lennard-Jones 12-6 potential.

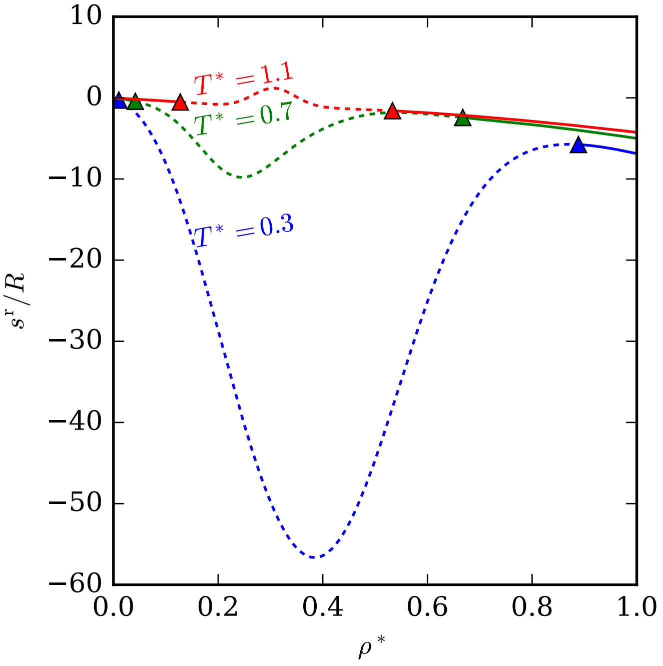


**Fig. S10.** Residual entropy along selected isotherms for the Lennard-Jones 12-6 potential. The critical temperature of the potential is $T_c^* = 1.32$. The approximate location of the spinodals (indicated by the markers) is identified by the roots of a Chebyshev expansion (199).

### 3.E. Lennard-Jones.

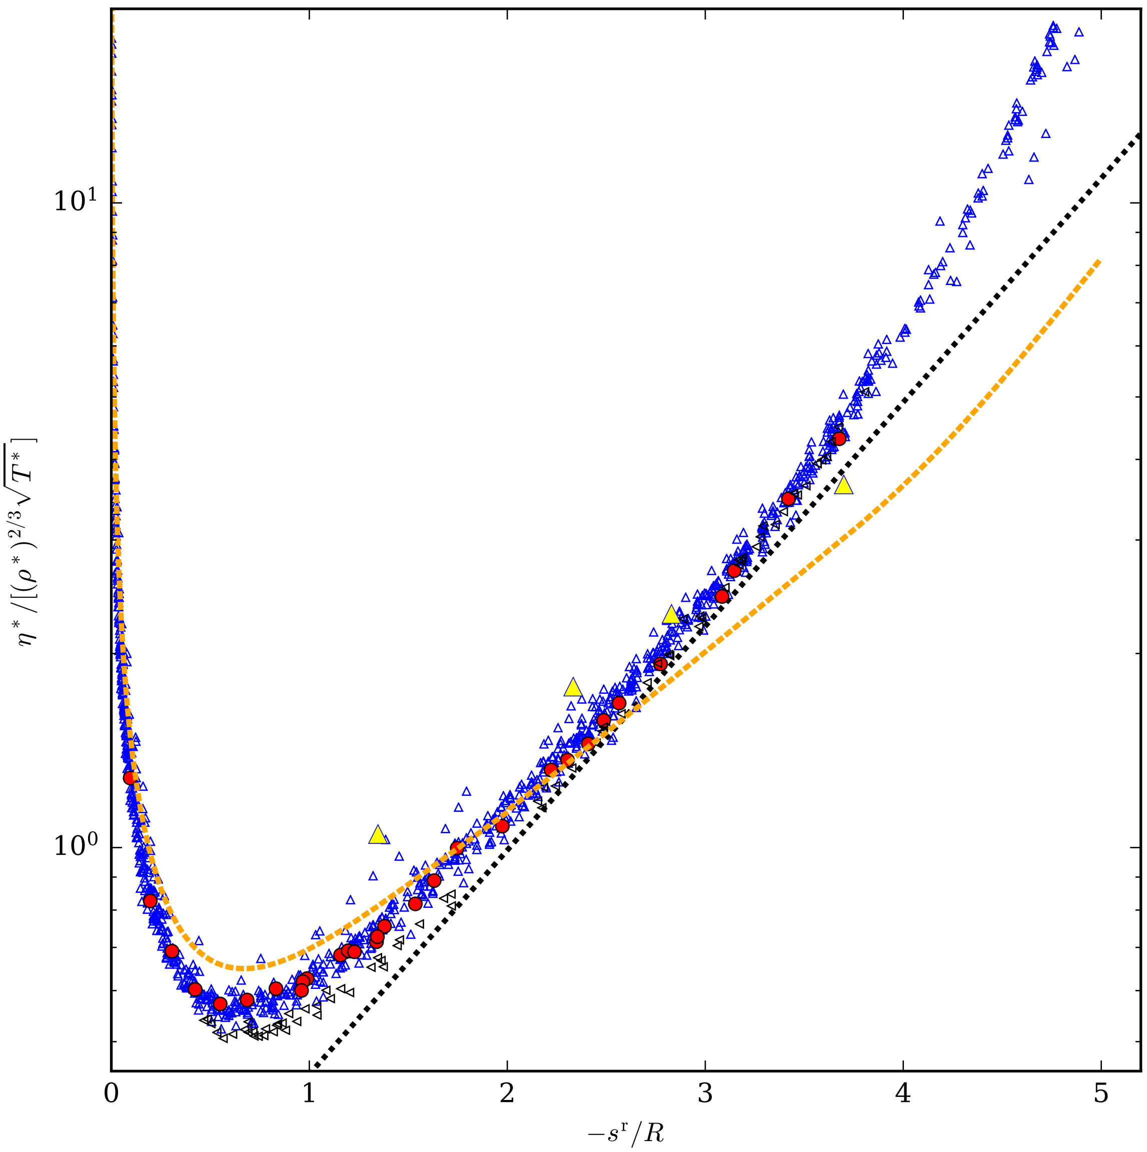


**Fig. S11.** Overlaid data for each of the model potentials studied in this work (blue △: Lennard-Jones 12-6 potential(192–198), black ◁: IPP with $n = 12$ (182), red ◯: repulsive WCA potential, yellow △: Lennard-Jones data from Ashurst and Hoover(200) considered by Rosenfeld (201), orange dashed curve: hard sphere (Enskog theory plus correction of (179)), black dashed line: correlation from Rosenfeld(202)).

### 3.F. Overview.

## 4. Residual Entropy Corresponding States

**4.A. Alternative Length Scales.** In the work of Noro and Frenkel (203) they note that for a wide range of potentials with an attractive contribution that the value of the "stickyness" parameter $\tau_{\rm NF}$ is given by the approximate value of 0.1. This "stickyness" parameter is related to the reduced second virial coefficient given by

$$B_2^* \equiv 1 - \frac{1}{4\tau_{\rm NF}} = \frac{B_2(T_{\rm c})}{\frac{2}{3}\pi\sigma_{\rm eff}^3} \quad [64]$$

and the equivalent hard sphere diameter can therefore be obtained from

$$\sigma_{\rm eff} = \sqrt[3]{\frac{B_2(T_{\rm c})}{\frac{2}{3}\pi\left(1-\frac{1}{4\tau_{\rm NF}}\right)}}. \quad [65]$$

The second virial coefficient $B_2(T_{\rm c})$ is evaluated from the equation of state (must be in units of $\mathrm{m}^3$/particle), and the length scale $\sigma_{\rm e}$ is obtained in units of meters. Figure S12 shows the results of this analysis. The effective length scales that are obtained by this method do not show a very linear relationship with the values of $\sigma$ fit for each fluid.

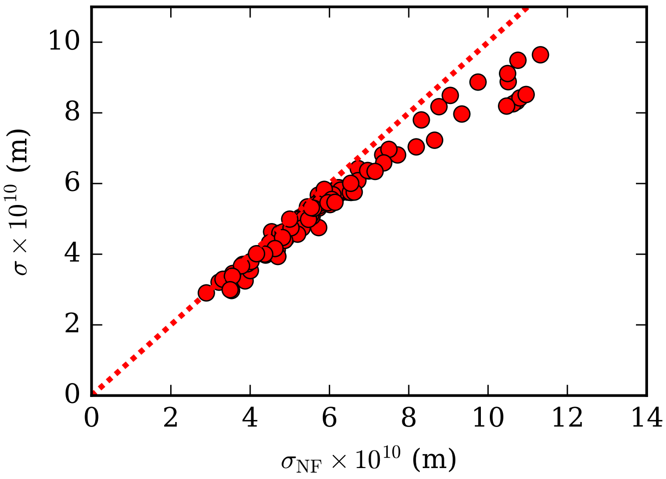


**Fig. S12.** Fitted values of $\sigma$ for each fluid for the mapping to the repulsive reference potential and the effective length scales obtained from the Noro-Frenkel universality for $\varepsilon/k_{\rm B} = T_{\rm c}/1.32$. The markers correspond to the full set of fluids from NIST REFPROP and with experimental viscosity data from NIST ThermoData Engine #103b version 10.1.

In Figs. S13 to S15 the fitted length scales are shown for $\varepsilon/k_{\rm B} = T_{\rm c}$ and $\varepsilon/k_{\rm B} = T_{\rm c}/0.7$ for each of the reference potentials.

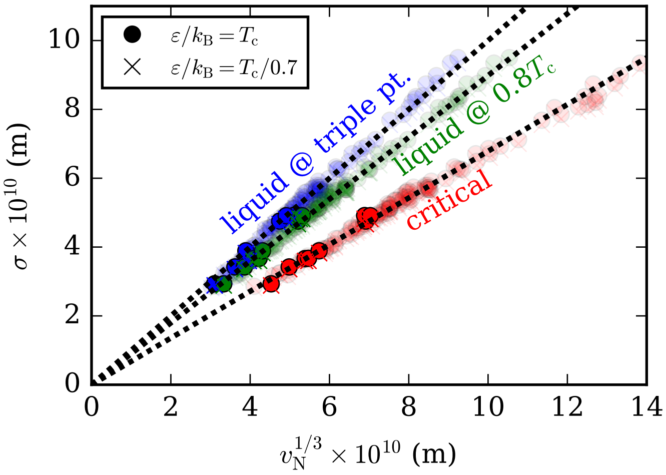


**Fig. S13.** Fitted values of $\sigma$ for each fluid for the mapping to the repulsive WCA reference potential. The slightly transparent markers correspond to the full set of fluids from NIST REFPROP and with experimental viscosity data from NIST ThermoData Engine #103b version 10.1, and the solid markers correspond to the eight molecular fluids selected in the main manuscript.

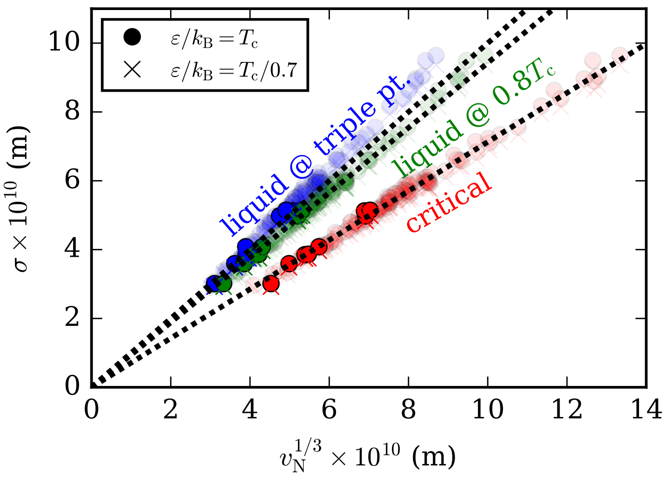


**Fig. S14.** Fitted values of $\sigma$ for each fluid for the mapping to the $n = 12$ IPP reference potential. The slightly transparent markers correspond to the full set of fluids from NIST REFPROP and with experimental viscosity data from NIST ThermoData Engine #103b version 10.1, and the solid markers correspond to the eight molecular fluids selected in the main manuscript.

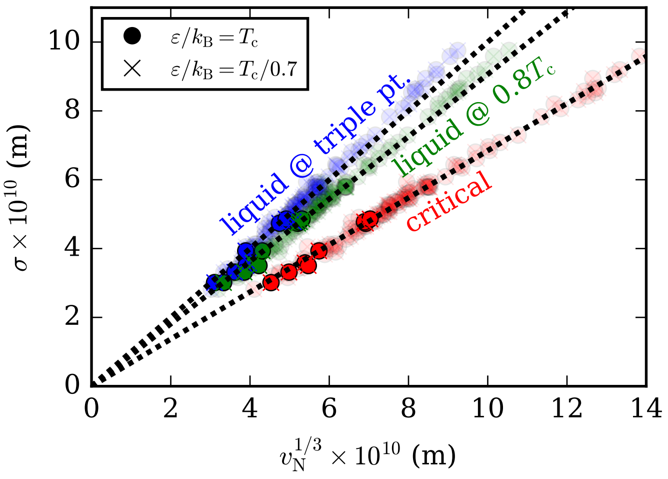


**Fig. S15.** Fitted values of $\sigma$ for each fluid for the mapping to the hard sphere reference potential. The slightly transparent markers correspond to the full set of fluids from NIST REFPROP and with experimental viscosity data from NIST ThermoData Engine #103b version 10.1, and the solid markers correspond to the eight molecular fluids selected in the main manuscript.

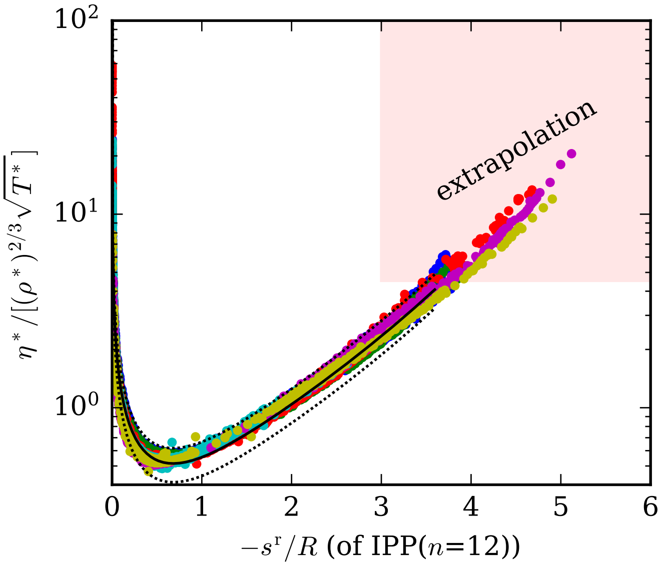


**Fig. S16.** Rosenfeld-scaled experimental data mapped onto the $n = 12$ IPP potential for the non-hydrogen-bonding fluids argon, methane, $CO_2$, $SF_6$, R-134a, and R-125.

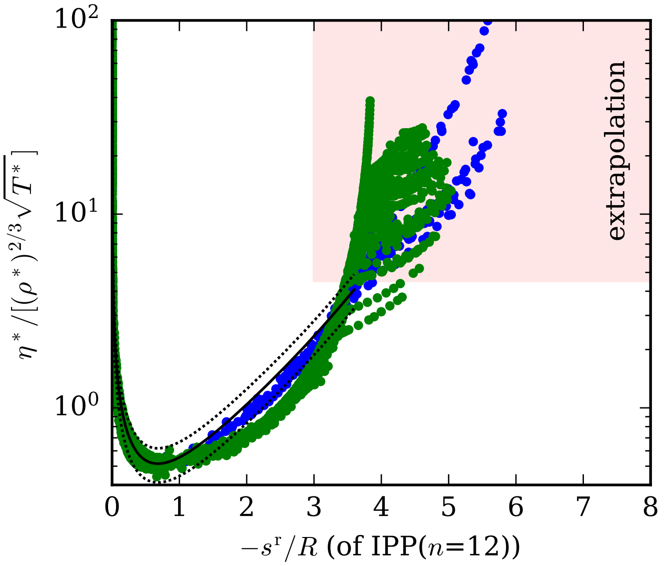


**Fig. S17.** Rosenfeld-scaled experimental data mapped onto the $n = 12$ IPP potential for the hydrogen-bonding fluids methanol and water.

### 4.B. IPP potential.

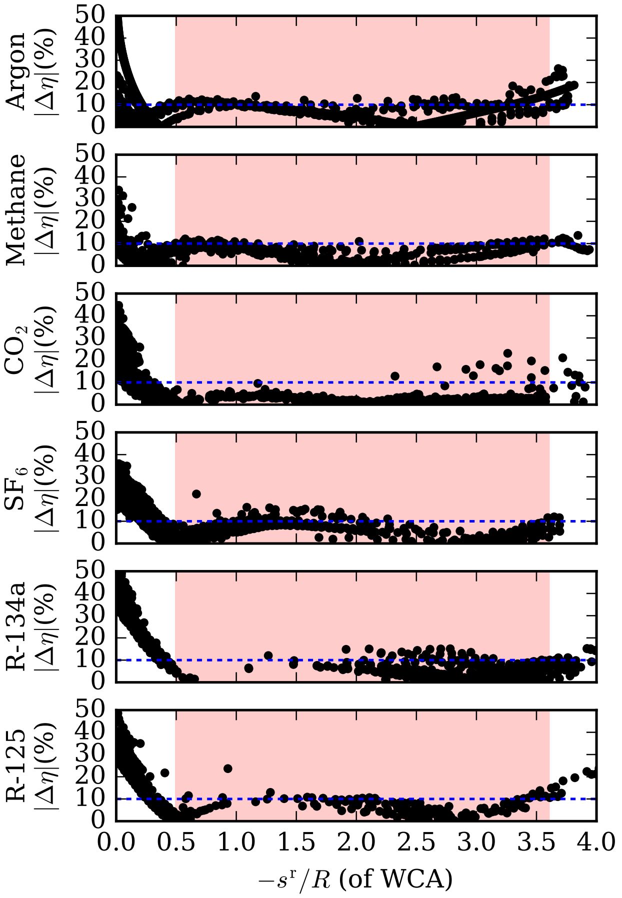


**Fig. S18.** Deviations between Rosenfeld-scaled experimental data mapped onto the $n = 12$ IPP potential and experimental data for the non-associating fluids argon, methane, $CO_2$, $SF_6$, R-134a, and R-125. Absolute deviation is given by $|\Delta\eta| = |(\eta_{\rm fit}/\eta_{\rm exp} - 1) \times 100|$. The colored rectangle is the approximate range of validity of this method, and the dashed line indicates 10%

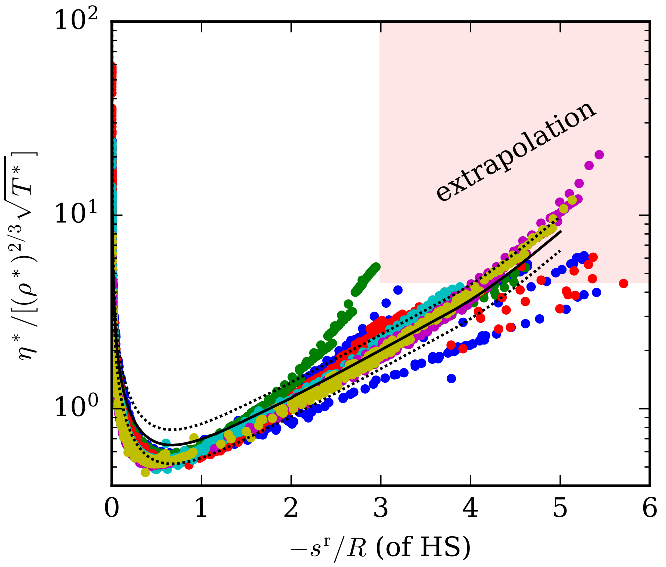


**Fig. S19.** Rosenfeld-scaled experimental data mapped onto the hard sphere potential for the non-hydrogen-bonding fluids argon, methane, $CO_2$, $SF_6$, R-134a, and R-125.

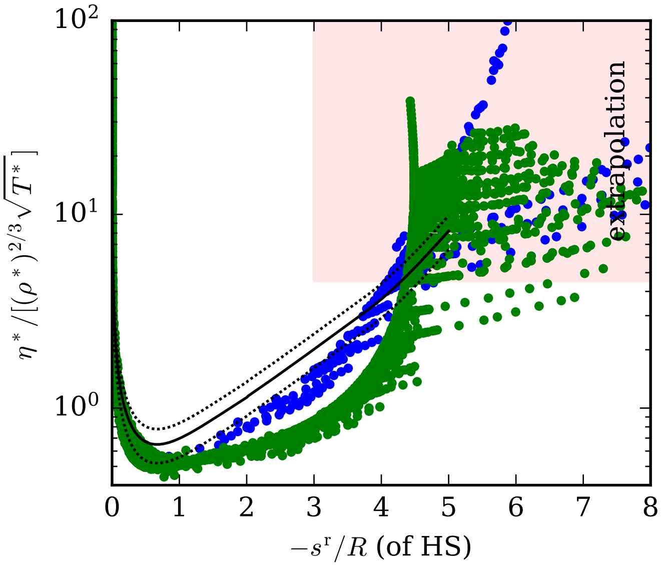


**Fig. S20.** Rosenfeld-scaled experimental data mapped onto the hard sphere potential for the hydrogen-bonding fluids methanol and water.

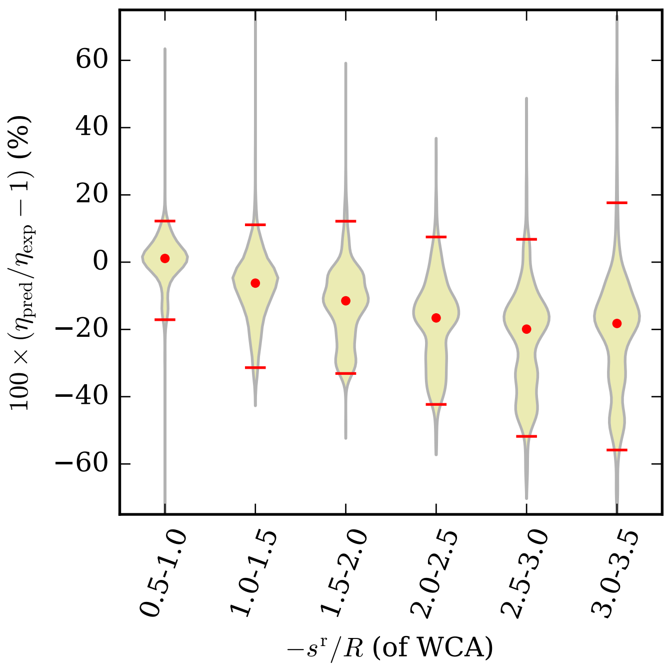


**Fig. S21.** Violin plots of the error in prediction of viscosity with values of $\sigma$ from the volume of the saturated liquid at $0.8T_{\rm c}$ for each fluid for the mapping to the repulsive WCA reference potential for non-associating fluids. The range of $-s^{\rm r}/R$ between 0.5 and 3.5 was split into bins of width 0.5. A violin distribution was constructed (by matplotlib(6)) for each data point that mapped into the bin. The plotted residual entropy corresponds to the center of the bin. The 97.5% and 2.5% percentiles are indicated with markers; the horizontal line is the median value. The dashed lines correspond to the divisions between bins.

## 4.C. Hard sphere.

## 5. Fitted parameters

**Table S14. Fitted values for $\sigma$ for the WCA potential**

| Fluid | Standard InChI key | $T_c$/K | $v_{N,t}^{1/3}$/nm | $v_{N,crit}^{1/3}$/nm | $v_{N,0.8T_c}^{1/3}$/nm | $\sigma(T_c/1.32)$/nm | $\sigma(T_c/1.0)$/nm | $\sigma(T_c/0.7)$/nm |
|---|---|---|---|---|---|---|---|---|
| 13BUTADIENE | KAKZBPTYRLMSJV-UHFFFAOYSA-N | 425.13 | 0.490 | 0.716 | 0.544 | 0.487 | 0.480 | 0.471 |
| 22DIMETHYLBUTANE | HNRMPXKDFBEGFZ-UHFFFAOYSA-N | 490.00 | 0.575 | 0.842 | 0.641 | 0.588 | 0.579 | 0.568 |
| 23DIMETHYLBUTANE | ZFFMLCVRJBZUDZ-UHFFFAOYSA-N | 500.60 | 0.567 | 0.840 | 0.638 | 0.583 | 0.574 | 0.564 |
| 3METHYLPENTANE | PFEOZHBOMNWTJB-UHFFFAOYSA-N | 506.00 | 0.557 | 0.842 | 0.639 | 0.578 | 0.569 | 0.559 |
| ACETONE | CSCPPACGZOOCGX-UHFFFAOYSA-N | 508.10 | 0.473 | 0.707 | 0.530 | 0.475 | 0.468 | 0.460 |
| AMMONIA | QGZKDVFQNNGYKY-UHFFFAOYSA-N | 405.56 | 0.338 | 0.495 | 0.369 | 0.324 | 0.319 | 0.314 |
| ARGON | XKRFYHLGVUSROY-UHFFFAOYSA-N | 150.69 | 0.361 | 0.498 | 0.385 | 0.345 | 0.340 | 0.333 |
| BENZENE | UHOVQNZJYSORNB-UHFFFAOYSA-N | 562.02 | 0.526 | 0.752 | 0.572 | 0.518 | 0.510 | 0.501 |
| BUTANE | IJDNQMDRQITEOD-UHFFFAOYSA-N | 425.12 | 0.509 | 0.751 | 0.571 | 0.520 | 0.512 | 0.502 |
| C11 | RSJKGSCJYJTIGS-UHFFFAOYSA-N | 638.80 | 0.695 | 1.031 | 0.775 | 0.704 | 0.693 | 0.682 |
| C12 | SNRUBQQJIBEYMU-UHFFFAOYSA-N | 658.10 | 0.716 | 1.077 | 0.798 | 0.723 | 0.712 | 0.700 |
| C16 | DCAYPVUWAIABOU-UHFFFAOYSA-N | 722.10 | 0.786 | 1.184 | 0.876 | 0.797 | 0.785 | 0.772 |
| C1CC6 | UAEPNZWRGJTJPN-UHFFFAOYSA-N | 572.20 | 0.567 | 0.848 | 0.645 | 0.588 | 0.580 | 0.570 |
| C22 | HOWGUJZVBDQJKV-UHFFFAOYSA-N | 792.20 | 0.872 | 1.319 | 0.975 | 0.888 | 0.876 | 0.861 |
| C3CC6 | DEDZSLCZHWTGOR-UHFFFAOYSA-N | 630.80 | 0.619 | 0.931 | 0.702 | 0.636 | 0.626 | 0.616 |
| C5F12 | NJCBUSHGCBERSK-UHFFFAOYSA-N | 421.00 | 0.616 | 0.915 | 0.688 | 0.642 | 0.633 | 0.622 |
| C6F14 | ZJIJAJXFLBMLCK-UHFFFAOYSA-N | 448.00 | 0.657 | 0.969 | 0.723 | 0.681 | 0.671 | 0.659 |
| CF3I | VPAYJEUHKVESSD-UHFFFAOYSA-N | 396.44 | 0.509 | 0.721 | 0.552 | 0.504 | 0.496 | 0.487 |
| CHLORINE | KZBUYRJDOAKODT-UHFFFAOYSA-N | 416.87 | 0.408 | 0.591 | 0.452 | 0.402 | 0.396 | 0.390 |
| CHLOROBENZENE | MVPPADPHJFYWMZ-UHFFFAOYSA-N | 632.35 | 0.542 | 0.800 | 0.604 | 0.541 | 0.533 | 0.524 |
| CO | UGFAIRIUMAVXCW-UHFFFAOYSA-N | 132.86 | 0.381 | 0.535 | 0.411 | 0.369 | 0.364 | 0.357 |
| CO2 | CURLTUGMZLYLDI-UHFFFAOYSA-N | 304.13 | 0.397 | 0.539 | 0.408 | 0.373 | 0.368 | 0.361 |
| CYCLOHEX | XDTMQSROBMDMFD-UHFFFAOYSA-N | 553.60 | 0.562 | 0.802 | 0.609 | 0.562 | 0.553 | 0.544 |
| CYCLOPEN | RGSFGYAAUTVSQA-UHFFFAOYSA-N | 511.72 | 0.516 | 0.751 | 0.575 | 0.523 | 0.515 | 0.506 |
| D2 | UFHFLCQGNIYNRP-VVKOMZTBSA-N | 38.34 | 0.340 | 0.458 | 0.362 | 0.321 | 0.316 | 0.311 |
| D2O | XLYOFNOQVPJJNP-ZSJDYOACSA-N | 643.85 | 0.311 | 0.454 | 0.333 | 0.297 | 0.293 | 0.288 |
| D4 | HMMGMWAXVFQUOA-UHFFFAOYSA-N | 586.50 | 0.801 | 1.168 | 0.875 | 0.817 | 0.805 | 0.791 |
| D5 | XMSXQFUHVRWGNA-UHFFFAOYSA-N | 618.30 | 0.843 | 1.265 | 0.947 | 0.887 | 0.874 | 0.858 |
| D6 | IUMSDRXLFWAGNT-UHFFFAOYSA-N | 645.78 | 0.905 | 1.383 | 1.015 | 0.949 | 0.934 | 0.918 |
| DEA | ZBCBWPMODOFKDW-UHFFFAOYSA-N | 736.50 | 0.543 | 0.795 | 0.589 | 0.569 | 0.560 | 0.550 |
| DECANE | DIOQZVSQGTUSAI-UHFFFAOYSA-N | 617.70 | 0.675 | 1.004 | 0.751 | 0.681 | 0.671 | 0.660 |
| DEE | RTZKZFJDLAIYFH-UHFFFAOYSA-N | 466.70 | nan | 0.775 | 0.587 | 0.530 | 0.522 | 0.513 |
| DMC | IEJIGPNLZYLLBP-UHFFFAOYSA-N | 557.00 | 0.516 | 0.746 | 0.562 | 0.506 | 0.499 | 0.490 |
| DME | LCGLNKUTAGEVQW-UHFFFAOYSA-N | 400.38 | 0.443 | 0.654 | 0.497 | 0.444 | 0.437 | 0.429 |
| EBENZENE | YNQLUTRBYVCPMQ-UHFFFAOYSA-N | 617.12 | 0.567 | 0.846 | 0.642 | 0.576 | 0.567 | 0.558 |
| EGLYCOL | LYCAIKOWRPUZTN-UHFFFAOYSA-N | 719.00 | 0.450 | 0.656 | 0.492 | 0.464 | 0.457 | 0.449 |
| ETHANE | OTMSDBZUPAUEDD-UHFFFAOYSA-N | 305.32 | 0.425 | 0.623 | 0.478 | 0.432 | 0.426 | 0.417 |
| ETHANOL | LFQSCWFLJHTTHZ-UHFFFAOYSA-N | 514.71 | 0.439 | 0.654 | 0.486 | 0.460 | 0.453 | 0.445 |
| ETHYLENE | VGGSQFUCUMXWEO-UHFFFAOYSA-N | 282.35 | 0.415 | 0.601 | 0.461 | 0.407 | 0.401 | 0.395 |
| ETHYLENEOXIDE | IAYPIBMASNFSPL-UHFFFAOYSA-N | 468.92 | 0.413 | 0.614 | 0.463 | 0.412 | 0.406 | 0.399 |
| FLUORINE | PXGOKWXKJXAPGV-UHFFFAOYSA-N | 144.41 | 0.334 | 0.474 | 0.369 | 0.329 | 0.324 | 0.319 |
| H2S | RWSOTUBLDIXVET-UHFFFAOYSA-N | 373.10 | 0.385 | 0.546 | 0.418 | 0.373 | 0.367 | 0.361 |
| HCL | VEXZGXHMUGYJMC-UHFFFAOYSA-N | 324.68 | 0.365 | 0.519 | 0.396 | 0.354 | 0.348 | 0.342 |
| HEPTANE | IMNFDUFMRHMDMM-UHFFFAOYSA-N | 540.20 | 0.599 | 0.893 | 0.672 | 0.608 | 0.599 | 0.589 |
| HEXANE | VLKZOEOYAKHREP-UHFFFAOYSA-N | 507.82 | 0.574 | 0.850 | 0.641 | 0.582 | 0.573 | 0.563 |
| HYDROGEN | UFHFLCQGNIYNRP-UHFFFAOYSA-N | 33.15 | 0.354 | 0.475 | 0.378 | 0.329 | 0.324 | 0.319 |

Continued on next page...

Table S14 – continued from previous page

| Fluid | Standard InChI key | $T_c$/K | $v_{N,t}^{1/3}$/nm | $v_{N,crit}^{1/3}$/nm | $v_{N,0.8T_c}^{1/3}$/nm | $\sigma(T_c/1.32)$/nm | $\sigma(T_c/1.0)$/nm | $\sigma(T_c/0.7)$/nm |
|---|---|---|---|---|---|---|---|---|
| IBUTENE | VQTUBCCKSQIDNK-UHFFFAOYSA-N | 418.09 | 0.496 | 0.736 | 0.557 | 0.504 | 0.496 | 0.487 |
| IHEXANE | AFABGHUZZDYHJO-UHFFFAOYSA-N | 497.70 | 0.562 | 0.849 | 0.641 | 0.581 | 0.573 | 0.563 |
| IOCTANE | NHTMVDHEPJAVLT-UHFFFAOYSA-N | 544.00 | 0.621 | 0.922 | 0.698 | 0.637 | 0.628 | 0.617 |
| IPENTANE | QWTDNUCVQCZILF-UHFFFAOYSA-N | 460.35 | 0.534 | 0.798 | 0.607 | 0.551 | 0.543 | 0.534 |
| ISOBUTAN | NNPPMTNAJDCUHE-UHFFFAOYSA-N | 407.81 | 0.507 | 0.754 | 0.573 | 0.521 | 0.514 | 0.504 |
| KRYPTON | DNNSSWSSYDEUBZ-UHFFFAOYSA-N | 209.48 | 0.385 | 0.535 | 0.412 | 0.371 | 0.365 | 0.358 |
| MD2M | YFCGDEUVHLPRCZ-UHFFFAOYSA-N | 599.40 | 0.818 | 1.243 | 0.925 | 0.849 | 0.837 | 0.823 |
| MD3M | FBZANXDWQAVSTQ-UHFFFAOYSA-N | 628.96 | 0.870 | 1.334 | 0.993 | 0.911 | 0.898 | 0.883 |
| MD4M | ADANNTOYRVPQLJ-UHFFFAOYSA-N | 653.20 | 0.924 | 1.428 | 1.054 | 0.964 | 0.950 | 0.934 |
| MDM | CXQXSVUQTKDNFP-UHFFFAOYSA-N | 565.36 | 0.752 | 1.136 | 0.850 | 0.780 | 0.768 | 0.755 |
| MEA | HZAXFHJVJLSVMW-UHFFFAOYSA-N | 671.40 | 0.463 | 0.675 | 0.507 | 0.479 | 0.472 | 0.464 |
| METHANE | VNWKTOKETHGBQD-UHFFFAOYSA-N | 190.56 | 0.390 | 0.547 | 0.423 | 0.373 | 0.367 | 0.359 |
| METHANOL | OKKJLVBELUTLKV-UHFFFAOYSA-N | 513.38 | 0.389 | 0.574 | 0.431 | 0.398 | 0.392 | 0.385 |
| MLINOLEA | WTTJVINHCBCLGX-NQLNTKRDSA-N | 799.00 | 0.808 | 1.271 | 0.918 | 0.832 | 0.821 | 0.807 |
| MLINOLEN | DVWSXZIHSUZZKJ-YSTUJMKBSA-N | 772.00 | nan | 1.251 | 0.905 | 0.826 | 0.814 | 0.801 |
| MM | UQEAIHBTYFGYIE-UHFFFAOYSA-N | 518.70 | 0.681 | 1.002 | 0.757 | 0.697 | 0.686 | 0.674 |
| MOLEATE | QYDYPVFESGNLHU-KHPPLWFESA-N | 782.00 | 0.817 | 1.269 | 0.926 | 0.842 | 0.830 | 0.817 |
| MPALMITA | FLIACVVOZYBSBS-UHFFFAOYSA-N | 755.00 | nan | 1.228 | 0.895 | 0.819 | 0.808 | 0.794 |
| MSTEARAT | HPEUJPJOZXNMSJ-UHFFFAOYSA-N | 775.00 | 0.836 | 1.279 | 0.931 | 0.852 | 0.840 | 0.826 |
| MXYLENE | IVSZLXZYQVIEFR-UHFFFAOYSA-N | 616.89 | 0.577 | 0.854 | 0.642 | 0.575 | 0.566 | 0.557 |
| N2O | GQPLMRYTRLFLPF-UHFFFAOYSA-N | 309.52 | 0.390 | 0.545 | 0.415 | 0.379 | 0.374 | 0.367 |
| NEON | GKAOGPIIYCISHV-UHFFFAOYSA-N | 44.40 | 0.302 | 0.410 | 0.319 | 0.290 | 0.286 | 0.281 |
| NEOPENTN | CRSOQBOWXPBRES-UHFFFAOYSA-N | 433.74 | 0.576 | 0.798 | 0.611 | 0.573 | 0.564 | 0.554 |
| NITROGEN | IJGRMHOSHXDMSA-UHFFFAOYSA-N | 126.19 | 0.378 | 0.530 | 0.408 | 0.367 | 0.362 | 0.355 |
| NONANE | BKIMMITUMNQMOS-UHFFFAOYSA-N | 594.55 | 0.650 | 0.972 | 0.726 | 0.658 | 0.649 | 0.638 |
| OCTANE | TVMXDCGIABBOFY-UHFFFAOYSA-N | 568.74 | 0.629 | 0.935 | 0.700 | 0.634 | 0.625 | 0.614 |
| OXYGEN | MYMOFIZGZYHOMD-UHFFFAOYSA-N | 154.58 | 0.345 | 0.496 | 0.383 | 0.338 | 0.333 | 0.327 |
| OXYLENE | CTQNGGLPUBDAKN-UHFFFAOYSA-N | 630.26 | 0.577 | 0.852 | 0.639 | 0.575 | 0.567 | 0.557 |
| PENTANE | OFBQJSOFQDEBGM-UHFFFAOYSA-N | 469.70 | 0.540 | 0.803 | 0.608 | 0.554 | 0.546 | 0.536 |
| PROPANE | ATUOYWHBWRKTHZ-UHFFFAOYSA-N | 369.89 | 0.464 | 0.693 | 0.529 | 0.481 | 0.474 | 0.465 |
| PROPYLEN | QQONPFPTGQHPMA-UHFFFAOYSA-N | 364.21 | 0.450 | 0.673 | 0.513 | 0.463 | 0.456 | 0.447 |
| PROPYLENEOXIDE | GOOHAUXETOMSMM-UHFFFAOYSA-N | 488.11 | 0.461 | 0.685 | 0.519 | 0.467 | 0.460 | 0.452 |
| PXYLENE | URLKBWYHVLBVBO-UHFFFAOYSA-N | 616.17 | 0.588 | 0.851 | 0.643 | 0.576 | 0.567 | 0.558 |
| R11 | CYRMSUTZVYGINF-UHFFFAOYSA-N | 471.11 | 0.506 | 0.744 | 0.565 | 0.517 | 0.509 | 0.500 |
| R113 | AJDIZQLSFPQPEY-UHFFFAOYSA-N | 487.21 | 0.568 | 0.822 | 0.618 | 0.573 | 0.564 | 0.554 |
| R114 | DDMOUSALMHHKOS-UHFFFAOYSA-N | 418.83 | nan | 0.788 | 0.597 | 0.552 | 0.544 | 0.534 |
| R115 | RFCAUADVODFSLZ-UHFFFAOYSA-N | 353.10 | 0.528 | 0.747 | 0.574 | 0.534 | 0.526 | 0.516 |
| R12 | PXBRQCKWGAHEHS-UHFFFAOYSA-N | 385.12 | 0.479 | 0.708 | 0.540 | 0.495 | 0.487 | 0.478 |
| R123 | OHMHBGPWCHTMQE-UHFFFAOYSA-N | 456.83 | 0.524 | 0.773 | 0.584 | 0.537 | 0.529 | 0.519 |
| R1233ZDE | LDTMPQQAWUMPKS-OWOJBTEDSA-N | 439.60 | 0.527 | 0.767 | 0.578 | 0.545 | 0.537 | 0.527 |
| R1234YF | FXRLMCRCYDHQFW-UHFFFAOYSA-N | 367.85 | 0.496 | 0.736 | 0.555 | 0.510 | 0.502 | 0.493 |
| R1234ZEE | CDOOAUSHHFGWSA-OWOJBTEDSA-N | 382.51 | 0.501 | 0.729 | 0.550 | 0.508 | 0.500 | 0.491 |
| R124 | BOUGCJDAQLKBQH-UHFFFAOYSA-N | 395.43 | nan | 0.740 | 0.560 | 0.520 | 0.512 | 0.502 |
| R125 | GTLACDSXYULKMZ-UHFFFAOYSA-N | 339.17 | 0.491 | 0.703 | 0.531 | 0.498 | 0.490 | 0.481 |
| R13 | AFYPFACVUDMOHA-UHFFFAOYSA-N | 302.00 | 0.454 | 0.668 | 0.510 | 0.463 | 0.456 | 0.447 |
| R134A | LVGUZGTVOIAKKC-UHFFFAOYSA-N | 374.21 | 0.475 | 0.692 | 0.520 | 0.483 | 0.476 | 0.467 |
| R14 | TXEYQDLBPFQVAA-UHFFFAOYSA-N | 227.51 | nan | 0.616 | 0.473 | 0.432 | 0.425 | 0.416 |
| R141B | FRCHKSNAZZFGCA-UHFFFAOYSA-N | 477.50 | 0.510 | 0.751 | 0.570 | 0.519 | 0.512 | 0.503 |
| R142B | BHNZEZWIUMJCGF-UHFFFAOYSA-N | 410.26 | 0.487 | 0.721 | 0.545 | 0.500 | 0.493 | 0.484 |

Continued on next page...

Table S14 – continued from previous page

| Fluid | Standard InChI key | $T_c$/K | $v_{N,t}^{1/3}$/nm | $v_{N,crit}^{1/3}$/nm | $v_{N,0.8T_c}^{1/3}$/nm | $\sigma(T_c/1.32)$/nm | $\sigma(T_c/1.0)$/nm | $\sigma(T_c/0.7)$/nm |
|---|---|---|---|---|---|---|---|---|
| R143A | UJPMYEOUBPIPHQ-UHFFFAOYSA-N | 345.86 | 0.472 | 0.687 | 0.517 | 0.474 | 0.467 | 0.458 |
| R150 | WSLDOOZREJYCGB-UHFFFAOYSA-N | 561.60 | 0.498 | 0.727 | 0.550 | 0.499 | 0.491 | 0.483 |
| R152A | NPNPZTNLOVBDOC-UHFFFAOYSA-N | 386.41 | 0.452 | 0.668 | 0.501 | 0.457 | 0.450 | 0.442 |
| R161 | UHCBBWUQDAVSMS-UHFFFAOYSA-N | 375.25 | 0.437 | 0.642 | 0.487 | 0.439 | 0.432 | 0.424 |
| R21 | UMNKXPULIDJLSU-UHFFFAOYSA-N | 451.48 | nan | 0.687 | 0.523 | 0.475 | 0.467 | 0.459 |
| R218 | QYSGYZVSCZSLHT-UHFFFAOYSA-N | 345.02 | 0.538 | 0.792 | 0.601 | 0.567 | 0.558 | 0.548 |
| R22 | VOPWNXZWBYDODV-UHFFFAOYSA-N | 369.30 | 0.437 | 0.650 | 0.493 | 0.447 | 0.440 | 0.432 |
| R227EA | YFMFNYKEUDLDTL-UHFFFAOYSA-N | 374.90 | 0.532 | 0.780 | 0.589 | 0.556 | 0.548 | 0.537 |
| R23 | XPDWGBQVDMORPB-UHFFFAOYSA-N | 299.29 | 0.409 | 0.604 | 0.454 | 0.411 | 0.404 | 0.397 |
| R236EA | FYIRUPZTYPILDH-UHFFFAOYSA-N | 412.44 | nan | 0.765 | 0.577 | 0.543 | 0.535 | 0.525 |
| R236FA | NSGXIBWMJZWTPY-UHFFFAOYSA-N | 398.07 | 0.529 | 0.771 | 0.581 | 0.544 | 0.536 | 0.526 |
| R245CA | AWTOFSDLNREIFS-UHFFFAOYSA-N | 447.57 | 0.516 | 0.751 | 0.567 | 0.530 | 0.522 | 0.512 |
| R245FA | MSSNHSVIGIHOJA-UHFFFAOYSA-N | 427.01 | 0.514 | 0.754 | 0.569 | 0.532 | 0.523 | 0.514 |
| R32 | RWRIWBAIICGTTQ-UHFFFAOYSA-N | 351.25 | 0.393 | 0.588 | 0.438 | 0.394 | 0.387 | 0.380 |
| R365MFC | WZLFPVPRZGTCKP-UHFFFAOYSA-N | 460.00 | 0.564 | 0.804 | 0.609 | 0.568 | 0.560 | 0.550 |
| R40 | NEHMKBQYUWJMIP-UHFFFAOYSA-N | 416.30 | nan | 0.613 | 0.465 | 0.416 | 0.410 | 0.402 |
| RC318 | BCCOBQSFUDVTJQ-UHFFFAOYSA-N | 388.38 | 0.578 | 0.812 | 0.612 | 0.583 | 0.574 | 0.563 |
| RE245CB2 | GCDWNCOAODIANN-UHFFFAOYSA-N | 406.81 | 0.563 | 0.793 | 0.596 | 0.555 | 0.546 | 0.536 |
| RE245FA2 | ZASBKNPRLPFSCA-UHFFFAOYSA-N | 444.88 | 0.550 | 0.785 | 0.589 | 0.546 | 0.537 | 0.528 |
| RE347MCC | NOPJRYAFUXTDLX-UHFFFAOYSA-N | 437.70 | 0.572 | 0.857 | 0.643 | 0.601 | 0.591 | 0.581 |
| SF6 | SFZCNBIFKDRMGX-UHFFFAOYSA-N | 318.72 | 0.509 | 0.689 | 0.525 | 0.499 | 0.491 | 0.482 |
| SO2 | RAHZWNYVWXNFOC-UHFFFAOYSA-N | 430.64 | 0.403 | 0.590 | 0.443 | 0.400 | 0.394 | 0.387 |
| TOLUENE | YXFVVABEGXRONW-UHFFFAOYSA-N | 591.75 | 0.540 | 0.806 | 0.609 | 0.547 | 0.539 | 0.530 |
| WATER | XLYOFNOQVPJJNP-UHFFFAOYSA-N | 647.10 | 0.310 | 0.453 | 0.333 | 0.299 | 0.295 | 0.290 |
| XENON | FHNFHKCVQCLJFQ-UHFFFAOYSA-N | 289.73 | 0.420 | 0.583 | 0.448 | 0.401 | 0.395 | 0.388 |

**Table S15. Fitted values for $\sigma$ for the IPP($n = 12$) potential**

| Fluid | Standard InChI key | $T_c$/K | $v_{N,t}^{1/3}$/nm | $v_{N,crit}^{1/3}$/nm | $v_{N,0.8T_c}^{1/3}$/nm | $\sigma(T_c/1.32)$/nm | $\sigma(T_c/1.0)$/nm | $\sigma(T_c/0.7)$/nm |
|---|---|---|---|---|---|---|---|---|
| 13BUTADIENE | KAKZBPTYRLMSJV-UHFFFAOYSA-N | 425.13 | 0.490 | 0.716 | 0.544 | 0.512 | 0.500 | 0.485 |
| 22DIMETHYLBUTANE | HNRMPXKDFBEGFZ-UHFFFAOYSA-N | 490.00 | 0.575 | 0.842 | 0.641 | 0.623 | 0.609 | 0.591 |
| 23DIMETHYLBUTANE | ZFFMLCVRJBZUDZ-UHFFFAOYSA-N | 500.60 | 0.567 | 0.840 | 0.638 | 0.617 | 0.603 | 0.585 |
| 3METHYLPENTANE | PFEOZHBOMNWTJB-UHFFFAOYSA-N | 506.00 | 0.557 | 0.842 | 0.639 | 0.610 | 0.596 | 0.579 |
| ACETONE | CSCPPACGZOOCGX-UHFFFAOYSA-N | 508.10 | 0.473 | 0.707 | 0.530 | 0.500 | 0.489 | 0.475 |
| AMMONIA | QGZKDVFQNNGYKY-UHFFFAOYSA-N | 405.56 | 0.338 | 0.495 | 0.369 | 0.342 | 0.335 | 0.325 |
| ARGON | XKRFYHLGVUSROY-UHFFFAOYSA-N | 150.69 | 0.361 | 0.498 | 0.385 | 0.367 | 0.359 | 0.349 |
| BENZENE | UHOVQNZJYSORNB-UHFFFAOYSA-N | 562.02 | 0.526 | 0.752 | 0.572 | 0.548 | 0.536 | 0.520 |
| BUTANE | IJDNQMDRQITEOD-UHFFFAOYSA-N | 425.12 | 0.509 | 0.751 | 0.571 | 0.548 | 0.536 | 0.520 |
| C11 | RSJKGSCJYJTIGS-UHFFFAOYSA-N | 638.80 | 0.695 | 1.031 | 0.775 | 0.751 | 0.734 | 0.713 |
| C12 | SNRUBQQJIBEYMU-UHFFFAOYSA-N | 658.10 | 0.716 | 1.077 | 0.798 | 0.774 | 0.756 | 0.734 |
| C16 | DCAYPVUWAIABOU-UHFFFAOYSA-N | 722.10 | 0.786 | 1.184 | 0.876 | 0.859 | 0.839 | 0.814 |
| C1CC6 | UAEPNZWRGJTJPN-UHFFFAOYSA-N | 572.20 | 0.567 | 0.848 | 0.645 | 0.625 | 0.611 | 0.593 |
| C3CC6 | DEDZSLCZHWTGOR-UHFFFAOYSA-N | 630.80 | 0.619 | 0.931 | 0.702 | 0.676 | 0.660 | 0.641 |
| C5F12 | NJCBUSHGCBERSK-UHFFFAOYSA-N | 421.00 | 0.616 | 0.915 | 0.688 | 0.690 | 0.674 | 0.654 |
| C6F14 | ZJIJAJXFLBMLCK-UHFFFAOYSA-N | 448.00 | 0.657 | 0.969 | 0.723 | 0.730 | 0.714 | 0.693 |
| CF3I | VPAYJEUHKVESSD-UHFFFAOYSA-N | 396.44 | 0.509 | 0.721 | 0.552 | 0.531 | 0.519 | 0.504 |
| CHLORINE | KZBUYRJDOAKODT-UHFFFAOYSA-N | 416.87 | 0.408 | 0.591 | 0.452 | 0.424 | 0.414 | 0.402 |
| CHLOROBENZENE | MVPPADPHJFYWMZ-UHFFFAOYSA-N | 632.35 | 0.542 | 0.800 | 0.604 | 0.571 | 0.558 | 0.542 |
| CO | UGFAIRIUMAVXCW-UHFFFAOYSA-N | 132.86 | 0.381 | 0.535 | 0.411 | 0.389 | 0.380 | 0.369 |
| CO2 | CURLTUGMZLYLDI-UHFFFAOYSA-N | 304.13 | 0.397 | 0.539 | 0.408 | 0.395 | 0.386 | 0.375 |
| CYCLOHEX | XDTMQSROBMDMFD-UHFFFAOYSA-N | 553.60 | 0.562 | 0.802 | 0.609 | 0.599 | 0.585 | 0.568 |
| CYCLOPEN | RGSFGYAAUTVSQA-UHFFFAOYSA-N | 511.72 | 0.516 | 0.751 | 0.575 | 0.555 | 0.542 | 0.526 |
| D2 | UFHFLCQGNIYNRP-VVKOMZTBSA-N | 38.34 | 0.340 | 0.458 | 0.362 | 0.336 | 0.328 | 0.319 |
| D2O | XLYOFNOQVPJJNP-ZSJDYOACSA-N | 643.85 | 0.311 | 0.454 | 0.333 | 0.306 | 0.299 | 0.291 |
| D4 | HMMGMWAXVFQUOA-UHFFFAOYSA-N | 586.50 | 0.801 | 1.168 | 0.875 | 0.883 | 0.862 | 0.837 |
| D5 | XMSXQFUHVRWGNA-UHFFFAOYSA-N | 618.30 | 0.843 | 1.265 | 0.947 | 0.971 | 0.949 | 0.921 |
| DECANE | DIOQZVSQGTUSAI-UHFFFAOYSA-N | 617.70 | 0.675 | 1.004 | 0.751 | 0.727 | 0.710 | 0.689 |
| DEE | RTZKZFJDLAIYFH-UHFFFAOYSA-N | 466.70 | nan | 0.775 | 0.587 | 0.558 | 0.545 | 0.529 |
| DMC | IEJIGPNLZYLLBP-UHFFFAOYSA-N | 557.00 | 0.516 | 0.746 | 0.562 | 0.535 | 0.523 | 0.508 |
| DME | LCGLNKUTAGEVQW-UHFFFAOYSA-N | 400.38 | 0.443 | 0.654 | 0.497 | 0.467 | 0.456 | 0.443 |
| EBENZENE | YNQLUTRBYVCPMQ-UHFFFAOYSA-N | 617.12 | 0.567 | 0.846 | 0.642 | 0.609 | 0.595 | 0.578 |
| EGLYCOL | LYCAIKOWRPUZTN-UHFFFAOYSA-N | 719.00 | 0.450 | 0.656 | 0.492 | 0.490 | 0.479 | 0.465 |
| ETHANE | OTMSDBZUPAUEDD-UHFFFAOYSA-N | 305.32 | 0.425 | 0.623 | 0.478 | 0.456 | 0.446 | 0.433 |
| ETHANOL | LFQSCWFLJHTTHZ-UHFFFAOYSA-N | 514.71 | 0.439 | 0.654 | 0.486 | 0.491 | 0.479 | 0.465 |
| ETHYLENE | VGGSQFUCUMXWEO-UHFFFAOYSA-N | 282.35 | 0.415 | 0.601 | 0.461 | 0.429 | 0.420 | 0.407 |
| ETHYLENEOXIDE | IAYPIBMASNFSPL-UHFFFAOYSA-N | 468.92 | 0.413 | 0.614 | 0.463 | 0.433 | 0.423 | 0.411 |
| FLUORINE | PXGOKWXKJXAPGV-UHFFFAOYSA-N | 144.41 | 0.334 | 0.474 | 0.369 | 0.346 | 0.338 | 0.329 |
| H2S | RWSOTUBLDIXVET-UHFFFAOYSA-N | 373.10 | 0.385 | 0.546 | 0.418 | 0.392 | 0.383 | 0.372 |
| HCL | VEXZGXHMUGYJMC-UHFFFAOYSA-N | 324.68 | 0.365 | 0.519 | 0.396 | 0.374 | 0.365 | 0.354 |
| HEPTANE | IMNFDUFMRHMDMM-UHFFFAOYSA-N | 540.20 | 0.599 | 0.893 | 0.672 | 0.643 | 0.629 | 0.610 |
| HEXANE | VLKZOEOYAKHREP-UHFFFAOYSA-N | 507.82 | 0.574 | 0.850 | 0.641 | 0.614 | 0.600 | 0.582 |
| IBUTENE | VQTUBCCKSQIDNK-UHFFFAOYSA-N | 418.09 | 0.496 | 0.736 | 0.557 | 0.530 | 0.518 | 0.502 |
| IHEXANE | AFABGHUZZDYHJO-UHFFFAOYSA-N | 497.70 | 0.562 | 0.849 | 0.641 | 0.613 | 0.599 | 0.582 |
| IOCTANE | NHTMVDHEPJAVLT-UHFFFAOYSA-N | 544.00 | 0.621 | 0.922 | 0.698 | 0.676 | 0.661 | 0.641 |
| IPENTANE | QWTDNUCVQCZILF-UHFFFAOYSA-N | 460.35 | 0.534 | 0.798 | 0.607 | 0.581 | 0.568 | 0.552 |
| ISOBUTAN | NNPPMTNAJDCUHE-UHFFFAOYSA-N | 407.81 | 0.507 | 0.754 | 0.573 | 0.553 | 0.540 | 0.525 |
| KRYPTON | DNNSSWSSYDEUBZ-UHFFFAOYSA-N | 209.48 | 0.385 | 0.535 | 0.412 | 0.393 | 0.384 | 0.372 |
| MD2M | YFCGDEUVHLPRCZ-UHFFFAOYSA-N | 599.40 | 0.818 | 1.243 | 0.925 | 0.917 | 0.896 | 0.870 |

Continued on next page...

Table S15 – continued from previous page

| Fluid | Standard InChI key | $T_c$/K | $v_{N,t}^{1/3}$/nm | $v_{N,crit}^{1/3}$/nm | $v_{N,0.8T_c}^{1/3}$/nm | $\sigma(T_c/1.32)$/nm | $\sigma(T_c/1.0)$/nm | $\sigma(T_c/0.7)$/nm |
|---|---|---|---|---|---|---|---|---|
| MD3M | FBZANXDWQAVSTQ-UHFFFAOYSA-N | 628.96 | 0.870 | 1.334 | 0.993 | 0.987 | 0.964 | 0.936 |
| MDM | CXQXSVUQTKDNFP-UHFFFAOYSA-N | 565.36 | 0.752 | 1.136 | 0.850 | 0.836 | 0.817 | 0.793 |
| MEA | HZAXFHJVJLSVMW-UHFFFAOYSA-N | 671.40 | 0.463 | 0.675 | 0.507 | 0.508 | 0.496 | 0.482 |
| METHANE | VNWKTOKETHGBQD-UHFFFAOYSA-N | 190.56 | 0.390 | 0.547 | 0.423 | 0.394 | 0.385 | 0.374 |
| METHANOL | OKKJLVBELUTLKV-UHFFFAOYSA-N | 513.38 | 0.389 | 0.574 | 0.431 | 0.421 | 0.411 | 0.399 |
| MM | UQEAIHBTYFGYIE-UHFFFAOYSA-N | 518.70 | 0.681 | 1.002 | 0.757 | 0.740 | 0.723 | 0.702 |
| MOLEATE | QYDYPVFESGNLHU-KHPPLWFESA-N | 782.00 | 0.817 | 1.269 | 0.926 | 0.911 | 0.890 | 0.864 |
| MSTEARAT | HPEUJPJOZXNMSJ-UHFFFAOYSA-N | 775.00 | 0.836 | 1.279 | 0.931 | 0.925 | 0.904 | 0.878 |
| MXYLENE | IVSZLXZYQVIEFR-UHFFFAOYSA-N | 616.89 | 0.577 | 0.854 | 0.642 | 0.607 | 0.594 | 0.576 |
| NEON | GKAOGPIIYCISHV-UHFFFAOYSA-N | 44.40 | 0.302 | 0.410 | 0.319 | 0.304 | 0.297 | 0.288 |
| NEOPENTN | CRSOQBOWXPBRES-UHFFFAOYSA-N | 433.74 | 0.576 | 0.798 | 0.611 | 0.607 | 0.593 | 0.576 |
| NITROGEN | IJGRMHOSHXDMSA-UHFFFAOYSA-N | 126.19 | 0.378 | 0.530 | 0.408 | 0.388 | 0.379 | 0.368 |
| NONANE | BKIMMITUMNQMOS-UHFFFAOYSA-N | 594.55 | 0.650 | 0.972 | 0.726 | 0.700 | 0.684 | 0.664 |
| OCTANE | TVMXDCGIABBOFY-UHFFFAOYSA-N | 568.74 | 0.629 | 0.935 | 0.700 | 0.674 | 0.659 | 0.639 |
| OXYGEN | MYMOFIZGZYHOMD-UHFFFAOYSA-N | 154.58 | 0.345 | 0.496 | 0.383 | 0.355 | 0.347 | 0.337 |
| OXYLENE | CTQNGGLPUBDAKN-UHFFFAOYSA-N | 630.26 | 0.577 | 0.852 | 0.639 | 0.609 | 0.595 | 0.578 |
| PENTANE | OFBQJSOFQDEBGM-UHFFFAOYSA-N | 469.70 | 0.540 | 0.803 | 0.608 | 0.584 | 0.571 | 0.554 |
| PROPANE | ATUOYWHBWRKTHZ-UHFFFAOYSA-N | 369.89 | 0.464 | 0.693 | 0.529 | 0.509 | 0.497 | 0.483 |
| PROPYLEN | QQONPFPTGQHPMA-UHFFFAOYSA-N | 364.21 | 0.450 | 0.673 | 0.513 | 0.486 | 0.475 | 0.461 |
| PROPYLENEOXIDE | GOOHAUXETOMSMM-UHFFFAOYSA-N | 488.11 | 0.461 | 0.685 | 0.519 | 0.493 | 0.481 | 0.467 |
| PXYLENE | URLKBWYHVLBVBO-UHFFFAOYSA-N | 616.17 | 0.588 | 0.851 | 0.643 | 0.609 | 0.595 | 0.577 |
| R11 | CYRMSUTZVYGINF-UHFFFAOYSA-N | 471.11 | 0.506 | 0.744 | 0.565 | 0.545 | 0.533 | 0.517 |
| R113 | AJDIZQLSFPQPEY-UHFFFAOYSA-N | 487.21 | 0.568 | 0.822 | 0.618 | 0.609 | 0.595 | 0.577 |
| R114 | DDMOUSALMHHKOS-UHFFFAOYSA-N | 418.83 | nan | 0.788 | 0.597 | 0.587 | 0.574 | 0.557 |
| R115 | RFCAUADVODFSLZ-UHFFFAOYSA-N | 353.10 | 0.528 | 0.747 | 0.574 | 0.567 | 0.554 | 0.538 |
| R12 | PXBRQCKWGAHEHS-UHFFFAOYSA-N | 385.12 | 0.479 | 0.708 | 0.540 | 0.522 | 0.510 | 0.495 |
| R123 | OHMHBGPWCHTMQE-UHFFFAOYSA-N | 456.83 | 0.524 | 0.773 | 0.584 | 0.568 | 0.555 | 0.539 |
| R1233ZDE | LDTMPQQAWUMPKS-OWOJBTEDSA-N | 439.60 | 0.527 | 0.767 | 0.578 | 0.577 | 0.564 | 0.547 |
| R1234YF | FXRLMCRCYDHQFW-UHFFFAOYSA-N | 367.85 | 0.496 | 0.736 | 0.555 | 0.538 | 0.525 | 0.510 |
| R1234ZEE | CDOOAUSHHFGWSA-OWOJBTEDSA-N | 382.51 | 0.501 | 0.729 | 0.550 | 0.536 | 0.524 | 0.508 |
| R124 | BOUGCJDAQLKBQH-UHFFFAOYSA-N | 395.43 | nan | 0.740 | 0.560 | 0.550 | 0.537 | 0.521 |
| R125 | GTLACDSXYULKMZ-UHFFFAOYSA-N | 339.17 | 0.491 | 0.703 | 0.531 | 0.525 | 0.513 | 0.498 |
| R13 | AFYPFACVUDMOHA-UHFFFAOYSA-N | 302.00 | 0.454 | 0.668 | 0.510 | 0.489 | 0.478 | 0.464 |
| R134A | LVGUZGTVOIAKKC-UHFFFAOYSA-N | 374.21 | 0.475 | 0.692 | 0.520 | 0.510 | 0.499 | 0.484 |
| R14 | TXEYQDLBPFQVAA-UHFFFAOYSA-N | 227.51 | nan | 0.616 | 0.473 | 0.460 | 0.450 | 0.437 |
| R141B | FRCHKSNAZZFGCA-UHFFFAOYSA-N | 477.50 | 0.510 | 0.751 | 0.570 | 0.550 | 0.537 | 0.522 |
| R142B | BHNZEZWIUMJCGF-UHFFFAOYSA-N | 410.26 | 0.487 | 0.721 | 0.545 | 0.526 | 0.514 | 0.499 |
| R143A | UJPMYEOUBPIPHQ-UHFFFAOYSA-N | 345.86 | 0.472 | 0.687 | 0.517 | 0.499 | 0.488 | 0.474 |
| R150 | WSLDOOZREJYCGB-UHFFFAOYSA-N | 561.60 | 0.498 | 0.727 | 0.550 | 0.528 | 0.516 | 0.501 |
| R152A | NPNPZTNLOVBDOC-UHFFFAOYSA-N | 386.41 | 0.452 | 0.668 | 0.501 | 0.482 | 0.471 | 0.457 |
| R161 | UHCBBWUQDAVSMS-UHFFFAOYSA-N | 375.25 | 0.437 | 0.642 | 0.487 | 0.463 | 0.452 | 0.439 |
| R21 | UMNKXPULIDJLSU-UHFFFAOYSA-N | 451.48 | nan | 0.687 | 0.523 | 0.500 | 0.488 | 0.474 |
| R218 | QYSGYZVSCZSLHT-UHFFFAOYSA-N | 345.02 | 0.538 | 0.792 | 0.601 | 0.602 | 0.588 | 0.571 |
| R22 | VOPWNXZWBYDODV-UHFFFAOYSA-N | 369.30 | 0.437 | 0.650 | 0.493 | 0.472 | 0.461 | 0.447 |
| R227EA | YFMFNYKEUDLDTL-UHFFFAOYSA-N | 374.90 | 0.532 | 0.780 | 0.589 | 0.587 | 0.574 | 0.557 |
| R23 | XPDWGBQVDMORPB-UHFFFAOYSA-N | 299.29 | 0.409 | 0.604 | 0.454 | 0.433 | 0.423 | 0.411 |
| R236EA | FYIRUPZTYPILDH-UHFFFAOYSA-N | 412.44 | nan | 0.765 | 0.577 | 0.574 | 0.561 | 0.545 |
| R236FA | NSGXIBWMJZWTPY-UHFFFAOYSA-N | 398.07 | 0.529 | 0.771 | 0.581 | 0.575 | 0.562 | 0.545 |
| R245CA | AWTOFSDLNREIFS-UHFFFAOYSA-N | 447.57 | 0.516 | 0.751 | 0.567 | 0.563 | 0.550 | 0.534 |

Continued on next page...

Table S15 – continued from previous page

| Fluid | Standard InChI key | $T_c$/K | $v_{N,t}^{1/3}$/nm | $v_{N,crit}^{1/3}$/nm | $v_{N,0.8T_c}^{1/3}$/nm | $\sigma(T_c/1.32)$/nm | $\sigma(T_c/1.0)$/nm | $\sigma(T_c/0.7)$/nm |
|---|---|---|---|---|---|---|---|---|
| R245FA | MSSNHSVIGIHOJA-UHFFFAOYSA-N | 427.01 | 0.514 | 0.754 | 0.569 | 0.563 | 0.551 | 0.534 |
| R32 | RWRIWBAIICGTTQ-UHFFFAOYSA-N | 351.25 | 0.393 | 0.588 | 0.438 | 0.415 | 0.405 | 0.393 |
| R365MFC | WZLFPVPRZGTCKP-UHFFFAOYSA-N | 460.00 | 0.564 | 0.804 | 0.609 | 0.602 | 0.588 | 0.571 |
| R40 | NEHMKBQYUWJMIP-UHFFFAOYSA-N | 416.30 | nan | 0.613 | 0.465 | 0.440 | 0.430 | 0.418 |
| RC318 | BCCOBQSFUDVTJQ-UHFFFAOYSA-N | 388.38 | 0.578 | 0.812 | 0.612 | 0.621 | 0.607 | 0.589 |
| RE245CB2 | GCDWNCOAODIANN-UHFFFAOYSA-N | 406.81 | 0.563 | 0.793 | 0.596 | 0.586 | 0.573 | 0.556 |
| RE245FA2 | ZASBKNPRLPFSCA-UHFFFAOYSA-N | 444.88 | 0.550 | 0.785 | 0.589 | 0.578 | 0.564 | 0.548 |
| RE347MCC | NOPJRYAFUXTDLX-UHFFFAOYSA-N | 437.70 | 0.572 | 0.857 | 0.643 | 0.637 | 0.622 | 0.604 |
| SF6 | SFZCNBIFKDRMGX-UHFFFAOYSA-N | 318.72 | 0.509 | 0.689 | 0.525 | 0.526 | 0.514 | 0.499 |
| SO2 | RAHZWNYVWXNFOC-UHFFFAOYSA-N | 430.64 | 0.403 | 0.590 | 0.443 | 0.421 | 0.412 | 0.399 |
| TOLUENE | YXFVVABEGXRONW-UHFFFAOYSA-N | 591.75 | 0.540 | 0.806 | 0.609 | 0.578 | 0.565 | 0.549 |
| WATER | XLYOFNOQVPJJNP-UHFFFAOYSA-N | 647.10 | 0.310 | 0.453 | 0.333 | 0.314 | 0.307 | 0.298 |
| XENON | FHNFHKCVQCLJFQ-UHFFFAOYSA-N | 289.73 | 0.420 | 0.583 | 0.448 | 0.423 | 0.413 | 0.401 |

### Table S16. Fitted values for $\sigma$ for the HS potential

| Fluid | Standard InChI key | $T_c$/K | $v_{N,t}^{1/3}$/nm | $v_{N,crit}^{1/3}$/nm | $v_{N,0.8T_c}^{1/3}$/nm | $\sigma(T_c/1.32)$/nm | $\sigma(T_c/1.0)$/nm | $\sigma(T_c/0.7)$/nm |
|---|---|---|---|---|---|---|---|---|
| 13BUTADIENE | KAKZBPTYRLMSJV-UHFFFAOYSA-N | 425.13 | 0.490 | 0.716 | 0.544 | 0.479 | 0.479 | 0.479 |
| 22DIMETHYLBUTANE | HNRMPXKDFBEGFZ-UHFFFAOYSA-N | 490.00 | 0.575 | 0.842 | 0.641 | 0.587 | 0.587 | 0.587 |
| 23DIMETHYLBUTANE | ZFFMLCVRJBZUDZ-UHFFFAOYSA-N | 500.60 | 0.567 | 0.840 | 0.638 | 0.580 | 0.580 | 0.580 |
| 3METHYLPENTANE | PFEOZHBOMNWTJB-UHFFFAOYSA-N | 506.00 | 0.557 | 0.842 | 0.639 | 0.577 | 0.577 | 0.577 |
| ACETONE | CSCPPACGZOOCGX-UHFFFAOYSA-N | 508.10 | 0.473 | 0.707 | 0.530 | 0.475 | 0.475 | 0.475 |
| AMMONIA | QGZKDVFQNNGYKY-UHFFFAOYSA-N | 405.56 | 0.338 | 0.495 | 0.369 | 0.316 | 0.316 | 0.316 |
| ARGON | XKRFYHLGVUSROY-UHFFFAOYSA-N | 150.69 | 0.361 | 0.498 | 0.385 | 0.328 | 0.328 | 0.328 |
| BENZENE | UHOVQNZJYSORNB-UHFFFAOYSA-N | 562.02 | 0.526 | 0.752 | 0.572 | 0.518 | 0.518 | 0.518 |
| BUTANE | IJDNQMDRQITEOD-UHFFFAOYSA-N | 425.12 | 0.509 | 0.751 | 0.571 | 0.507 | 0.507 | 0.507 |
| C11 | RSJKGSCJYJTIGS-UHFFFAOYSA-N | 638.80 | 0.695 | 1.031 | 0.775 | 0.708 | 0.708 | 0.708 |
| C12 | SNRUBQQJIBEYMU-UHFFFAOYSA-N | 658.10 | 0.716 | 1.077 | 0.798 | 0.730 | 0.730 | 0.730 |
| C16 | DCAYPVUWAIABOU-UHFFFAOYSA-N | 722.10 | 0.786 | 1.184 | 0.876 | 0.807 | 0.807 | 0.807 |
| C1CC6 | UAEPNZWRGJTJPN-UHFFFAOYSA-N | 572.20 | 0.567 | 0.848 | 0.645 | 0.591 | 0.591 | 0.591 |
| C22 | HOWGUJZVBDQJKV-UHFFFAOYSA-N | 792.20 | 0.872 | 1.319 | 0.975 | 0.906 | 0.906 | 0.906 |
| C3CC6 | DEDZSLCZHWTGOR-UHFFFAOYSA-N | 630.80 | 0.619 | 0.931 | 0.702 | 0.641 | 0.641 | 0.641 |
| C5F12 | NJCBUSHGCBERSK-UHFFFAOYSA-N | 421.00 | 0.616 | 0.915 | 0.688 | 0.644 | 0.644 | 0.644 |
| C6F14 | ZJIJAJXFLBMLCK-UHFFFAOYSA-N | 448.00 | 0.657 | 0.969 | 0.723 | 0.680 | 0.680 | 0.680 |
| CF3I | VPAYJEUHKVESSD-UHFFFAOYSA-N | 396.44 | 0.509 | 0.721 | 0.552 | 0.501 | 0.501 | 0.501 |
| CHLORINE | KZBUYRJDOAKODT-UHFFFAOYSA-N | 416.87 | 0.408 | 0.591 | 0.452 | 0.405 | 0.405 | 0.405 |
| CHLOROBENZENE | MVPPADPHJFYWMZ-UHFFFAOYSA-N | 632.35 | 0.542 | 0.800 | 0.604 | 0.545 | 0.545 | 0.545 |
| CO | UGFAIRIUMAVXCW-UHFFFAOYSA-N | 132.86 | 0.381 | 0.535 | 0.411 | 0.370 | 0.370 | 0.370 |
| CO2 | CURLTUGMZLYLDI-UHFFFAOYSA-N | 304.13 | 0.397 | 0.539 | 0.408 | 0.360 | 0.360 | 0.360 |
| CYCLOHEX | XDTMQSROBMDMFD-UHFFFAOYSA-N | 553.60 | 0.562 | 0.802 | 0.609 | 0.562 | 0.562 | 0.562 |
| CYCLOPEN | RGSFGYAAUTVSQA-UHFFFAOYSA-N | 511.72 | 0.516 | 0.751 | 0.575 | 0.524 | 0.524 | 0.524 |
| D2 | UFHFLCQGNIYNRP-VVKOMZTBSA-N | 38.34 | 0.340 | 0.458 | 0.362 | 0.320 | 0.320 | 0.320 |
| D2O | XLYOFNOQVPJJNP-ZSJDYOACSA-N | 643.85 | 0.311 | 0.454 | 0.333 | 0.301 | 0.301 | 0.301 |
| D4 | HMMGMWAXVFQUOA-UHFFFAOYSA-N | 586.50 | 0.801 | 1.168 | 0.875 | 0.820 | 0.820 | 0.820 |
| D5 | XMSXQFUHVRWGNA-UHFFFAOYSA-N | 618.30 | 0.843 | 1.265 | 0.947 | 0.894 | 0.894 | 0.894 |
| D6 | IUMSDRXLFWAGNT-UHFFFAOYSA-N | 645.78 | 0.905 | 1.383 | 1.015 | 0.958 | 0.958 | 0.958 |
| DEA | ZBCBWPMODOFKDW-UHFFFAOYSA-N | 736.50 | 0.543 | 0.795 | 0.589 | 0.594 | 0.594 | 0.594 |
| DECANE | DIOQZVSQGTUSAI-UHFFFAOYSA-N | 617.70 | 0.675 | 1.004 | 0.751 | 0.685 | 0.685 | 0.685 |
| DEE | RTZKZFJDLAIYFH-UHFFFAOYSA-N | 466.70 | nan | 0.775 | 0.587 | 0.526 | 0.526 | 0.526 |
| DMC | IEJIGPNLZYLLBP-UHFFFAOYSA-N | 557.00 | 0.516 | 0.746 | 0.562 | 0.507 | 0.507 | 0.507 |
| DME | LCGLNKUTAGEVQW-UHFFFAOYSA-N | 400.38 | 0.443 | 0.654 | 0.497 | 0.435 | 0.435 | 0.435 |
| EBENZENE | YNQLUTRBYVCPMQ-UHFFFAOYSA-N | 617.12 | 0.567 | 0.846 | 0.642 | 0.579 | 0.579 | 0.579 |
| EGLYCOL | LYCAIKOWRPUZTN-UHFFFAOYSA-N | 719.00 | 0.450 | 0.656 | 0.492 | 0.477 | 0.477 | 0.477 |
| ETHANE | OTMSDBZUPAUEDD-UHFFFAOYSA-N | 305.32 | 0.425 | 0.623 | 0.478 | 0.406 | 0.406 | 0.406 |
| ETHANOL | LFQSCWFLJHTTHZ-UHFFFAOYSA-N | 514.71 | 0.439 | 0.654 | 0.486 | 0.459 | 0.459 | 0.459 |
| ETHYLENE | VGGSQFUCUMXWEO-UHFFFAOYSA-N | 282.35 | 0.415 | 0.601 | 0.461 | 0.412 | 0.412 | 0.412 |
| ETHYLENEOXIDE | IAYPIBMASNFSPL-UHFFFAOYSA-N | 468.92 | 0.413 | 0.614 | 0.463 | 0.413 | 0.413 | 0.413 |
| FLUORINE | PXGOKWXKJXAPGV-UHFFFAOYSA-N | 144.41 | 0.334 | 0.474 | 0.369 | 0.331 | 0.331 | 0.331 |
| H2S | RWSOTUBLDIXVET-UHFFFAOYSA-N | 373.10 | 0.385 | 0.546 | 0.418 | 0.363 | 0.363 | 0.363 |
| HCL | VEXZGXHMUGYJMC-UHFFFAOYSA-N | 324.68 | 0.365 | 0.519 | 0.396 | 0.341 | 0.341 | 0.341 |
| HEPTANE | IMNFDUFMRHMDMM-UHFFFAOYSA-N | 540.20 | 0.599 | 0.893 | 0.672 | 0.609 | 0.609 | 0.609 |
| HEXANE | VLKZOEOYAKHREP-UHFFFAOYSA-N | 507.82 | 0.574 | 0.850 | 0.641 | 0.579 | 0.579 | 0.579 |
| HYDROGEN | UFHFLCQGNIYNRP-UHFFFAOYSA-N | 33.15 | 0.354 | 0.475 | 0.378 | 0.327 | 0.327 | 0.327 |
| IBUTENE | VQTUBCCKSQIDNK-UHFFFAOYSA-N | 418.09 | 0.496 | 0.736 | 0.557 | 0.499 | 0.499 | 0.499 |
| IHEXANE | AFABGHUZZDYHJO-UHFFFAOYSA-N | 497.70 | 0.562 | 0.849 | 0.641 | 0.580 | 0.580 | 0.580 |
| IOCTANE | NHTMVDHEPJAVLT-UHFFFAOYSA-N | 544.00 | 0.621 | 0.922 | 0.698 | 0.638 | 0.638 | 0.638 |

Continued on next page...

Table S16 – continued from previous page

| Fluid | Standard InChI key | $T_c$/K | $v_{N,t}^{1/3}$/nm | $v_{N,crit}^{1/3}$/nm | $v_{N,0.8T_c}^{1/3}$/nm | $\sigma(T_c/1.32)$/nm | $\sigma(T_c/1.0)$/nm | $\sigma(T_c/0.7)$/nm |
|---|---|---|---|---|---|---|---|---|
| IPENTANE | QWTDNUCVQCZILF-UHFFFAOYSA-N | 460.35 | 0.534 | 0.798 | 0.607 | 0.549 | 0.549 | 0.549 |
| ISOBUTAN | NNPPMTNAJDCUHE-UHFFFAOYSA-N | 407.81 | 0.507 | 0.754 | 0.573 | 0.522 | 0.522 | 0.522 |
| KRYPTON | DNNSSWSSYDEUBZ-UHFFFAOYSA-N | 209.48 | 0.385 | 0.535 | 0.412 | 0.345 | 0.345 | 0.345 |
| MD2M | YFCGDEUVHLPRCZ-UHFFFAOYSA-N | 599.40 | 0.818 | 1.243 | 0.925 | 0.857 | 0.857 | 0.857 |
| MD3M | FBZANXDWQAVSTQ-UHFFFAOYSA-N | 628.96 | 0.870 | 1.334 | 0.993 | 0.919 | 0.919 | 0.919 |
| MD4M | ADANNTOYRVPQLJ-UHFFFAOYSA-N | 653.20 | 0.924 | 1.428 | 1.054 | 0.975 | 0.975 | 0.975 |
| MDM | CXQXSVUQTKDNFP-UHFFFAOYSA-N | 565.36 | 0.752 | 1.136 | 0.850 | 0.783 | 0.783 | 0.783 |
| MEA | HZAXFHJVJLSVMW-UHFFFAOYSA-N | 671.40 | 0.463 | 0.675 | 0.507 | 0.490 | 0.490 | 0.490 |
| METHANE | VNWKTOKETHGBQD-UHFFFAOYSA-N | 190.56 | 0.390 | 0.547 | 0.423 | 0.351 | 0.351 | 0.351 |
| METHANOL | OKKJLVBELUTLKV-UHFFFAOYSA-N | 513.38 | 0.389 | 0.574 | 0.431 | 0.397 | 0.397 | 0.397 |
| MLINOLEA | WTTJVINHCBCLGX-NQLNTKRDSA-N | 799.00 | 0.808 | 1.271 | 0.918 | 0.853 | 0.853 | 0.853 |
| MLINOLEN | DVWSXZIHSUZZKJ-YSTUJMKBSA-N | 772.00 | nan | 1.251 | 0.905 | 0.843 | 0.843 | 0.843 |
| MM | UQEAIHBTYFGYIE-UHFFFAOYSA-N | 518.70 | 0.681 | 1.002 | 0.757 | 0.696 | 0.696 | 0.696 |
| MOLEATE | QYDYPVFESGNLHU-KHPPLWFESA-N | 782.00 | 0.817 | 1.269 | 0.926 | 0.863 | 0.863 | 0.863 |
| MPALMITA | FLIACVVOZYBSBS-UHFFFAOYSA-N | 755.00 | nan | 1.228 | 0.895 | 0.833 | 0.833 | 0.833 |
| MSTEARAT | HPEUJPJOZXNMSJ-UHFFFAOYSA-N | 775.00 | 0.836 | 1.279 | 0.931 | 0.866 | 0.866 | 0.866 |
| MXYLENE | IVSZLXZYQVIEFR-UHFFFAOYSA-N | 616.89 | 0.577 | 0.854 | 0.642 | 0.577 | 0.577 | 0.577 |
| N2O | GQPLMRYTRLFLPF-UHFFFAOYSA-N | 309.52 | 0.390 | 0.545 | 0.415 | 0.405 | 0.405 | 0.405 |
| NEON | GKAOGPIIYCISHV-UHFFFAOYSA-N | 44.40 | 0.302 | 0.410 | 0.319 | 0.282 | 0.282 | 0.282 |
| NEOPENTN | CRSOQBOWXPBRES-UHFFFAOYSA-N | 433.74 | 0.576 | 0.798 | 0.611 | 0.560 | 0.560 | 0.560 |
| NITROGEN | IJGRMHOSHXDMSA-UHFFFAOYSA-N | 126.19 | 0.378 | 0.530 | 0.408 | 0.358 | 0.358 | 0.358 |
| NONANE | BKIMMITUMNQMOS-UHFFFAOYSA-N | 594.55 | 0.650 | 0.972 | 0.726 | 0.661 | 0.661 | 0.661 |
| OCTANE | TVMXDCGIABBOFY-UHFFFAOYSA-N | 568.74 | 0.629 | 0.935 | 0.700 | 0.634 | 0.634 | 0.634 |
| OXYGEN | MYMOFIZGZYHOMD-UHFFFAOYSA-N | 154.58 | 0.345 | 0.496 | 0.383 | 0.341 | 0.341 | 0.341 |
| OXYLENE | CTQNGGLPUBDAKN-UHFFFAOYSA-N | 630.26 | 0.577 | 0.852 | 0.639 | 0.579 | 0.579 | 0.579 |
| PENTANE | OFBQJSOFQDEBGM-UHFFFAOYSA-N | 469.70 | 0.540 | 0.803 | 0.608 | 0.544 | 0.544 | 0.544 |
| PROPANE | ATUOYWHBWRKTHZ-UHFFFAOYSA-N | 369.89 | 0.464 | 0.693 | 0.529 | 0.464 | 0.464 | 0.464 |
| PROPYLEN | QQONPFPTGQHPMA-UHFFFAOYSA-N | 364.21 | 0.450 | 0.673 | 0.513 | 0.451 | 0.451 | 0.451 |
| PROPYLENEOXIDE | GOOHAUXETOMSMM-UHFFFAOYSA-N | 488.11 | 0.461 | 0.685 | 0.519 | 0.467 | 0.467 | 0.467 |
| PXYLENE | URLKBWYHVLBVBO-UHFFFAOYSA-N | 616.17 | 0.588 | 0.851 | 0.643 | 0.580 | 0.580 | 0.580 |
| R11 | CYRMSUTZVYGINF-UHFFFAOYSA-N | 471.11 | 0.506 | 0.744 | 0.565 | 0.510 | 0.510 | 0.510 |
| R113 | AJDIZQLSFPQPEY-UHFFFAOYSA-N | 487.21 | 0.568 | 0.822 | 0.618 | 0.570 | 0.570 | 0.570 |
| R114 | DDMOUSALMHHKOS-UHFFFAOYSA-N | 418.83 | nan | 0.788 | 0.597 | 0.549 | 0.549 | 0.549 |
| R115 | RFCAUADVODFSLZ-UHFFFAOYSA-N | 353.10 | 0.528 | 0.747 | 0.574 | 0.528 | 0.528 | 0.528 |
| R12 | PXBRQCKWGAHEHS-UHFFFAOYSA-N | 385.12 | 0.479 | 0.708 | 0.540 | 0.481 | 0.481 | 0.481 |
| R123 | OHMHBGPWCHTMQE-UHFFFAOYSA-N | 456.83 | 0.524 | 0.773 | 0.584 | 0.534 | 0.534 | 0.534 |
| R1233ZDE | LDTMPQQAWUMPKS-OWOJBTEDSA-N | 439.60 | 0.527 | 0.767 | 0.578 | 0.537 | 0.537 | 0.537 |
| R1234YF | FXRLMCRCYDHQFW-UHFFFAOYSA-N | 367.85 | 0.496 | 0.736 | 0.555 | 0.498 | 0.498 | 0.498 |
| R1234ZEE | CDOOAUSHHFGWSA-OWOJBTEDSA-N | 382.51 | 0.501 | 0.729 | 0.550 | 0.496 | 0.496 | 0.496 |
| R124 | BOUGCJDAQLKBQH-UHFFFAOYSA-N | 395.43 | nan | 0.740 | 0.560 | 0.512 | 0.512 | 0.512 |
| R125 | GTLACDSXYULKMZ-UHFFFAOYSA-N | 339.17 | 0.491 | 0.703 | 0.531 | 0.486 | 0.486 | 0.486 |
| R13 | AFYPFACVUDMOHA-UHFFFAOYSA-N | 302.00 | 0.454 | 0.668 | 0.510 | 0.459 | 0.459 | 0.459 |
| R134A | LVGUZGTVOIAKKC-UHFFFAOYSA-N | 374.21 | 0.475 | 0.692 | 0.520 | 0.473 | 0.473 | 0.473 |
| R14 | TXEYQDLBPFQVAA-UHFFFAOYSA-N | 227.51 | nan | 0.616 | 0.473 | 0.390 | 0.390 | 0.390 |
| R141B | FRCHKSNAZZFGCA-UHFFFAOYSA-N | 477.50 | 0.510 | 0.751 | 0.570 | 0.519 | 0.519 | 0.519 |
| R142B | BHNZEZWIUMJCGF-UHFFFAOYSA-N | 410.26 | 0.487 | 0.721 | 0.545 | 0.492 | 0.492 | 0.492 |
| R143A | UJPMYEOUBPIPHQ-UHFFFAOYSA-N | 345.86 | 0.472 | 0.687 | 0.517 | 0.463 | 0.463 | 0.463 |
| R150 | WSLDOOZREJYCGB-UHFFFAOYSA-N | 561.60 | 0.498 | 0.727 | 0.550 | 0.500 | 0.500 | 0.500 |
| R152A | NPNPZTNLOVBDOC-UHFFFAOYSA-N | 386.41 | 0.452 | 0.668 | 0.501 | 0.448 | 0.448 | 0.448 |

Continued on next page...

Table S16 – continued from previous page

| Fluid | Standard InChI key | $T_c$/K | $v_{N,t}^{1/3}$/nm | $v_{N,crit}^{1/3}$/nm | $v_{N,0.8T_c}^{1/3}$/nm | $\sigma(T_c/1.32)$/nm | $\sigma(T_c/1.0)$/nm | $\sigma(T_c/0.7)$/nm |
|---|---|---|---|---|---|---|---|---|
| R161 | UHCBBWUQDAVSMS-UHFFFAOYSA-N | 375.25 | 0.437 | 0.642 | 0.487 | 0.427 | 0.427 | 0.427 |
| R21 | UMNKXPULIDJLSU-UHFFFAOYSA-N | 451.48 | nan | 0.687 | 0.523 | 0.468 | 0.468 | 0.468 |
| R218 | QYSGYZVSCZSLHT-UHFFFAOYSA-N | 345.02 | 0.538 | 0.792 | 0.601 | 0.556 | 0.556 | 0.556 |
| R22 | VOPWNXZWBYDODV-UHFFFAOYSA-N | 369.30 | 0.437 | 0.650 | 0.493 | 0.441 | 0.441 | 0.441 |
| R227EA | YFMFNYKEUDLDTL-UHFFFAOYSA-N | 374.90 | 0.532 | 0.780 | 0.589 | 0.544 | 0.544 | 0.544 |
| R23 | XPDWGBQVDMORPB-UHFFFAOYSA-N | 299.29 | 0.409 | 0.604 | 0.454 | 0.400 | 0.400 | 0.400 |
| R236EA | FYIRUPZTYPILDH-UHFFFAOYSA-N | 412.44 | nan | 0.765 | 0.577 | 0.536 | 0.536 | 0.536 |
| R236FA | NSGXIBWMJZWTPY-UHFFFAOYSA-N | 398.07 | 0.529 | 0.771 | 0.581 | 0.534 | 0.534 | 0.534 |
| R245CA | AWTOFSDLNREIFS-UHFFFAOYSA-N | 447.57 | 0.516 | 0.751 | 0.567 | 0.527 | 0.527 | 0.527 |
| R245FA | MSSNHSVIGIHOJA-UHFFFAOYSA-N | 427.01 | 0.514 | 0.754 | 0.569 | 0.526 | 0.526 | 0.526 |
| R32 | RWRIWBAIICGTTQ-UHFFFAOYSA-N | 351.25 | 0.393 | 0.588 | 0.438 | 0.383 | 0.383 | 0.383 |
| R365MFC | WZLFPVPRZGTCKP-UHFFFAOYSA-N | 460.00 | 0.564 | 0.804 | 0.609 | 0.563 | 0.563 | 0.563 |
| R40 | NEHMKBQYUWJMIP-UHFFFAOYSA-N | 416.30 | nan | 0.613 | 0.465 | 0.408 | 0.408 | 0.408 |
| RC318 | BCCOBQSFUDVTJQ-UHFFFAOYSA-N | 388.38 | 0.578 | 0.812 | 0.612 | 0.574 | 0.574 | 0.574 |
| RE245CB2 | GCDWNCOAODIANN-UHFFFAOYSA-N | 406.81 | 0.563 | 0.793 | 0.596 | 0.544 | 0.544 | 0.544 |
| RE245FA2 | ZASBKNPRLPFSCA-UHFFFAOYSA-N | 444.88 | 0.550 | 0.785 | 0.589 | 0.542 | 0.542 | 0.542 |
| RE347MCC | NOPJRYAFUXTDLX-UHFFFAOYSA-N | 437.70 | 0.572 | 0.857 | 0.643 | 0.593 | 0.593 | 0.593 |
| SF6 | SFZCNBIFKDRMGX-UHFFFAOYSA-N | 318.72 | 0.509 | 0.689 | 0.525 | 0.479 | 0.479 | 0.479 |
| SO2 | RAHZWNYVWXNFOC-UHFFFAOYSA-N | 430.64 | 0.403 | 0.590 | 0.443 | 0.397 | 0.397 | 0.397 |
| TOLUENE | YXFVVABEGXRONW-UHFFFAOYSA-N | 591.75 | 0.540 | 0.806 | 0.609 | 0.550 | 0.550 | 0.550 |
| WATER | XLYOFNOQVPJJNP-UHFFFAOYSA-N | 647.10 | 0.310 | 0.453 | 0.333 | 0.302 | 0.302 | 0.302 |
| XENON | FHNFHKCVQCLJFQ-UHFFFAOYSA-N | 289.73 | 0.420 | 0.583 | 0.448 | 0.394 | 0.394 | 0.394 |

## References


1. Mohr PJ, Newell DB, Taylor BN (2016) CODATA recommended values of the fundamental physical constants: 2014. *J. Phys. Chem. Ref. Data* 45(4):043102.
2. Span R, Wagner W (1996) A New Equation of State for Carbon Dioxide Covering the Fluid Region from the Triple Point Temperature to 1100 K at Pressures up to 800 MPa. *J. Phys. Chem. Ref. Data* 25:1509–1596.
3. Giordano VM, Datchi F, Dewaele A (2006) Melting curve and fluid equation of state of carbon dioxide at high pressure and high temperature. *J. Chem. Phys.* 125(5):054504.
4. Abramson EH (2009) Viscosity of carbon dioxide measured to a pressure of 8 GPa and temperature of 673 K. *Physical Review E* 80(2):021201. 2009/08/19/.
5. Tegeler C, Span R, Wagner W (1999) A New Equation of State for Argon Covering the Fluid Region for Temperatures From the Melting Line to 700 K at Pressures up to 1000 MPa. *J. Phys. Chem. Ref. Data* 28:779–850.
6. Hunter JD (2007) Matplotlib: A 2D graphics environment. *Computing In Science & Engineering* 9(3):90–95.
7. Michels A, Botzen A, Schuurman W (1954) The viscosity of argon at pressures up to 2000 atmospheres. *Physica (Amsterdam)* 20:1141–8.
8. Kestin J, Whitelaw JH (1963) A Relative Determination of the Viscosity of Several Gases by the Oscillating Disk Method. *Physica A* 29:335–356.
9. Gracki JA, Flynn GP, Ross J (1969) Viscosity of nitrogen, helium, hydrogen, and argon from -100 to 25 řC up to 150-250 atm. *J. Chem. Phys.* 51(9):3856–63.
10. Kestin J, Paykoc E, Sengers JV (1971) Viscosity of helium, argon, and nitrogen as a function of density.
11. Haynes WM (1973) Viscosity of Gaseous and Liquid Argon. *Physica* 67(3):440–470.
12. Vermesse J, Vidal D (1973) Measurement of the viscosity coefficient of argon at high pressure (in French). *C. R. Hebd. Seances Acad. Sci.* Ser. B:277(9.
13. Trappeniers NJ, van der Gulik PS, van den Hooff H (1980) The Viscosity of Argon at Very High Pressure, up to the Melting Line. *Chemical Physics Letters* 70(3):438–443.
14. van der Gulik PS, Trappeniers NJ (1986) The viscosity of argon at high densities. *Physica* 135A:1–20.
15. Mostert R, van der Gulik PS, van den Berg HR (1989) Comment on the Experimental Viscosity of Argon at High Densities. *Physica A* 156:921–923.
16. Abramson EH (2011) Viscosity of argon to 5 GPa and 673 K. *High Pressure Research* 31(4):544–548. ISI:000299475400003.
17. Ross IF, Brown GM (1957) Viscosities of gases at high pressures. *Ind. Eng. Chem.* 49:2026.
18. Baron JD, Roof JG, Wells FW (1959) Viscosity of nitrogen, methane, ethane, and propane at elevated temperature and pressure. *J. Chem. Eng. Data* 4:283–288.
19. Carmichael LT, Berry VM, Sage BH (1965) Viscosity of Hydrocarbons. Methane. *J. Chem. Eng. Data* 10:57–61.
20. Haynes WM (1973) Viscosity of saturated liquid methane. *Physica (Amsterdam)* 70(2):410–412.
21. Chuang Sy, Chappelear PS, Kobayashi R (1976) Viscosity of Methane, Hydrogen, and Four Mixtures of Methane and Hydrogen from -100 C to 0 C at High Pressures. *J. Chem. Eng. Data* 21:403–411.
22. Diller DE (1980) Measurements of the viscosity of compressed gaseous and liquid methane. *Physica A (Amsterdam)* 104(3):417–426.
23. Huang ETS, Swift GW, Kurata F (1966) Viscosities of methane and propane at low temperatures and high pressures. *AIChE J.* 12:932–936.
24. van der Gulik PS, Mostert R, van den Berg HR (1988) The viscosity of methane at 25řC up to 10 kilobars. *Physica A (Amsterdam)* 151:153.
25. van der Gulik PS, Mostert R, van den Berg HR (1992) The viscosity of methane at 273 K up to 1 GPa. *Fluid Phase Equilib.* 79:301–311.
26. Evers C, Loesch HW, Wagner W (2002) An absolute viscometer-densimeter and measurements of the viscosity of nitrogen, methane, helium, neon, argon, and krypton over a wide range of density and temperature. *Int. J. Thermophys.* 23:1411–1439.
27. Hurly JJ, Gillis KA, Mehl JB, Moldover MR (2003) The Viscosity of Seven Gases Measured with a Greenspan Viscometer. *Int. J. Thermophys.* 24:1441–1474.
28. Abramson EH (2011) Viscosity of methane to 6 GPa and 673 K. *Phys. Rev. E* 84:062201.
29. Golubev IF (1970) *Viscosity of gases and gas mixtures. A handbook.* (Jerusalem), p. 245.
30. Michels A, Botzen A, Schuurman W (1957) The viscosity of carbon dioxide between 0 řC and 75 řC and at pressures up to 2000 atmospheres. *Physica (Amsterdam)* 23:95–102.
31. Kestin J, Whitelaw JH (1963) A relative determination of the viscosity of several gases by the oscillating disk method. *Physica (Amsterdam)* 29:335–356.
32. Golubev IF, Gnezdilov NE, Brodskoya GV (1971) The viscosity of air and carbon dioxide at various temperatures and pressures (in Russian). *Kimiya i teknologiya organicheska sinteza, ONTl, GIAP, part 8* pp. 48–53.
33. Golubev IF, Shepeleva RI (1971) The viscosity of liquid carbon dioxide at temperatures from -30,0 to +20,0ř C and pressures from 40 to 500 kg/cm2 (in Russian). *Kimiya i teknologiya organicheska sinteza, ONTI, GIAP, Part 8* pp. 44–47.
34. Haepp HJ (1976) Messung der Viskosität von Kohlendioxid und Propylen. *Wärme- und Stoffübertragung* 9(4):281–290.

http://dx.doi.org/10.1007/BF01003580.
35. Vogel E, Barkow L (1986) Precision Measurements of the Viscosity Coefficient of Carbon Dioxide between Room Temperature and 650 K. *Zeitschrift für Physikalische Chemie, Leipzig* 267(5):1038–1043.
36. Hendl S, Neumann AK, Vogel E (1993) The viscosity of carbon dioxide and its initial density dependence. *High Temperatures - High Pressures* 25(5):503–511. The viscosity of carbon dioxide and its initial density dependence.
37. Docter A, Lösch HW, Wagner W (1997) *Entwicklung und Aufbau einer Anlage zur simultanen Messung der Viskosität und der Dichte fluider Stoffe.* (VDI-Verlag GmbH, Düsseldorf, FRG) Vol. 3, No. 494, p. 150.
38. van der Gulik PS (1997) Viscosity of carbon dioxide in the liquid phase. *Physica A* 238:81–112.
39. Estrada-Alexanders AF, Hurly JJ (2008) Kinematic viscosity and speed of sound in gaseous CO, CO2, SiF4, SF6, C4F8, and NH3 from 220 K to 375 K and pressures up to 3.4 MPa. *Journal of Chemical Thermodynamics* 40(2):193–202.
40. Schäfer M, Richter M, Span R (2015) Measurements of the Viscosity of Carbon Dioxide at Temperatures from 253.15 K to 473.15 K with Pressures up to 1.2 MPa. *Journal of Chemical Thermodynamics.*
41. Kestin J, Ro ST, Wakeham WA (1971) Reference Values of the Viscosity of Twelve Gases at 25řC. *Transactions of the Faraday Society* 67:2308.
42. Ueda K, Kigoshi K (1974) The Viscosity of the Gaseous Hexafluorides of Sulfur, Selenium and Tellurium. *J. Inorg. Nucl. Chem.* 36(5):989–992.
43. Timrot DL, Serednitskaya MA, Traktueva SA (1975) Investigation of the Viscosity of Sulfur Hexafluoride by the Method of an Oscillating Disk (in Russian). *Teplofizika Vysokikh Temperatur* 13(5):1112–1116.
44. Grigorev BA, Keramidi AS, Grachev VK, Rastorguev YL (1977) An Experimental Investigation of the Viscosity of Sulphur Hexafluoride. *Teploenergetika (Moscow)* 24(9):85–.
45. Kestin J, Khalifa HE, Ro ST, Wakeham WA (1977) The viscosity and diffusion coefficients of eighteen binary gaseous systems. *Physica 88A* pp. 242–260.
46. Ulybin SA, Makarushkin VI (1977) Viscosity of Sulfur Hexafluoride at Temperatures of 230-800řK and Pressures up to 5ů108 dyn/cm2. *Teplofizika Vysokikh Temperatur* 15(6):1195–1201.
47. Hoogland JHB, Trappeniers NJ (1982) The Coefficient of Viscosity of Sulfur Hexafluoride along the Critical Isochore. *Proc. Symp. Thermophys.* 8:440–442.
48. Hoogland JHB, van den Berg HR, Trappeniers NJ (1985) Measurements of the viscosity of sulphur hexafluoride up to 100 bar by a capillary-flow viscometer. *Physica A* 134:169–192.
49. Takahashi M, Yokoyama C, Takahashi S (1987) Viscosity of Saturated Vapor of Inorganic Liquefied Gases in *The Eighth Japan Symposium on Thermophysical Properties.*
50. Strehlow T, Vogel E (1989) Temperature Dependence and Initial Density Dependence of the Viscosity of Sulphur Hexafluoride. *Physica A* 161:101–117.
51. Hurly JJ, Gillis KA, Mehl JB, Moldover MR (2003) The Viscosity of Seven Gases Measured with a Greenspan Viscometer. *International Journal of Thermophysics.*
52. Wilhelm J, Seibt D, Bich E, Vogel E, Hassel E (2005) Viscosity Measurements on Gaseous Sulfur Hexafluoride. *Journal of Chemical and Engineering Data* 50(3):896–906. file://localhost/Arno/Data
53. Estrada-Alexanders AF, Hurly JJ (2008) Kinematic viscosity and speed of sound in gaseous CO, CO2, SiF4, SF6, C4F8, and NH3 from 220 K to 375 K and pressures up to 3.4 MPa. *Journal of Chemical Thermodynamics* 40(2):193–202.
54. Ruvinski GY, Lavrenchenko GK, Ilyushenko SV (1990) Thermophysical Properties of R134a. *Kholodilnaja Tekhnika* (7):20–26.
55. Kumagai A, Takahashi S (1991) Viscosity of Saturated Liquid Fluorocarbon Refrigerants from 273 to 353 K. *International Journal of Thermophysics* 12(1):105–117.
56. Okubo T, Hasuo T, Nagashima A (1992) Measurement of the Viscosity of HFC 134a in the Temperature Range 213-423 K and at Pressures up to 30 MPa. *International Journal of Thermophysics* 13(6):931–942.
57. Diller DE, Aragon AS, Laesecke A (1993) Measurements of the Viscosities of Saturated and Compressed Liquid 1,1,1,2-tetrafluoroethane (R134a), 2,2-dichloro-1,1,1-trifluoroethane (R123) and 1,1-dichloro-1-fluoroethane (R141b). *Fluid Phase Equilibria* 88:251–262.
58. Assael MJ, Dymond JH, Polimatidou SK (1994) Measurements of the Viscosity of R134a and R32 in the Temperature Range 270-340K at Pressures up to 20 MPa. *International Journal of Thermophysics* 15(4):591–601.
59. Pasekov MF, Ustyuzhanin EE (1994) The Viscosity of R134a Refrigerant in the Gas Phase. *High Temperature* 32(4):591–594.
60. Assael MJ, Papadopoulos AA, Polimatidou S (1995) Measurements of the Viscosity of Refrigerants in the Vapour Phase in *4th Asian Thermophysical Properties Conference.* (Tokyo, Japan), pp. 623–626.
61. NRC-CNRC EM (1995).
62. Assael MJ, Polimatidou S (1996) Measurements of the Viscosity of Refrigerants in the Vapour Phase. *International Journal of Thermophysics* in press.
63. Oliveira CMBP, Fenghour A (1996).
64. Shibasaki-Kitagawa N, Takahashi M, Yokoyama C (1998) Viscosity of Gaseous HFC-134a (1,1,1,2-Tetrafluoroethane) Under High Pressures. *International Journal of Thermophysics* 19(5):1285–1295.
65. Laesecke A, Lüddecke TOD, Hafer RF, Morris DJ (1999) Viscosity Measurements of Ammonia, R32, and R134a. Vapor Buoyancy and Radial Acceleration in Capillary Viscometers. *International Journal of Thermophysics* 20(2):401–434.

66. Comuñas MJP, et al. (2003) Viscosity Measurements and Correlations for 1,1,1,2-tetrafluoroethane (HFC-134a) up to 140 MPa. *Fluid Phase Equilibria* 210(1):21–32.
67. Laesecke A, Bair S (2011) High Pressure Viscosity Measurements of 1,1,1,2-Tetrafluoroethane. *International Journal of Thermophysics* 32(5):925–941.
68. Meng X, Zhang J, Wu J (2011) Compressed Liquid Viscosity of 1,1,1,3,3-Pentafluoropropane (R245fa) and 1,1,1,3,3,3-Hexafluoropropane (R236fa). *Journal of Chemical & Engineering Data.* file://localhost/Arno/Data
69. Meng X, Qiu G, Wu J, Abdulagatov IM (2013) Viscosity measurements for 2,3,3,3-tetrafluoroprop-1-ene (R1234yf) and trans-1,3,3,3-tetrafluoropropene (R1234ze(E)). *The Journal of Chemical Thermodynamics* 63:24–30.
70. Zhao G, Bi S, Fröba AP, Wu J (2014) Liquid Viscosity and Surface Tension of R1234yf and R1234ze Under Saturation Conditions by Surface Light Scattering. *Journal of Chemical & Engineering Data* 59(4):1366–1371.
71. Diller DE, Peterson SM (1993) Measurements of the Viscosities of Saturated and Compressed Fluid 1-Chlor-1,2,2,2-Tetrafluoroethane (R124) and Pentafluoroethane (R125) at Temperatures Between 120 and 420 K. *Int. J. Thermophysics* 14(1):55–66.
72. Ripple D, Matar O (1993) Viscosity of the Saturated Liquid Phase of Six Halogenated Compounds and Three Mixtures. *Journal of Chemical and Engineering Data* 38:560–564.
73. Assael MJ, Papadopoulos AA, Polimatidou S (1995) Measurements of the Viscosity of Refrigerants in the Vapour Phase in *4th Asian Thermophysical Properties Conference.* (Tokyo, Japan), pp. 623–626.
74. Ripple D, Defibaugh D (1997) Viscosity of the Saturated Liquid Phase of Three Fluorinated Ethanes: R152a, R143a, and R125. *J. Chem. Eng. Data* 42:360–364.
75. Oliveira CMBP, Wakeham WA (1999) The Viscosity of R134a, R32, and R125 at Saturation. *International Journal of Thermophysics* 20(2):365–373.
76. Takahashi M, Shibasaki-Kitagawa N, Yokoyama C (1999) Viscosity of Gaseous HFC-125 (pentafluoroethane) Under High Pressures. *International Journal of Thermophysics* 20(2):445–453.
77. Fröba AP, Will S, Leipertz A (1999) Kinematic viscosity and surface tension of refrigerants from surface light scattering in *20th International Congress of Refrigeration.* (International Institute of Refrigeration, Sydney, Australia), p. preprint.
78. Bridgman PW (1926) The Effect of Pressure on the Viscosity of Fourty Three Pure Liquids. *Proceedings of the American Academy of Arts and Sciences* 61:57–99.
79. Mitsukuri S, Tonomura T (1927) Coefficient of viscosity for ethyl ether, acetone and methyl alcohol at low temperatures (in Japanese). *Journal of the Chemical Society of Japan* 48:334–340. Req. Mar. 16, 2006. Rec. Mar. 31, 2006.
80. Blokker PC (1936) Viscosity of methyl alcohol and acetone above their boiling points. *Receuil des Travaux Chimiques des Pays-Bas* 55:170–172. Ord. Feb. 24, 2004. Rec. Feb. 26, 2004.
81. Amis ES, Choppin AR, Padgitt FL (1942) Temperature and Composition Coefficients of the Density, Refractive Index, and Viscosity of the Methyl Alcohol-Dioxane System. *Journal of the American Chemical Society* 64:1207–1212. Ostwald -Sprengel pycnometer, Ostwald Cannon-Fenske viscometer.
82. Bridgman PW (1949) Viscosities to 30,000 kg/cm2. *Proceedings of the American Academy of Arts and Sciences* 77(4):115–128.
83. Golubev IF (1970) *Viscosity of gases and gas mixtures. A handbook.* (Jerusalem), p. 245.
84. Hammond LW, Howard KS, McAllister RA (1958) Viscosities and Densities of Methanol-Toluene Solutions up to their Normal Boiling Points. *Journal of Physical Chemistry* 62:637–639.
85. Ling TD, vanăWinkle M (1958) Properties of Binary Mixtures as a Function of Composition. *Industrial and Engineering Chemistry* 3(1):88–95.
86. Bamelis P, Nuyskens P, Meeussen m (1965) Influence de l'association des alcools sur la viscosité des solutions. *Journal de Chimie Physique et de Physico-Chimie Biologique* 62:158–170. pycnometer, Ostwald viscometer.
87. Isakova NP, Oshueva LA (1966) Viscosity of Liquid Methanol at High Pressures. *Russian Journal of Physical Chemistry* 40(5):607. One page only! Contains an abstract and a data table.
88. Harlow A (1967) Ph.D. thesis (University of London). Water.
89. Yergovich TW, Swift GW, Kurata F (1971) Density and viscosity of aqueous solutions of methanol and acetone from the freezing point to 10 řC. *Journal of Chemical and Engineering Data* 16(2):222–226.
90. Weber W (1975) Über die Druckabhängigkeit der Viskosität von Alkohol-Wasser-Gemischen. *Rheologica Acta* 14:1012–1025. Falling ball viscometer (Höppler).
91. Lee FM, Lahti LE, Stoops CE (1976) Solution Properties of Urea-Alcohol-Water Mixtures. *Journal of Chemical and Engineering Data* 21(1):36–40.
92. Schneider R (1978) Ph.D. thesis (Technische Universität Berlin).
93. Isdale JD, Easteal AJ, Woolf LA (1985) Shear viscosity of methanol and methanol + water mixtures under pressure. *International Journal of Thermophysics* 6(5):439–450.
94. Pikkarainen L (1988) Viscosities of binary solvent mixtures of N,N-diethylmethanesulfonamide with aliphatic alcohols. *Journal of Chemical and Engineering Data* 33(3):299–301.
95. Matsuo S, Makita T (1991) Viscosity of Methanol and 2-Methyl-2-Propanol. *International Journal of Thermophysics* 12(3):459–468.
96. Herbst CA, KingăJr. HE, Gao Z, Ou-Yang HD (1992) Dynamic light scattering measurements of high-pressure viscosity utilizing a diamond anvil cell. *Journal of Applied Physics* 72(3):838–844.

97. Aminabhavi TM, Aralaguppi MI, Harogoppad SB, Balundgi RH (1993) Densities, viscosities, refractive indices, and speeds of sound for methyl acetoacetate + aliphatic alcohols (C1-C8). *Journal of Chemical and Engineering Data* 38(1):31–39.
98. Cook RL, Herbst CA, KingăJr. HE (1993) High-Pressure Viscosity of Glass-Forming Liquids Measured by the Centrifugal Force Diamond Anvil Cell Viscometer. *Journal of Physical Chemistry* 97(10):2355–2361.
99. Assael M, Polimatidou SK (1994) Measurements of the Viscosity of Alcohols in the Temperature Range 290-340 K at Pressures up to 30 MPa. *International Journal of Thermophysics* 15(1):95–107.
100. Tu CH, Lee SL, Peng IH (2001) Excess Volumes and Viscosities of Binary Mixtures of Aliphatic Alcohols (C1-C4) with Nitromethane. *Journal of Chemical and Engineering Data* 46(1):151–155.
101. Abdulagatov I, Azizov N (2003) Viscosity for aqueous Li2SO4 solutions at temperatures from 298 to 575 K and at pressures up to 30 MPa. *J. Chem. Eng. Data* 48:1549–1556.
102. Abdulagatov I, Azizov N (2005) Viscosities of aqueous LiNO3 solutions at temperatures from 298 to 573 K and at pressures up to 30 MPa. *Ind. Eng. Chem. Res.* 44:416–425.
103. Abdulagatov I, Zeinalova A, Azizov N (2005) Viscosity of Aqueous Na2SO4 at Temperatures from 298 to 573 K and at Pressures up to 40 MPa. *Fluid Phase Equilib.* 227:57–70.
104. Agaev N, Yusibova A (1967) Experimental study of the viscosity of water at high pressures in the temperature range 0-100 řC (in Russian). *Teploenergetika 14(9), 75 (1967) [Thermal Eng. 14(9), 108 (1967)].*
105. Agayev NA (1980) Experimental Investigation of the Viscosity of Ordinary Water and Steam in the Temperature Range from -10 to 375řC and at Pressures from 0.1 to 200 MPa in *Proceedings of the 9th International Conference on the Properties of Steam*, eds. Straub J, Scheffler K. (Pergamon, Oxford), pp. 362–374.
106. Assael M, Polimatidou S (1994) Measurements of the Viscosity of Alcohols in the Temperature Range 290-340 K at Pressures up to 30 MPa. *Int. J. Thermophys.* 15:95–107.
107. Baldauf W, Knapp H (1983) Experimental Determination of Diffusion Coefficients, Viscosities, Densities and Refractive Indexes of 11 Binary Liquid Systems. *Berichte der Bunsengesellschaft für Physikalische Chemie* 87:304–309.
108. Berstad D, et al. (1988) Accurate Measurements of the Viscosity of Water in the Temperature Range 19.5-25.5 řC. *Physica A* 151:246–280.
109. Coe, J.R. J, Godfrey T (1944) Viscosity of Water. *J. Appl. Phys.* 15:625–626.
110. Collings A, Bejenov N (1983) A High Precision Capillary Viscometer and Further Relative Results for the Viscosity of Water. *Metrologia* 19:61–66.
111. DeFries T, Jonas J (1977) Pressure dependence of NMR proton spin-lattice relaxation times and shear viscosity in liquid water in the temperature range -15-10řC. *J. Chem. Phys.* 66(3):896–901.
112. Dudziak KH, Franck EU (1966) Messungen der Viskositat des Wassers bis 560 řC und 3500 bar. *Berichte der Bunsengesellschaft für Physikalische Chemie* 70:1120–1128.
113. Dumas D, Grjotheim K, Hogdahl P, Øye HA (1970) Theory of Oscillating Bodies and Its Utilization for Determination of High-Temperature Viscosities. *Acta Chem. Scand.* 24:510–530.
114. Eicher LD, Zwolinski BJ (1971) High-Precision Viscosity of Supercooled Water and Analysis of the Extended Range Temperature Coefficient. *J. Phys. Chem.* 75(13):2016–2024.
115. Först P, Werner F, Delgado A (2000) The Viscosity of Water at High Pressures - Especially at Subzero Degrees Centigrade. *Rheol. Acta* 39:566–573.
116. Gonçalves F (1980) The Viscosity of Water + Heavy Water Mixtures in the Range 20 - 60 řC in *Proceedings of the 9th International Conference on the Properties of Steam*, eds. Straub J, Scheffler K. (Pergamon, Oxford), pp. 354–361.
117. Hallett J (1963) The Temperature Dependence of the Viscosity of Supercooled Water. *Proceedings of the Physical Society* 82:1046–1050.
118. Hardy R, Cottington R (1949) Viscosity of Deuterium Oxide and Water in the Range 5 to 125 řC. *J. Res. Nat. Bur. Stand.* 42:573–578.
119. Harlow A (1967) *Further Investigations into the Effect of High Pressure on the Viscosity of Liquids.* (PhD Thesis, Department of Chemical Engineering and Chemical Technology, Imperial College of Science and Technology, London), p. 324.
120. Harris K, Woolf L (2004) Temperature and Volume Dependence of the Viscosity of Water and Heavy Water at Low Temperatures. *J. Chem. Eng. Data* 49:1064–1069.
121. Harris K, Woolf L (2004) Temperature and Volume Dependence of the Viscosity of Water and Heavy Water at Low Temperatures, erratum. *J. Chem. Eng. Data* 49(6):1851.
122. Horne R, Johnson D (1966) The viscosity of water under pressure. *J. Phys. Chem.* 70(7):2182–2190.
123. Isdale J, Spence C (1975) *A Self-centring Falling Body Viscometer for High Pressures, NEL Report No. 592.* (National Engineering Laboratory, East Kilbride, Glasgow), p. 20.
124. James CJ, Mulcahy DE, Steel BJ (1984) Viscometer Calibration Standards: Viscosities of Water Between 0 and 60řC and of Selected Aqueous Sucrose Solutions at 25řC From Measurements With a Flared Capillary Viscometer. *J. Phys. D: Appl. Phys.* 17:225–230.
125. Kerimov A, Agaev N, Abaszade A (1969) Experimental Study of the Viscosity of Water at Temperatures of 100-275 řC and at High Pressures (in Russian). *Teploenergetika 16(11), 87 (1969) [Thermal Eng. 16(11), 126 (1969)].*
126. Kestin J, Wang H (1960) The Viscosity of Superheated Steam up to 270 řC. *Physica* 26:575–584.

127. Kestin J, Richardson P (1963) The Viscosity of Superheated Steam up to 275 řC. A Refined Determination. *J. Heat Transfer* 85:295–302.
128. Kestin J, Khalifa H, Ro S, Wakeham W (1977) Preliminary Data on the Pressure Effect on the Viscosity of Sodium Chloride-Water Solutions in the Range 10-40 řC. *J. Chem. Eng. Data* 22:207–214.
129. Kestin J, Khalifa H, Sookiazian H, Wakeham W (1978) Experimental Investigatlon of the Effect of Pressure on the Viscosity of Water in the Temperature Range 10 - 150 řC. *Berichte der Bunsengesellschaft für Physikalische Chemie* 82:180–188.
130. Kestin J, Shankland I (1981) The Free Disk as an Absolute Viscometer and the Viscosity of Water in the Range 25-150 řC. *J. Non-Equilib. Thermodyn.* 6:241.
131. Kestin J, Imaishi N, Nott S, Sengers J (1985) Viscosity of Light and Heavy Water and their Mixtures. *Physica A* 134A:38–58.
132. Kingham D, Adams W, McGuire M (1974) Viscosity Measurements of Water in Region of Its Maximum Density. *J. Chem. Eng. Data* 19:1–3.
133. Korosi A, Fabuss B (1968) Viscosity of Liquid Water from 25 to 150 řC. Measurements in Pressurised Glass Capillary Viscometer. *Anal. Chem.* 40:157–162.
134. Korson L, Drost-Hansen W, Millero F (1969) Viscosity of Water at Various Temperatures. *J. Phys. Chem.* 73:34–39.
135. Kozlov G (1985) Determination of the Viscosity of Water by a Pulse NMR Method (in Russian). *Kolloidnyi Zhurnal 47(6), 1184 (1985) [Colloid Chem. 47(6), 1018 (1986)].*
136. Kubota H, et al. (1979) Specific Volume and Viscosity of Methanol-Water Mixtures Under High Pressure. *The Review of Physical Chemistry of Japan* 49(2):59–69.
137. Kudish A, Wolf D, Steckel F (1974) Physical Properties of Oxygen-17 Water. Absolute Viscosity and Density of Oxygen-17 Water Between 15 and 35 řC. *Journal of the Chemical Society, Faraday Transactions 1* 70:484–489.
138. Latto B (1965) Viscosity of Steam at Atmospheric Pressure. *Int. J. Heat Mass Transfer* 8:689–720.
139. Lee M, Wei M (1992) Densities and Viscosities of 2-Butanone/Dibutyl Ether, 2-Picoline/2-Butanone, and 2-Picoline/Water Mixtures. *J. Chem. Eng. Data* 37:209–212.
140. Lee M, Lin TK (1995) Density and Viscosity for Monoethanolamine + Water, + Ethanol, and + 2-Propanol. *J. Chem. Eng. Data* 40:336–339.
141. Malyarov G (1959) (in Russian). *Trudi VNIIM* 37:125–140.
142. Mashovets V, Puchkov L, Sargaev P, Fedorov M (1971) Apparatus for Measuring the Viscosities of Electrolyte Solutions at Temperatures up to 275 řC (in Russian). *Zh. Prikl. Khim. 44(1), 90 (1971) [J. App. Chem. USSR, 44(1), 85 (1971)].*
143. Mayinger F (1962) Messungen der Viskositat von Wasser und Wasserdampf bis zu 700 řC und 800 AT. *Int. J. Heat Mass Transfer* 5:807–824.
144. Mazurkiewicz J, Tomasik P (1990) Viscosity and Dielectric Properties of Liquid Binary Mixtures. *J. Phys. Org. Chem.* 3:493–502.
145. Melzer W, Baldauf W, Knapp H (1989) Measurement of Diffusivity, Viscosity, Density and Refractivity of Eight Binary Liquid Mixtures. *Chem. Eng. Prog.* 26:71–79.
146. Moszynski J (1961) The Viscosity of Steam and water at Moderate Pressures and Temperatures. *Transactions of the ASME* 83:111–123.
147. Naake LD (1984) *Die Viskosität von n-Dekan und Methan-Dekan-Mischungen bis 300 řC und 3000 bar.* (PhD Thesis, University of Karlsruhe).
148. Nagashima A, Tanishita I (1969) Viscosity Measurement of Water and Steam at High Temperatures and High Pressures. *Bulletin of the Japanese Society of Mechanical Engineers* 12(54):1467–1478.
149. Nagashima A, Tanishita I, Murai Y (1974) Measurement of Pressure Effect on Viscosity of Steam. *J. Chem. Eng. Data* 19(3):212–213.
150. Olivé F, Patil K, Coronas A, Fernández F (1994) Densities, Viscosities, and Excess Properties of Trifluoroethanol-Water,Ttetraethylene Glycol Dimethylether-Water, and Trifluoroethanol-Tetraethylene Glycol Dimethylether at 303.15 K. *Int. J. Thermophys.* 15:661–674.
151. Oltermann G (1977) *Measurement of the Viscosity of Steam near the Critical Point.* (PhD Thesis, Technische Universität Hannover), p. 78.
152. Penkina N, Matsonashvili BY (1971) Radiolsotope Viscometer for Measurements over Wide Ranges of Temperatures and Pressures (in Russian). *Zh. Prikl. Khim. 44(2), 447 (1971) [J. App. Chem. USSR, 44(2), 448 (1971)].*
153. Ramkumar D, Kudchadker A (1989) Mixture Properties of the Water + g-butyrolactone + Tetrahydrofuran System. 2. Viscosities and Surface Tensions of g-Butyrolactone + Water a 303.15-343.15 K and g-Butyrolactone + Tetrahydrofuran at 278.15-298.15 K. *J. Chem. Eng. Data* 34:463–465.
154. Ravikovich C, Solomko V (1958) Study of the viscosity and critical tempertures of some deuterated compounds and their mixtures (in Russian). *Ukr. Khim. Zh. (Russ. Ed.)* 24:7–12.
155. Rivkin S, Levin AY (1966) Experimental Study of the Viscosity of Water and Steam. *Teploenergetika 13(4), 79 (1966) [Thermal Eng. 13(4), 104 (1966)].*
156. Rivkin S, Levin AY, Izrailevskii L (1968) (in Russian). *Teploenergetika 15(12), 74 (1968) [Thermal Eng. 15(12), 108 (1968)].*
157. Rivkin S, Levin AY, Izrailevskii L (1970) Study of the Coefficient of Dynamic Viscosity of Steam Close to the Saturation

Line (in Russian). *Teploenergetika 17(8), 88 (1970) [Thermal Eng. 17(8), 127 (1970)].*
158. Rivkin S, Levin AY, Izrailevskii L (1972) Dynamic Viscosity Coefficient of Water and Water Vapour (in Russian). *Teplo i Massoperenos* 7:61–71.
159. Rivkin S, Levin AY, Izrailevskii L, Kharitonov K (1973) An Experimental Investigation of the Viscosity of Water in the Supercritical Region of Parameters of State at Pressures up to 500 bar and Temperatures up to 500 řC. *Teploenergetika 20(8), 11 (1973) [Thermal Eng. 20(8), 14 (1973)].*
160. Rivkin S, Levin AY, Izrailevskii L, Kharitonov K (1975) Experimental Investigation of Viscosity of Light Water Near the Critical Point and of Heavy Water in Liquid Phase and in Supercritical Region in *Proceedings 8th International Conference on Properties of Steam*, eds. Bury P, Perdon H, Vodar B. pp. 153–166.
161. Roscoe R, Bainbridge W (1958) Viscosity Determination by the Oscillating Vessel Method. II: The Viscosity of Water at 20 řC. *Proceedings of the Physical Society* 72:585–595.
162. Rosenberger F, Iwan J, Alexander D, Jin W (1992) Gravimetric Capillary Method for Kinematic Viscosity Measurements. *Rev. Sci. Instrum.* 63:4196–4199.
163. Sato K, Minamiyama T, Yata J, Oka T (1968) Measurement of Viscosity of Steam at Moderate Temperatures and Pressures, Paper B-5 in *7th International Conference on the Properties of Steam.* (ASME, New York).
164. Sato K, Minamiyama T, Yata J, Oka T, Suzuki M (1970) A Study of Viscosity for Steam at Moderate Pressures in *Proceedings 45th Annual Meeting, Kansai Div. Jap. Soc. Mech. Eng.* Vol. 704, pp. 7–9.
165. Shifrin A (1959) (in Russian). *Teploenergetika 6(9), 22.*
166. Stanley E, Batten R (1969) Viscosity of water at high pressures and moderate temperatures. *J. Phys. Chem.* 73(5):1187–1191.
167. Swindells J, Coe, J.R. J, Godfrey T (1952) Absolute Viscosity of Water at 20 řC. *J. Res. Nat. Bur. Stand.* 48:1–31.
168. Tanaka K, et al. (1965) (in Japanese). *Transactions of the Japan Society of Mechanical Engineers* 31:1847–1859.
169. Tanaka K, Matsuda H, Fujiwara H, Kubota H, Makita T (1987) Viscosity of (Water + Alcohol) Mixtures Under High Pressure. *Int. J. Thermophys.* 8:147–163.
170. Teske V, Vogel E, Bich E (2005) Viscosity Measurements on Water Vapor and their Evaluation. *J. Chem. Eng. Data* 50:2082–2087.
171. Timrot D, Serednitskaya M, Bespalov M (1973) Experimental Investigation of Steam Viscosity at Temperatures from 50 to 500 řC and Pressures from 0.06 to 1.5 bar (in Russian). *Teploenergetika 20(8), 78 (1973) [Thermal Eng. 20(8), 106 (1973)].*
172. Weber W (1955) Die Temperaturabhangigkeit der Viskositat des Wassers zwischen 0 und 40 řC. *Zeitschrift für Angewandte Physik* 7:96–98.
173. White G, Twining R (1914) The Viscosity of Undercooled Water as Measured in a New Viscosimeter. *J. Am. Chem. Soc.* 50:380–389.
174. Whitelaw J (1960) Viscosity of Steam at Supercritical Pressures. *Journal of Mechanical Engineering Science* 2:288–294.
175. Wode H, Seidel W (1994) Precise Viscosity Measurements of Binary Liquid Mixtures of Acetonitrile-Water and 1,3-Dimethyl-2-Imidazolidinone-Water. *Berichte der Bunsengesellschaft für Physikalische Chemie* 98:927–934.
176. Yasumoto I (1970) Viscosity of Water Vapor ln the Temperature Range from 6 to 29 řC. *Bull. Chem. Soc. Jpn.* 43:3917–3919.
177. Carnahan NF, Starling KE (1969) Equation of State for Nonattracting Rigid Spheres. *J. Chem. Phys.* 51(2):635–636.
178. Barlow NS, Schultz AJ, Weinstein SJ, Kofke DA (2012) An asymptotically consistent approximant method with application to soft- and hard-sphere fluids. *J. Chem. Phys.* 137(20):204102.
179. Sigurgeirsson H, Heyes DM (2003) Transport coefficients of hard sphere fluids. *Mol. Phys.* 101(3):469–482.
180. Dymond J (1976) A Modified Hard-Sphere Theory for Transport Properties of Fluids Over the Whole Density Range. *Chem. Phys.* 17:101–109.
181. Chapman S, Cowling TG (1970) *The Mathematical Theory of Non-uniform Gases: An Account of the Kinetic Theory of Viscosity, Thermal Conduction and Diffusion in Gases.* (Cambridge University Press).
182. Fomin YD, Brazhkin VV, Ryzhov VN (2012) Transport coefficients of soft sphere fluid at high densities. *JETP Letters* 95(6):320–325.
183. Tan TB, Schultz AJ, Kofke DA (2011) Virial coefficients, equation of state, and solid–fluid coexistence for the soft sphere model. *Mol. Phys.* 109(1):123–132.
184. Heyes DM, Okumura H (2006) Equation of state and structural properties of the Weeks-Chandler-Andersen fluid. *J. Chem. Phys.* 124(16):164507.
185. Elliot JR, Daubert TE (1986) The temperature dependence of the hard sphere diameter. *Fluid Phase Equilib.* 31(2):153–160.
186. Ghobadi AF, Elliott JR (2013) Adapting SAFT–perturbation theory to site-based molecular dynamics simulation. I. Homogeneous fluids. *J. Chem. Phys.* 139(23):234104.
187. Ahmed A, Sadus RJ (2009) Phase diagram of the Weeks-Chandler-Andersen potential from very low to high temperatures and pressures. *Phys. Rev. E* 80(6):061101.
188. Chandler D, Weeks JD, Andersen HC (1983) Van der Waals Picture of Liquids, Solids, and Phase Transformations. *Science* 220(4599):787–794.
189. Allen MP, Tildesley DJ (1987) *Computer Simulations of Liquids.* (Oxford University Press, New York).

190. Tenney CM, Maginn EJ (2010) Limitations and recommendations for the calculation of shear viscosity using reverse nonequilibrium molecular dynamics. *J. Chem. Phys.* 132(1):014103–8.
191. Daivis PJ, Evans DJ (1994) Comparison of constant pressure and constant volume nonequilibrium simulations of sheared model decane. *J. Chem. Phys.* 100(1):541–547.
192. Baidakov VG, Protsenko SP, Kozlova ZR (2012) Metastable Lennard-Jones fluids. I. Shear viscosity. *J. Chem. Phys.* 137(16):164507.
193. Galliéro G, Boned C, Baylaucq A (2005) Molecular Dynamics Study of the Lennard-Jones Fluid Viscosity: Application to Real Fluids. *Ind. Eng. Chem. Res.* 44(17):6963–6972.
194. Heyes DM (1988) Transport coefficients of Lennard-Jones fluids: A molecular-dynamics and effective-hard-sphere treatment. *Phys. Rev. B* 37(10):5677–5696.
195. Meier K, Laesecke A, Kabelac S (2004) Transport coefficients of the Lennard-Jones model fluid. I. Viscosity. *J. Chem. Phys.* 121:3671.
196. Michels J, Trappeniers N (1985) Molecular dynamical calculations of the viscosity of Lennard-Jones systems. *Physica A* 133(1-2):281–290.
197. Oderji HY, Ding H, Behnejad H (2011) Calculation of the second self-diffusion and viscosity virial coefficients of Lennard-Jones fluid by equilibrium molecular dynamics simulations. *Phys. Rev. E* 83(6).
198. Vasquez VR, Macedo EA, Zabaloy MS (2004) Lennard-Jones Viscosities in Wide Ranges of Temperature and Density: Fast Calculations Using a Steady–State Periodic Perturbation Method. *Int. J. Thermophys.* 25(6):1799–1818.
199. Bell IH, Bouck L, Alpert BK (2018) ChebTools: C++11 (and Python) tools for working with Chebyshev expansions. *Journal of Open Source Software*.
200. Ashurst WT, Hoover WG (1975) Dense-fluid shear viscosity via nonequilibrium molecular dynamics. *Phys. Rev. A* 11(2):658–678.
201. Rosenfeld Y (1977) Relation between the transport coefficients and the internal entropy of simple systems. *Phys. Rev. A* 15(6):2545–2549.
202. Rosenfeld Y (1999) A quasi-universal scaling law for atomic transport in simple fluids. *J. Phys.: Condens. Matter* 11(28):5415–5427.
203. Noro MG, Frenkel D (2000) Extended corresponding-states behavior for particles with variable range attractions. *J. Chem. Phys.* 113(8):2941–2944.
